# Supplementary material for: Progress Report on Numerical Modeling of a Prototype Fuel Cell
Source: arXiv:2002.04519 ancillary file (2020-11-13)
Supplement: Supplementary file 1 [file sm_pt1.pdf]

# Progress Report on Numerical Modeling of a Prototype Fuel Cell:

## 1. Comparison between Mathematical Formulations

### Supplemental Material

Otávio Beruski,<sup>1,\*</sup> Ivan Korkischko,<sup>1,†</sup> Thiago Lopes,<sup>1,‡</sup> and Fabio Coral Fonseca<sup>1,§</sup>

<sup>1</sup>*Instituto de Pesquisas Energéticas e Nucleares,  
IPEN/CNEN-SP, 05508-000, São Paulo, São Paulo, Brazil*

#### SI. INTRODUCTION

This document provides the supplementary information for some decisions, results and discussions made that were deemed secondary to the article. For proper context and discussions, we refer the reader to the paper. The following is presented here. Section SII presents the different species transport formulations and the results supporting the rationale of using an effective  $O_3$ /“air” mixture for the full model. Section SIII compares different couplings between molecular diffusion, porous media correction and Knudsen diffusion, as well as the effect of including each one and combinations of them. Section SIV provides additional information on the comparison between the original Alpha model and the improved Beta model: figures for variables related to the flow field, a brief comparison between Stokes-Darcy (SD) and Darcy-Brinkman (DB) flow field formulations, and figures containing error estimates for the scalar response variables, obtained from the grid convergence study. Finally, Section SV provides additional information on the parametric study of reaction rate constants, exploring the range of values more thoroughly.

---

\* oberuski@alumni.usp.br

† ivan.korkischko@gmail.com

‡ tlopeschem@gmail.com

§ fabiocf@usp.br

## SII. COMPARISON BETWEEN MIXTURES

As mentioned in Section II.A.2 of the paper, the improved model uses a simplified formulation for the fluid’s species. As reported in [1], the experimental device used O<sub>3</sub>-enriched air as working fluid, and thus a first approach would be to model its species as a O<sub>3</sub>/O<sub>2</sub>/N<sub>2</sub> fluid. However it is known that only the O<sub>3</sub> is reactive in the experimental conditions used, and that  $\chi_{\text{O}_3} \sim 10^{-3}$  at the inlet,  $\chi_i$  being the species’ molar fraction. Thus one might consider that  $\chi_{\text{O}_2}$  and  $\chi_{\text{N}_2}$  are approximately constant. Indeed, this is the same rationale behind the diluted species approach used previously[2]. This has two implications, namely i) the fluid’s properties, i.e. viscosity and density, are largely due to O<sub>2</sub> and N<sub>2</sub>, and thus very much like air; and ii) the chemical driving forces acting on O<sub>3</sub> are mainly given by  $\nabla\chi_{\text{O}_3}$  in a bath of air. Therefore, another option would be to model the fluid using effective “air” molecules along with O<sub>3</sub>. In this way, one saves computational resources while at the same time reducing the hardships of measuring, or calculating, the binary diffusion coefficients for each pair of species in the fluid at varied concentrations.

In order to verify these assumptions, numerical simulations were carried using the improved mathematical framework, detailed in Section II.A.2 of the paper, with the reduced geometry shown in Section II.B.1 of Part II. Two formulations were thus compared for the species transport: O<sub>3</sub>/air and O<sub>3</sub>/O<sub>2</sub>/N<sub>2</sub>. Density was given using the ideal gas law, with the molar mass of “air” molecules given in Table III of the paper ( $M_{\text{air}}$ ), while viscosity was given by a constitutive equation provided by the software, function only of the temperature, and thus the same for both mixtures. The binary diffusion coefficients had to be simplified, with the O<sub>3</sub>/air mixture following the paper, i.e. using the diffusion coefficient of O<sub>3</sub> in air,  $D_{\text{O}_3}$ , of Table II; while for the O<sub>3</sub>/O<sub>2</sub>/N<sub>2</sub> mixture  $D_{\text{O}_3}$  was used for the O<sub>3</sub> – O<sub>2</sub> and O<sub>3</sub> – N<sub>2</sub> pairs, and a 1:1 molar ratio binary diffusion coefficient for O<sub>2</sub> – N<sub>2</sub>:

$$D_{\text{O}_2-\text{N}_2} = 5.6771 \times 10^{-9} T^{3/2} \exp\left(-\frac{107.2}{T}\right) \quad (1)$$

with  $D$  in m<sup>2</sup> s<sup>-1</sup> and  $T$  in K. The above relation for  $D_{\text{O}_2-\text{N}_2}$  was obtained from non-linear regression of temperature-dependent experimental data compiled in [3, 4]. Likewise, the Knudsen diffusivities were the same for the O<sub>3</sub> – air, O<sub>3</sub> – O<sub>2</sub>, and O<sub>3</sub> – N<sub>2</sub> pairs, obtained using Eq. 10 of the paper for O<sub>3</sub>. The Knudsen diffusivity for the O<sub>2</sub> – N<sub>2</sub> pair, on the other hand, was given by an inverse sum of each coefficient, weighed by their respective

molar fractions:

$$D_{\text{O}_2-\text{N}_2}^K = \left( \frac{\chi_{\text{O}_2}}{D_{\text{O}_2}^K} + \frac{\chi_{\text{N}_2}}{D_{\text{N}_2}^K} \right)^{-1} \quad (2)$$

where each  $D_i^K$  was also calculated using Eq. 10 of the paper. The mesh and solver schemes used follow the brief description given the paper, however with  $\lambda = 16$ , with additional details in Part II and respective Supplemental Material (SM).

Below are presented the relevant results within the context of the paper and the proposed comparison, viz., the scalar response variables, the profiles, and surfaces. Section II.B.2 of the paper details the acquisition of each response variable. Figure S1 shows the scalar variables for both mixtures, while Figure S2 presents the  $\bar{R}_{\text{O}_3}$  and  $P_{\text{O}_3}$  profiles for  $Q = 250$  and  $450 \text{ cm}^3 \text{ min}^{-1}$ . And Figure S3 shows the  $\mathbf{P}_{\text{O}_3}$  surfaces, also for  $Q = 250$  and  $450 \text{ cm}^3 \text{ min}^{-1}$ , and the difference between the two mixtures.

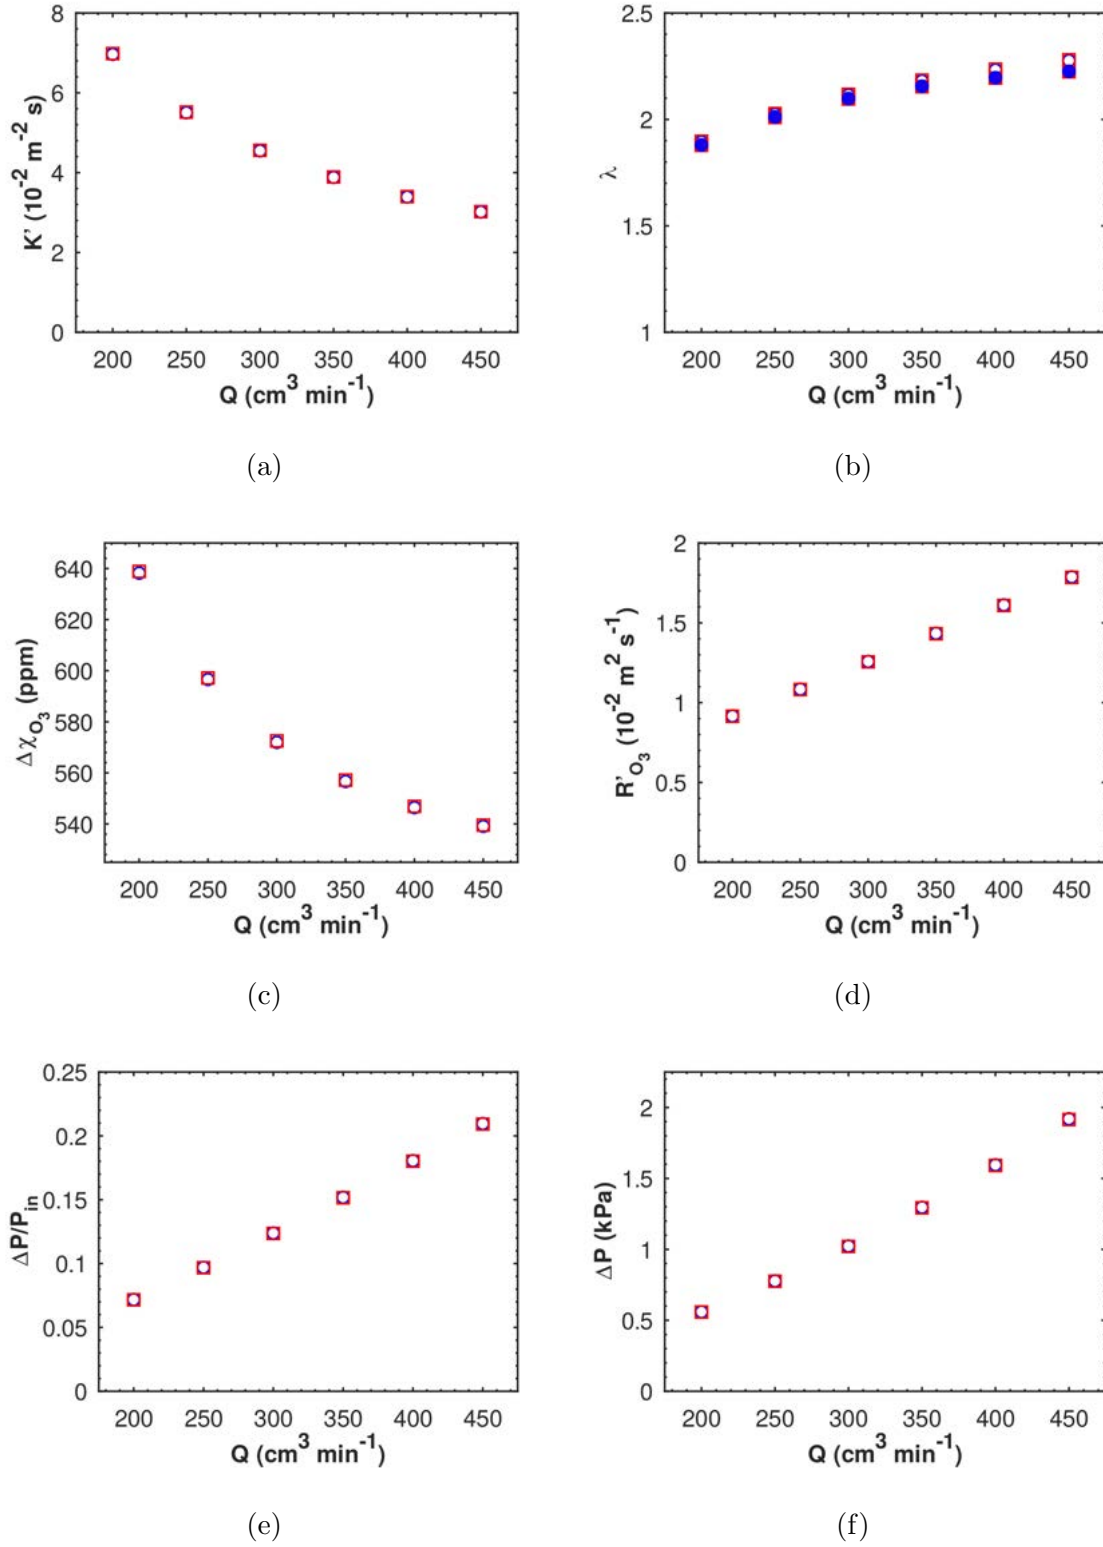

FIG. S1: Scalar response variables as function of inlet flow rate  $Q$  for both  $\text{O}_3/\text{air}$  ( $\circ$ ) and  $\text{O}_3/\text{O}_2/\text{N}_2$  ( $\square$ ) mixtures: (a)  $K' = \Delta\chi_{\text{O}_3}/R'_{\text{O}_3}$ , (b)  $\lambda$  (empty symbols) and  $\lambda'$  (full symbols), (c)  $\Delta\chi_{\text{O}_3}$ , (d)  $R'_{\text{O}_3}$ , (e)  $\Delta P/P_{\text{in}}$ , and (f)  $\Delta P$ .

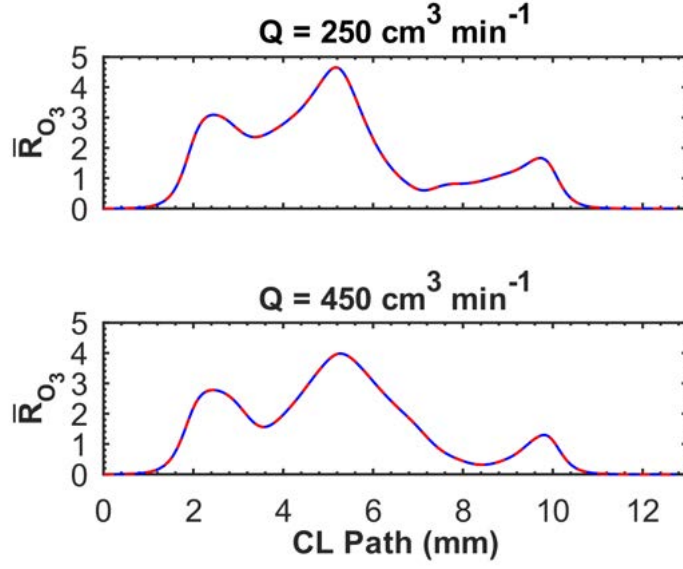

(a)

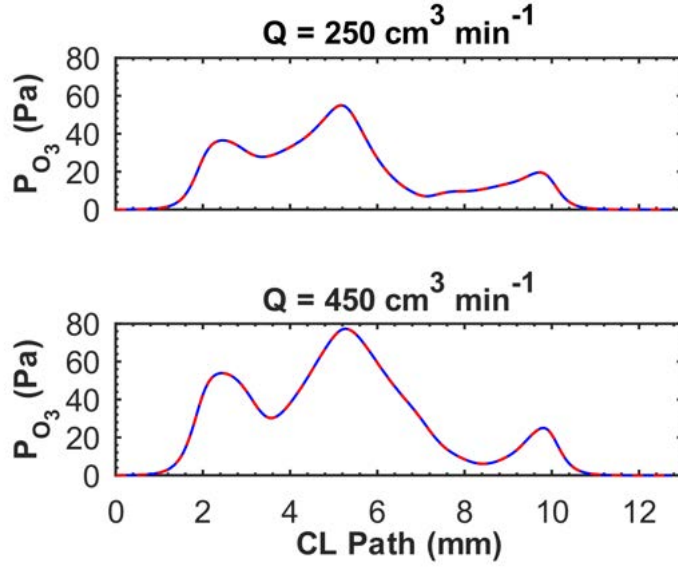

(b)

FIG. S2: **(a)** Normalized reaction rate and **(b)** ozone partial pressure profiles as function of the path along the CL upper boundary, for inlet flow rates  $Q = 250$  (top) and  $450 \text{ cm}^3 \text{ min}^{-1}$  (bottom). Both mixtures are shown,  $O_3/\text{air}$  (full line) and  $O_3/O_2/N_2$  (dashed line).

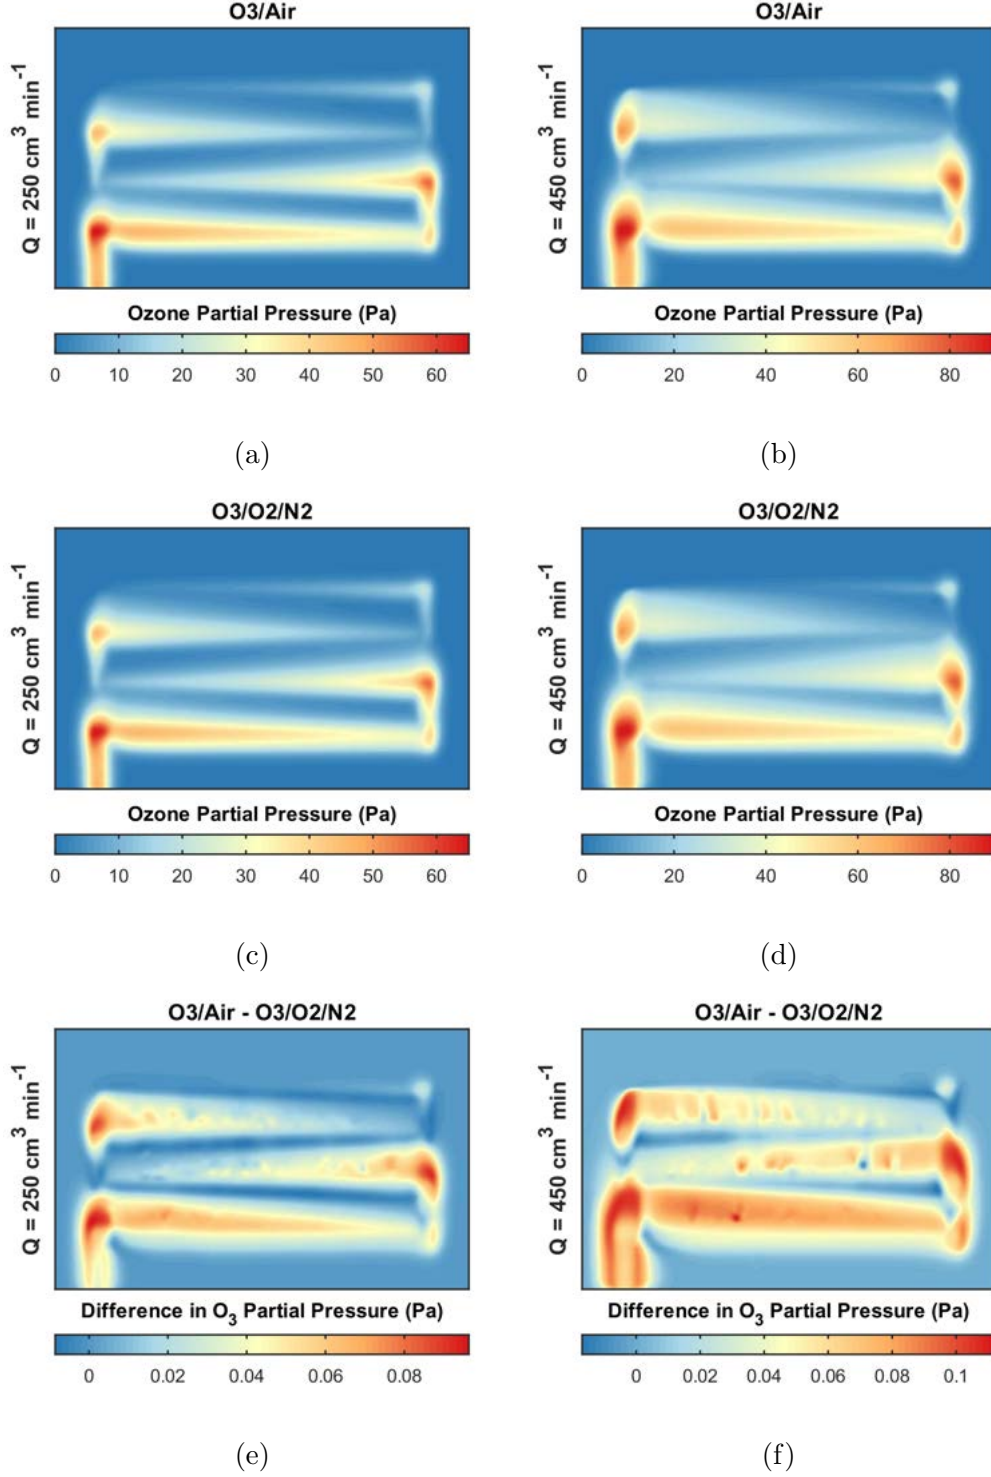

FIG. S3: Ozone partial pressure surfaces obtained at the upper boundary of the CL domain, for inlet flow rates  $Q = 250$  (left column) and  $450 \text{ cm}^3 \text{ min}^{-1}$  (right column):  $\text{O}_3/\text{air}$  mixture (top row),  $\text{O}_3/\text{O}_2/\text{N}_2$  mixture (middle row), and difference between them (bottom row).

### **III. COUPLING BETWEEN FREE, POROUS MEDIA, AND KNUDSEN DIFFUSION**

It was pointed out in Section II.A.2 of the paper that the coupling between different modes of diffusion was not entirely clear at this point. By that it is meant the mathematical relation that expresses the effective diffusion coefficient that would be measured in a macroscopic device,  $D_i$ . In the paper it was chosen to apply a correction to the free diffusion,  $D_i^{\text{free}}$ , due to the porous media:

$$D_i^{\text{Pm}} = f_{\text{eff}} D_i^{\text{free}} \quad (3)$$

where  $f_{\text{eff}} = f_{\text{eff}}(\epsilon, \tau)$ , with  $\epsilon$  and  $\tau$  being the porosity and tortuosity of the porous medium, respectively. This was then coupled to Knudsen diffusivity, in an inverse sum shown in Eq. 9 of the paper. Such scheme will be represented as MS \* Pm + K, i.e. porous media correction applied to Maxwell-Stefan diffusivity plus Knudsen diffusivity. It should be once again noticed, however, that  $D_i$  is an entry of the MS diffusion matrix, and thus this is only an accurate representation of the actual diffusivity for a binary mixture, as in the case of O<sub>3</sub>/air, and even then only in the case of constant composition. While COMSOL Multiphysics<sup>®</sup> allows modification of the model's equations, for instance allowing the coupling to Knudsen diffusivity after calculation of the multi-component Fick diffusivities, this was not attempted. Given this present limitation, the MS \* Pm + K scheme was compared with four other schemes: ii) Pm \* (MS + K), iii) MS + K, iv) MS \* Pm, and v) MS. This allows one to estimate the contribution of each effect, namely the coupling to porous media and Knudsen diffusion, and the possible effect different coupling would have on the model.

Numerical calculation were then carried using the improved mathematical framework, detailed in Section II.A.2 of the paper, with the reduced geometry shown in Section II.B.1. The simplified O<sub>3</sub>/air mixture was used, and the five different diffusion schemes were applied to the  $D_{\text{O}_3\text{-air}} \approx D_{\text{O}_3}$  entry to the MS diffusion matrix. For the sake of completeness, the different schemes are defined in the following way:

1. MS \* Pm + K:  $D_i = \left[ \frac{1}{f_{\text{Pm}} D_i^{\text{free}}} + \frac{1}{D_i^K} \right]^{-1}$
2. Pm \* (MS + K):  $D_i = f_{\text{Pm}} \left[ \frac{1}{D_i^{\text{free}}} + \frac{1}{D_i^K} \right]^{-1}$
3. MS + K:  $D_i = \left[ \frac{1}{D_i^{\text{free}}} + \frac{1}{D_i^K} \right]^{-1}$

4. MS \* Pm:  $D_i = f_{\text{Pm}} D_i^{\text{free}}$

5. MS:  $D_i = D_i^{\text{free}}$

The remainder of the mathematical framework is the same for each scheme. The mesh and solver schemes used are the same used in Section SII. Additional details may be found in Part II and respective SM.

Below are presented the relevant results within the context of the paper and the proposed comparison, viz., the scalar response variables, the profiles, and surfaces. Section II.B.2 of the paper details the acquisition of each response variable. Figure S4 shows the scalar variables for all schemes, while Figure S5 presents the  $\bar{R}_{\text{O}_3}$  and  $P_{\text{O}_3}$  profiles at  $Q = 250$  and  $450 \text{ cm}^3 \text{ min}^{-1}$ . Figures S6 and S7 shows the  $\mathbf{P}_{\text{O}_3}$  surfaces, for  $Q = 250$  and  $450 \text{ cm}^3 \text{ min}^{-1}$  respectively, while Figures S8 and S9 shows the differences between the scheme used in the paper, MS \* Pm + K, and each of the remaining schemes, for  $Q = 250$  and  $450 \text{ cm}^3 \text{ min}^{-1}$  respectively.

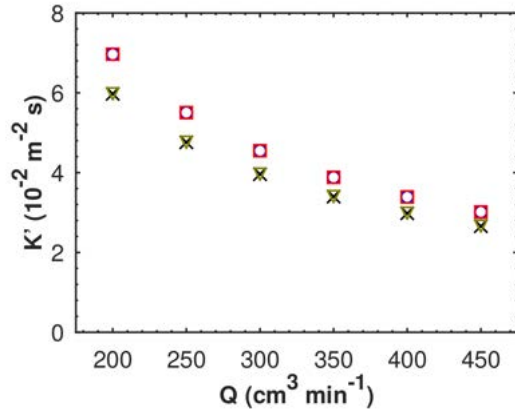

(a)

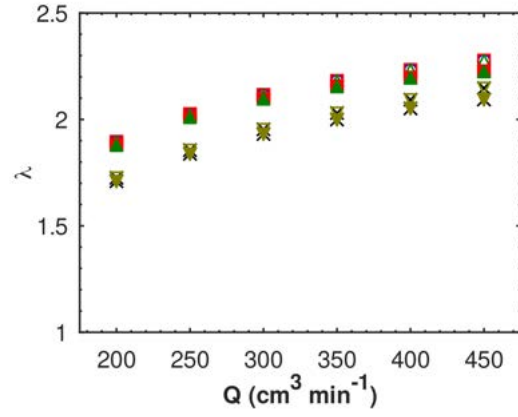

(b)

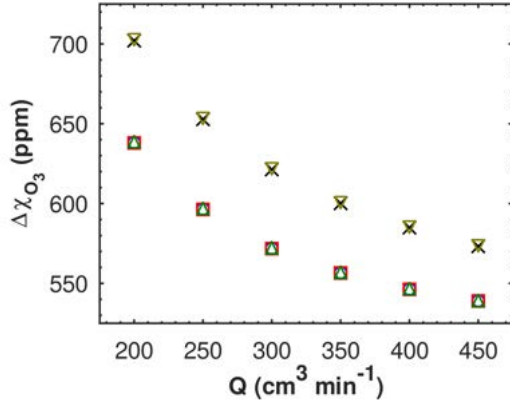

(c)

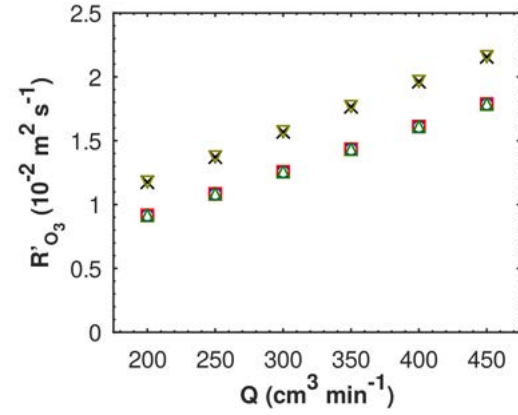

(d)

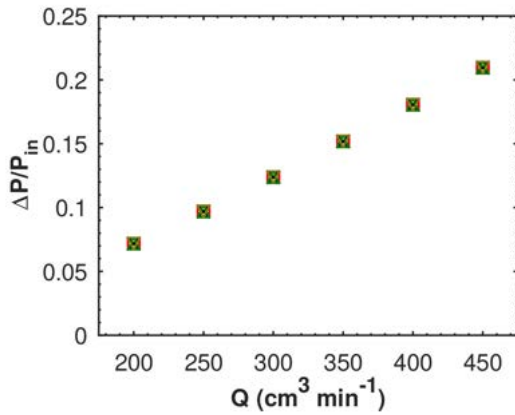

(e)

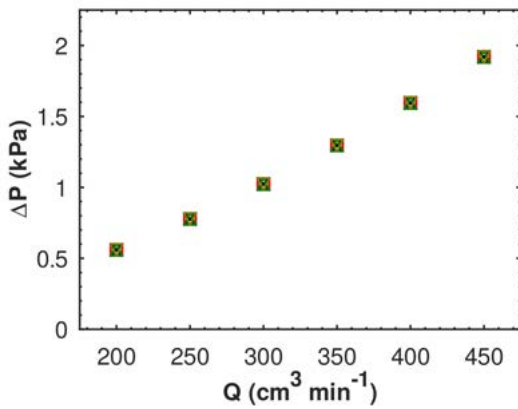

(f)

FIG. S4: Scalar variables as function of inlet flow rate  $Q$  for different coupling schemes: MS \* Pm + K (○), Pm \* (MS + K) (□), MS + K (×), MS \* Pm (△), and MS (▽). (a)  $K' = \Delta\chi_{O_3}/R'_{O_3}$ , (b)  $\lambda$  (empty symbols) and  $\lambda'$  (full symbols), (c)  $\Delta\chi_{O_3}$ , (d)  $R'_{O_3}$ , (e)  $\Delta P/P_{in}$ , and (f)  $\Delta P$ .

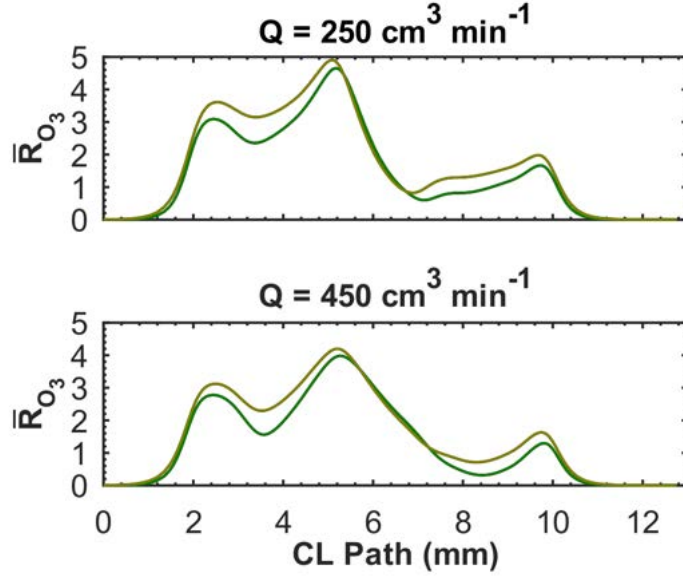

(a)

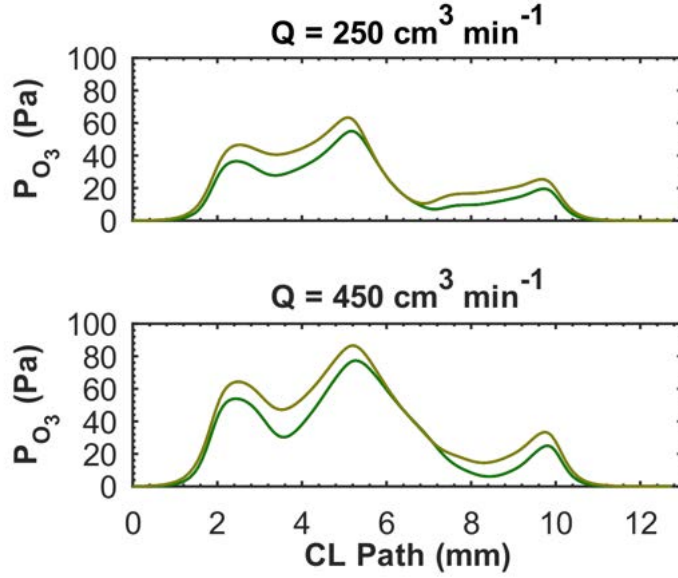

(b)

FIG. S5: **(a)** Normalized reaction rate and **(b)** ozone partial pressure profiles as function of the path along the CL upper boundary, for inlet flow rates  $Q = 250$  (top) and  $450 \text{ cm}^3 \text{ min}^{-1}$  (bottom). The following coupling schemes are shown:  $MS * Pm + K$ ,  $Pm * (MS + K)$ ,  $MS + K$ ,  $MS * Pm$ , and  $MS$ .  $MS + K$  and  $MS$  show larger values and are superimposed. The remaining show lower values and are also superimposed.

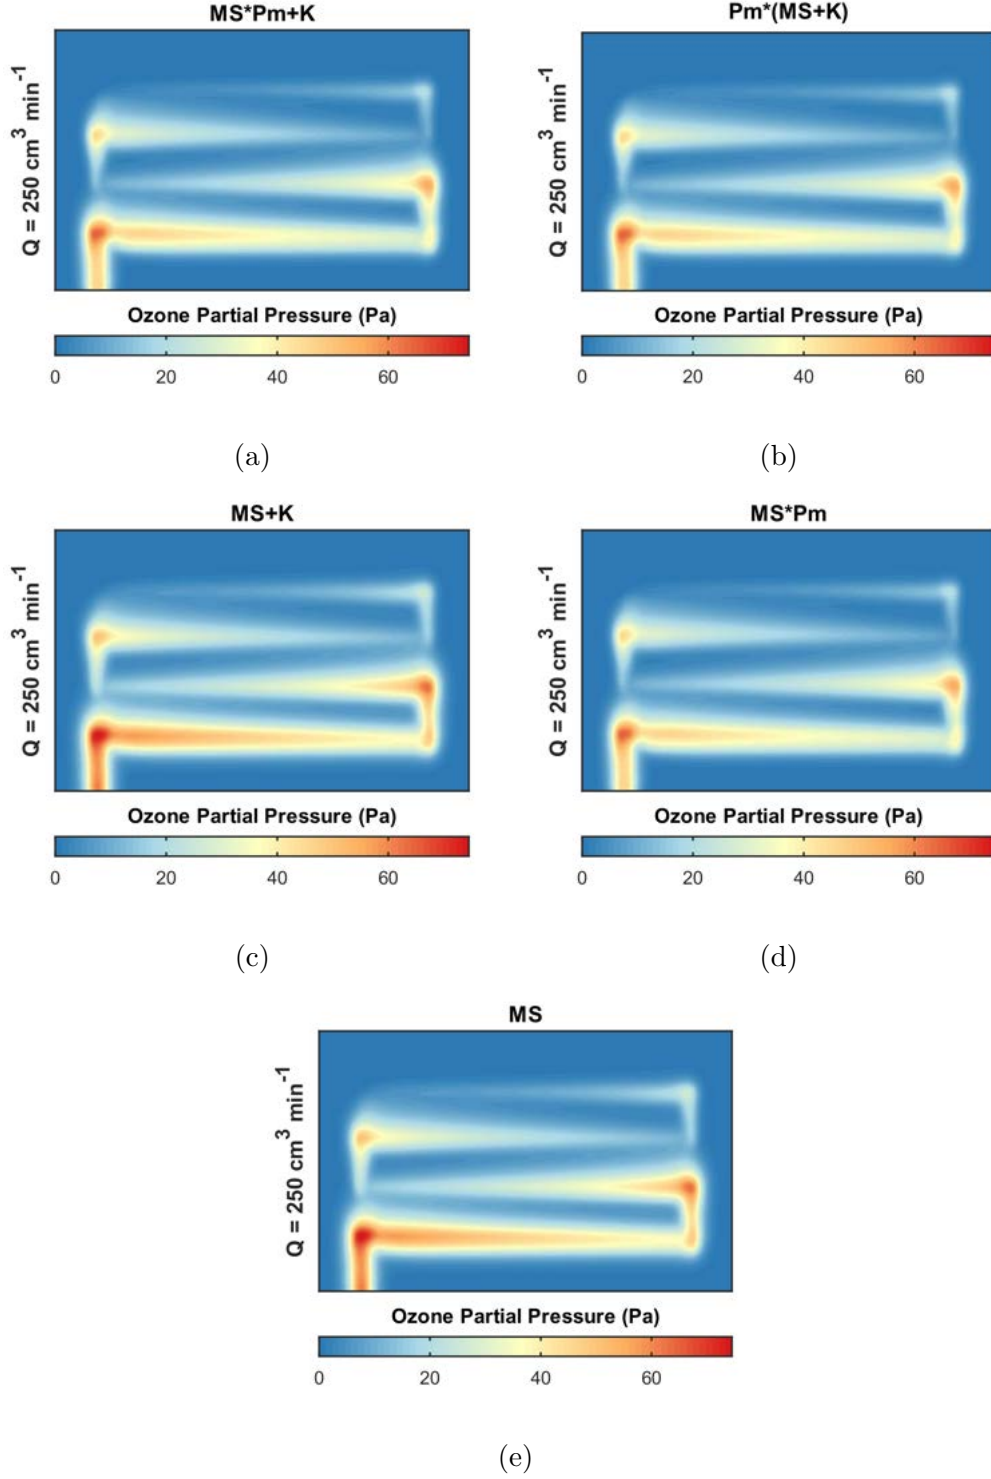

FIG. S6: Ozone partial pressure surfaces obtained at the upper boundary of the CL domain, for inlet flow rate  $Q = 250 \text{ cm}^3 \text{ min}^{-1}$ , using the follow coupling schemes: (a)  $MS * Pm + K$ , (b)  $Pm * (MS + K)$ , (c)  $MS + K$ , (d)  $MS * Pm$ , and (e)  $MS$ .

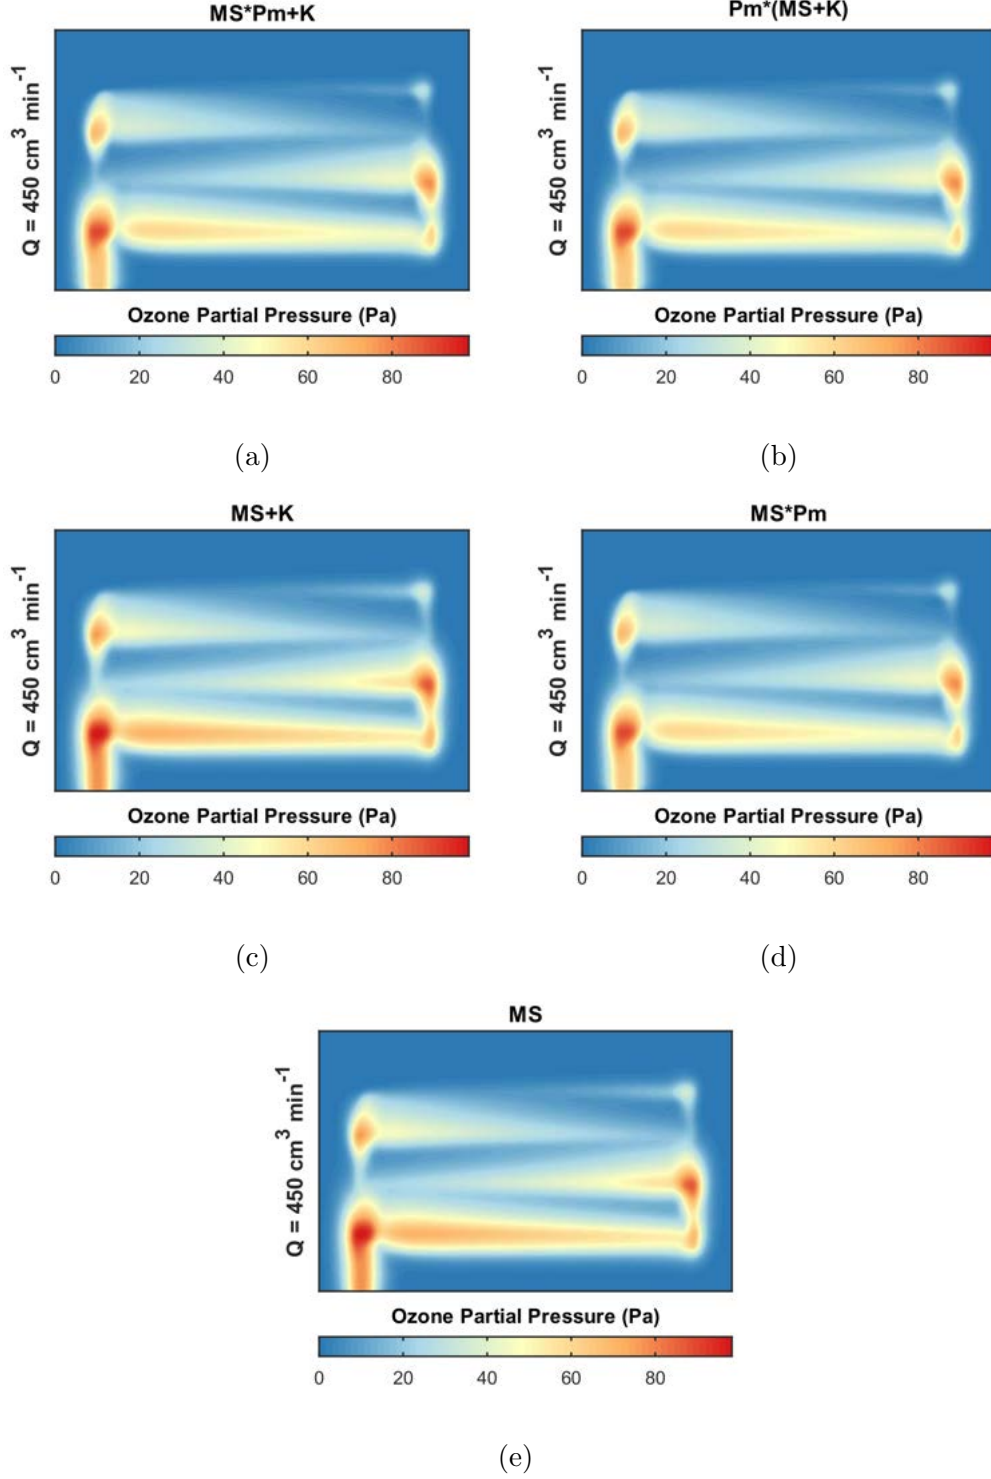

FIG. S7: Ozone partial pressure surfaces obtained at the upper boundary of the CL domain, for inlet flow rate  $Q = 450 \text{ cm}^3 \text{ min}^{-1}$ , using the follow coupling schemes: (a)  $MS * Pm + K$ , (b)  $Pm * (MS + K)$ , (c)  $MS + K$ , (d)  $MS * Pm$ , and (e)  $MS$ .

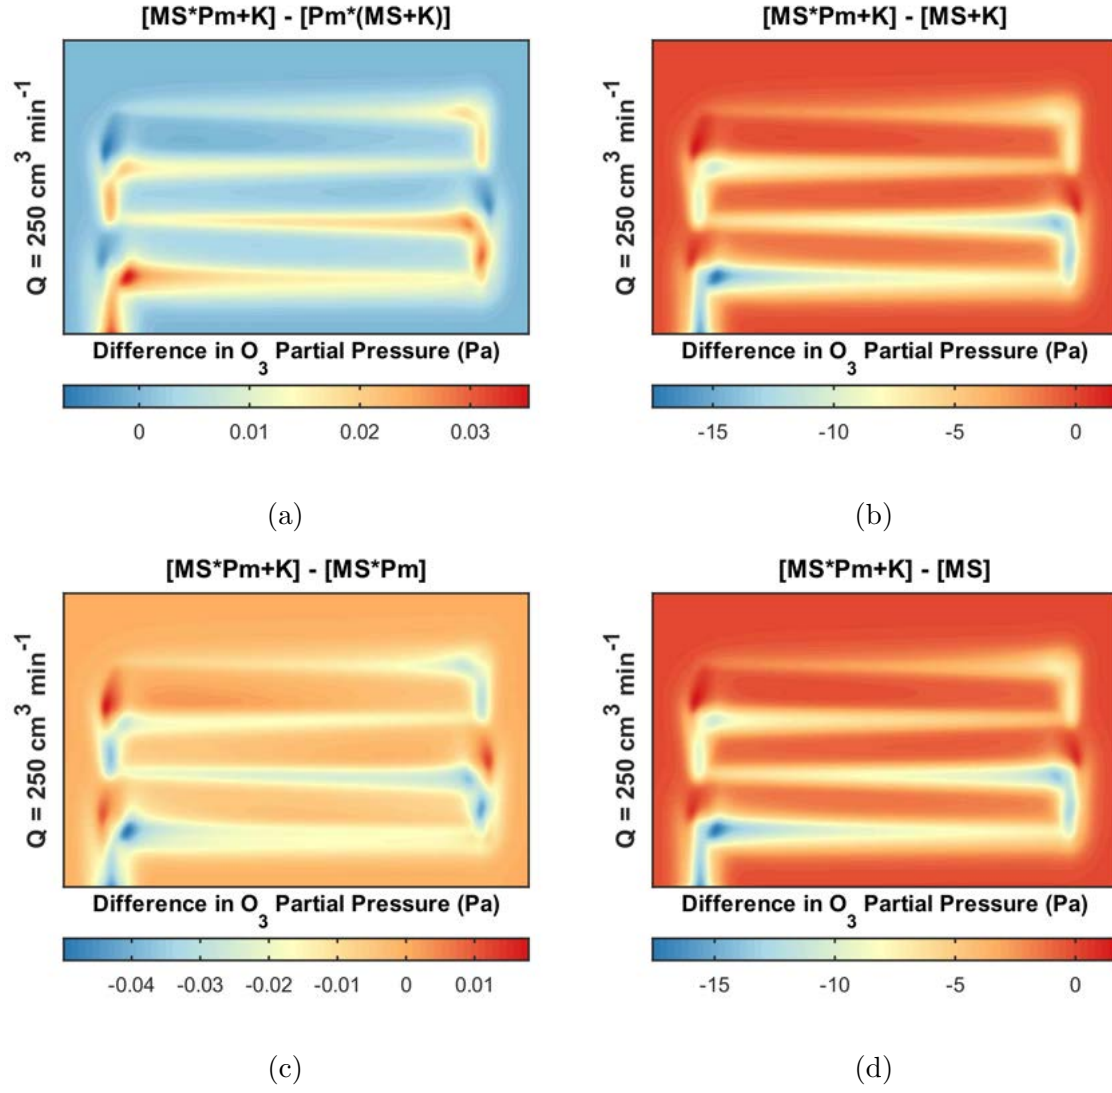

FIG. S8: Difference in ozone partial pressure surfaces between the preferable  $MS * Pm + K$  scheme and (a)  $Pm * (MS + K)$ , (b)  $MS + K$ , (c)  $MS * Pm$ , or (d)  $MS$ . All surfaces were obtained at  $Q = 250 \text{ cm}^3 \text{ min}^{-1}$ .

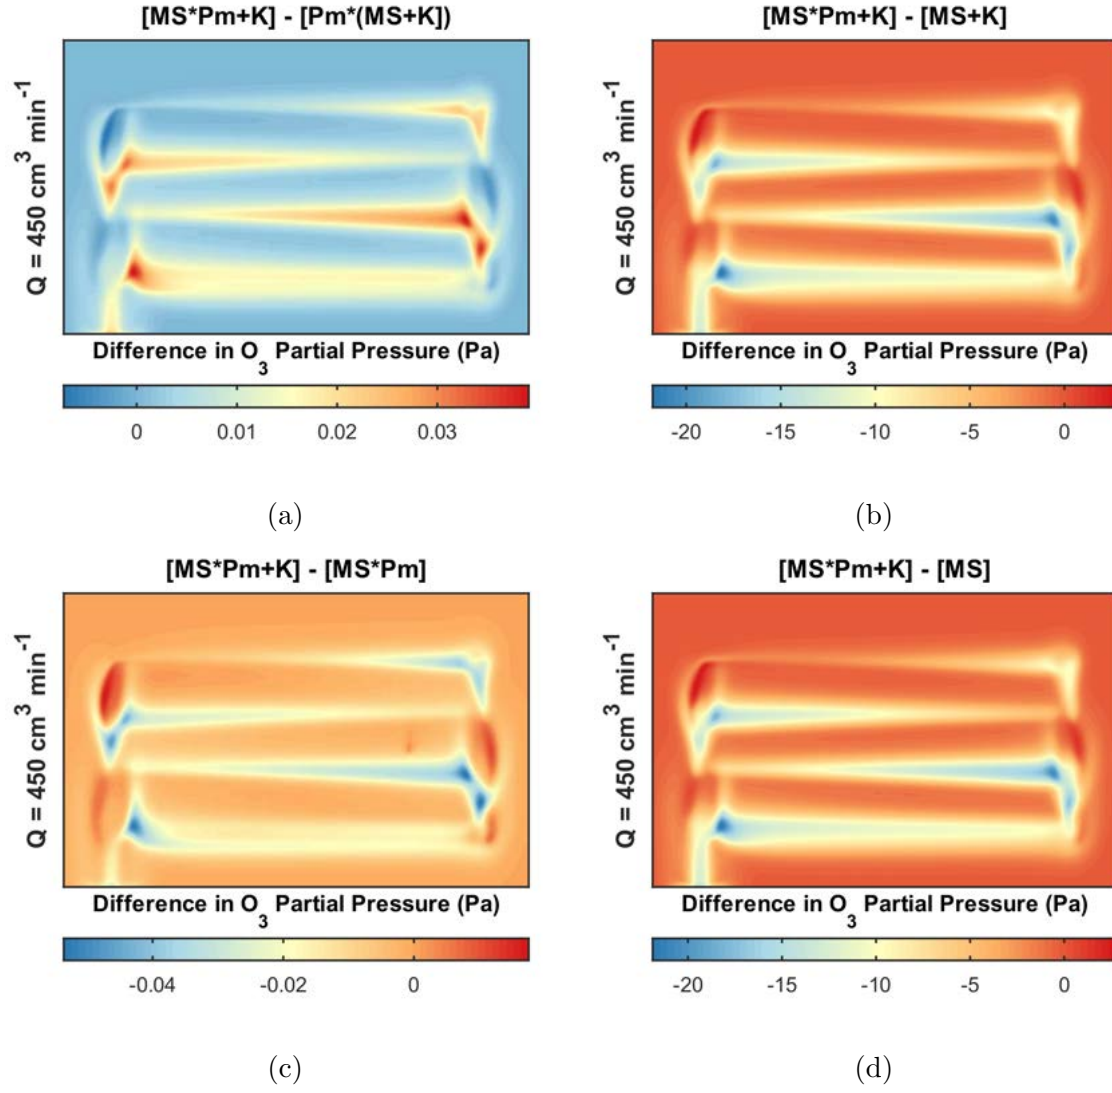

FIG. S9: Difference in ozone partial pressure surfaces between the preferable  $MS * Pm + K$  scheme and (a)  $Pm * (MS + K)$ , (b)  $MS + K$ , (c)  $MS * Pm$ , or (d)  $MS$ . All surfaces were obtained at  $Q = 450 \text{ cm}^3 \text{ min}^{-1}$ .

## SIV. MODEL COMPARISON

This section provides additional information on several points touched on in Section III.B of the paper. These include the A) flow field-related response variables; B) a brief comparison between SD and DB formulation for coupled free and porous media flow in the improved model Beta and for the chosen mesh; and C) plots with error estimates for the Beta model.

### A. Flow Field-related Variables

As described above, here will be presented the flow field-related response variables that were disregarded during the model comparison in the paper. These are the  $\Delta P/P_{\text{in}}$  ratio and  $\Delta P$ , as well as the  $U$  profiles along the  $x$  and  $z$  axes. These are given in Figures S10 and S11, respectively. In addition,  $P_{\text{O}_3}/R'_{\text{O}_3}$  profiles are provided in Figure S12, as mentioned in Section III.B.

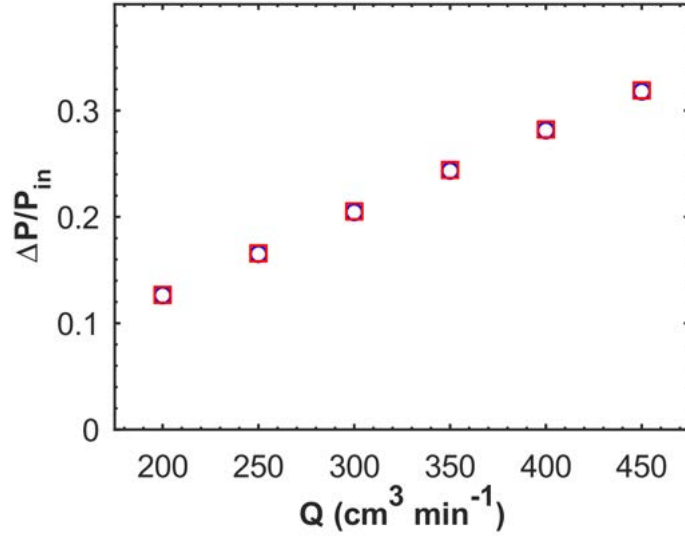

(a)

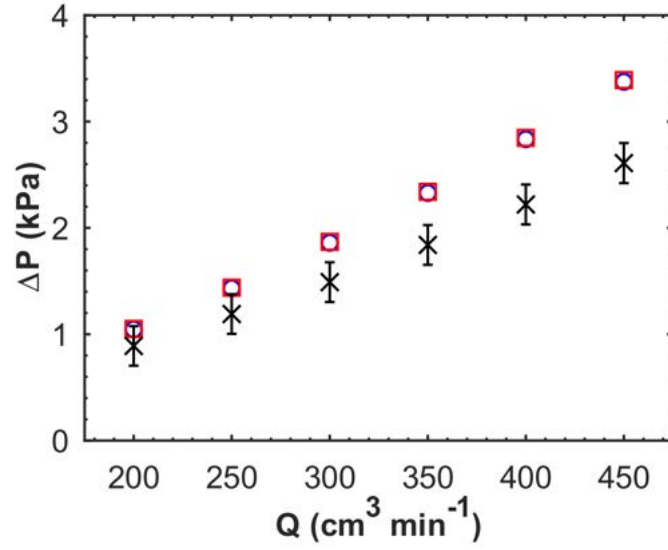

(b)

FIG. S10: Scalar response variables as a function of the inlet flow rate obtained for both Alpha ( $\circ$ ) and Beta ( $\square$ ) models: **(a)**  $\Delta P/P_{in}$  and **(b)**  $\Delta P$ . Also shown is the available experimental data[2] ( $\times$ ) as a reference.

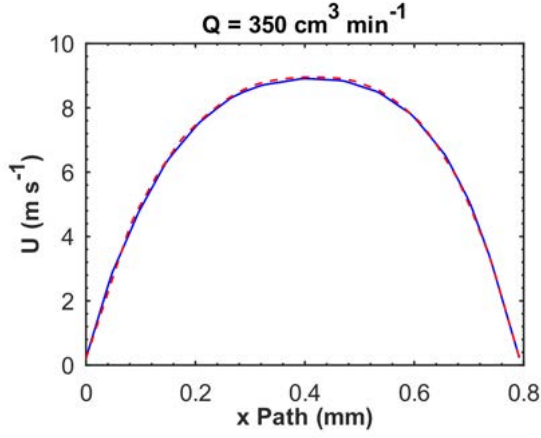

(a)

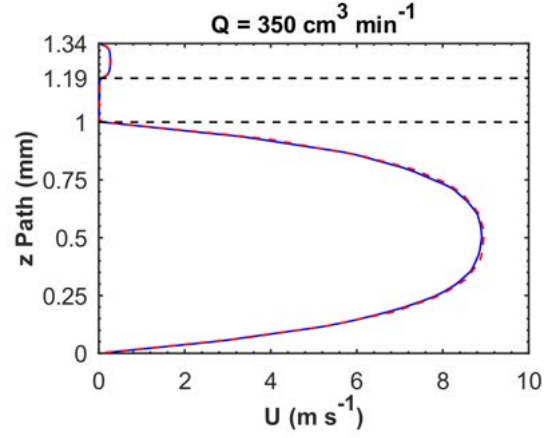

(b)

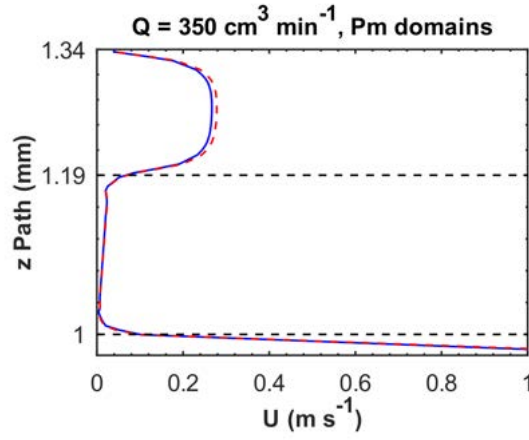

(c)

FIG. S11: Flow speed profiles for the Alpha (full lines) and Beta (dashed lines) models, with  $Q = 350 \text{ cm}^3 \text{ min}^{-1}$ : (a) profile along the  $x$  axis, (b) along the  $z$  axis, with (c) zoom in on the Pm domains. The dashed horizontal lines indicate the boundaries between domains.

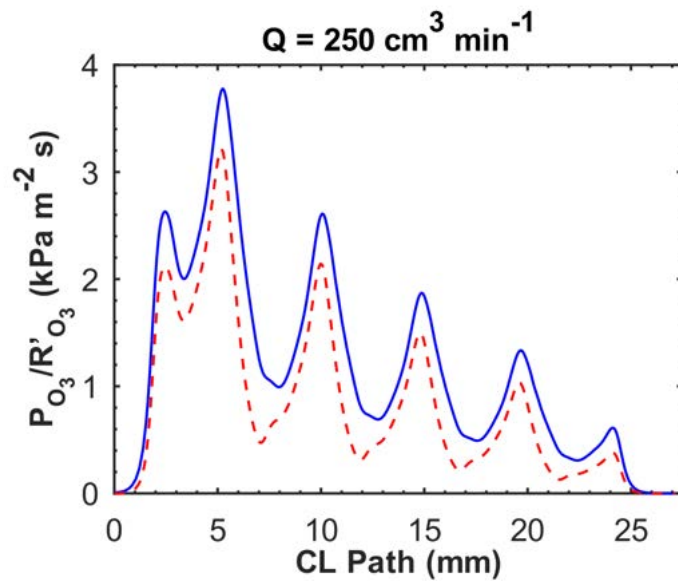

(a)

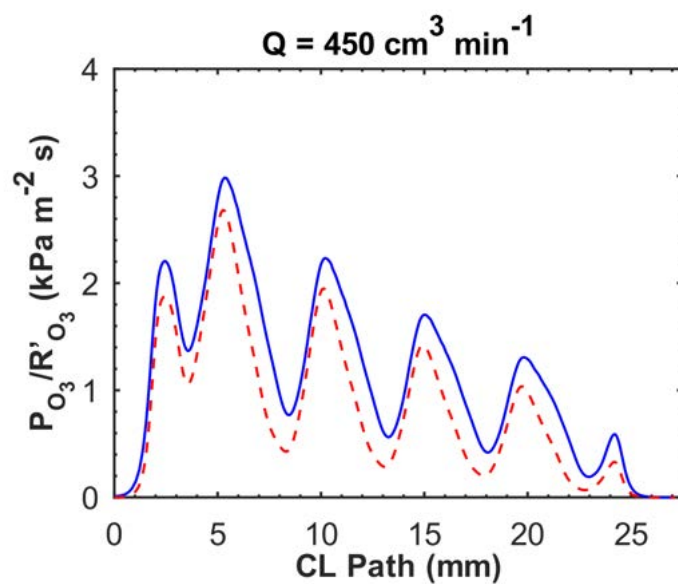

(b)

FIG. S12: Ozone partial pressure profiles normalized by their respective apparent reaction rates, for the Alpha (full lines) and Beta (dashed lines) models, for (a)  $Q = 250$  and (b)  $Q = 450 \text{ cm}^3 \text{ min}^{-1}$ .

## **B. Model Comparison with Error Estimates**

Here are provided duplicates of Fig. 3, Section III.A of the paper, and of Fig. S10, Section SIV A of this document, with the inclusion of error estimates for the Beta model. These are shown in Figures S13 and S14, respectively, where no discretization error was estimated for the Alpha model.

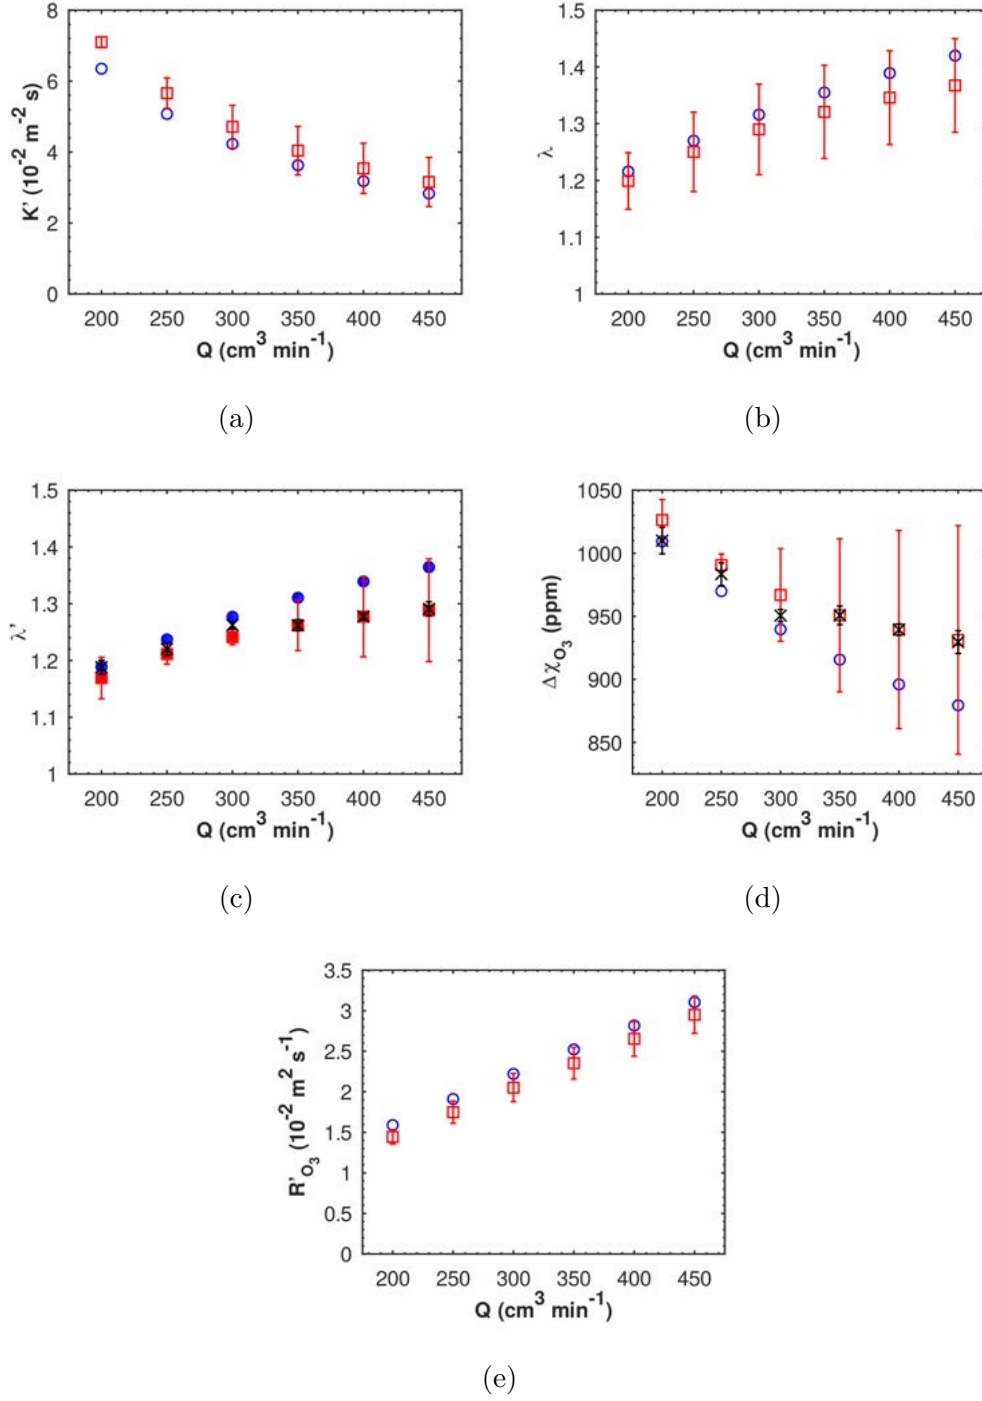

FIG. S13: Scalar response variables as function of inlet flow rate  $Q$  for both Alpha ( $\circ$ ) and Beta ( $\square$ ) models: **(a)**  $K' = \Delta\chi_{O_3}/R'_{O_3}$ , **(b)**  $\lambda$ , **(c)**  $\lambda'$ , **(d)**  $\Delta\chi_{O_3}$ , and **(e)**  $R'_{O_3}$ . Also shown are the available experimental data[2] ( $\times$ ) as a reference. Error bars show estimated discretization errors, for numerical results, and one standard deviation for experimental data.

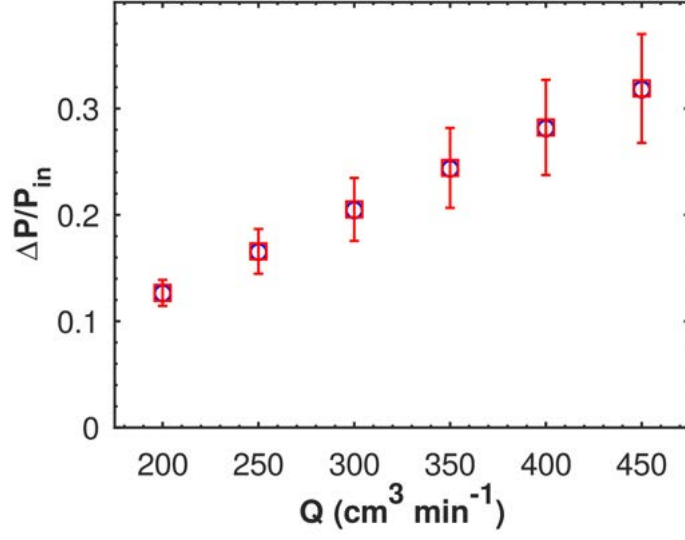

(a)

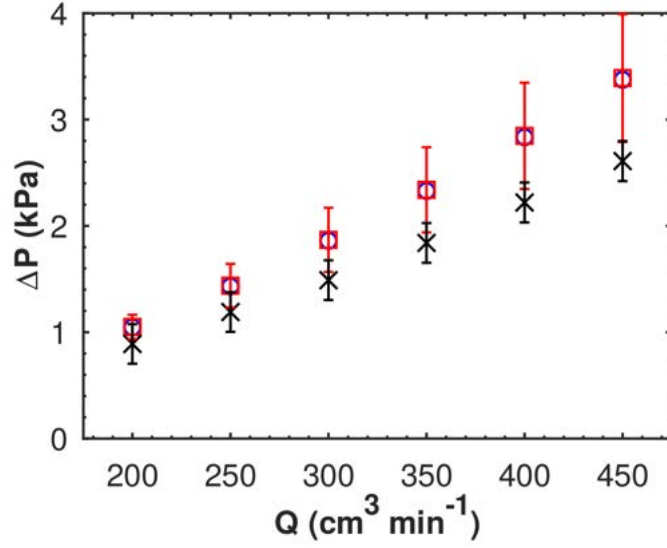

(b)

FIG. S14: Scalar response variables as function of inlet flow rate  $Q$  for both Alpha ( $\circ$ ) and Beta ( $\square$ ) models: (a)  $\Delta P/P_{\text{in}}$  and (b)  $\Delta P$ . Also shown are the available experimental data[2] ( $\times$ ) as a reference. Error bars show estimated discretization errors, for numerical results, and one standard deviation for experimental data.

### C. Stokes-Darcy and Darcy-Brinkman Formulations

For consistency, the SD formulation was used in both Alpha and Beta models, following [2]. The SD formulation is given by:

$$\rho(\mathbf{u} \cdot \nabla) \mathbf{u} = \nabla \left[ -P\mathbf{I} + \mu \left( \nabla \mathbf{u} + (\nabla \mathbf{u})^T \right) - \frac{2}{3} \mu (\nabla \cdot \mathbf{u}) \mathbf{I} \right] \quad (4)$$

$$\mathbf{u} = -\frac{\kappa}{\mu} \nabla P \quad (5)$$

in the Ch and Pm domains, respectively. The symbols follow the definitions used in the paper. The coupling between Ch and MPS domains is given by a slip length in the velocity field  $\mathbf{u}$  at the boundary separating both domains:

$$\mathbf{u} = \frac{L_s}{\mu} \tau_{n,t} \quad (6)$$

where  $\tau_{n,t}$  is the tangential shear stress at the boundary, and the slip length  $L_s$  is defined following [5]:

$$L_s = c \sqrt{\frac{\kappa}{\epsilon}} \quad (7)$$

where  $c = 1$  as in [2]. Only the pressure was continuous along the boundary, which, according to LeBars and Worster[5], is the same as the interface condition presented by Beavers and Joseph[6]. Finally, the Ch and Pm domains were coupled in this case, removing the need for explicit continuity equations for the variables. This might have resulted in differences in the mesh, however this was not pursued. The remaining of the models were as described in the paper.

The comparison between SD and DB formulations was done using the same variables of interest as in the paper. Thus, Figures S15 and S16 shows the scalar response variables,  $K'$ ,  $\lambda$ ,  $\lambda'$ ,  $\Delta\chi_{\text{O}_3}$ ,  $R'_{\text{O}_3}$ ,  $\Delta P/P_{\text{in}}$ , and  $\Delta P$ . Figure S17 presents the  $U$  profiles along the  $x$  and  $z$  axes. Figure S18 shows the  $P_{\text{O}_3}$  and  $\bar{R}_{\text{O}_3}$  profiles at the CL upper boundary, for  $Q = 250$  and  $450 \text{ cm}^3 \text{ min}^{-1}$ . Finally, Figures S19 and S20 shows the  $\mathbf{P}_{\text{O}_3}$  surfaces for  $Q = 250$  and  $450 \text{ cm}^3 \text{ min}^{-1}$ , respectively, as well as the differences between DB and SD surfaces for each model.

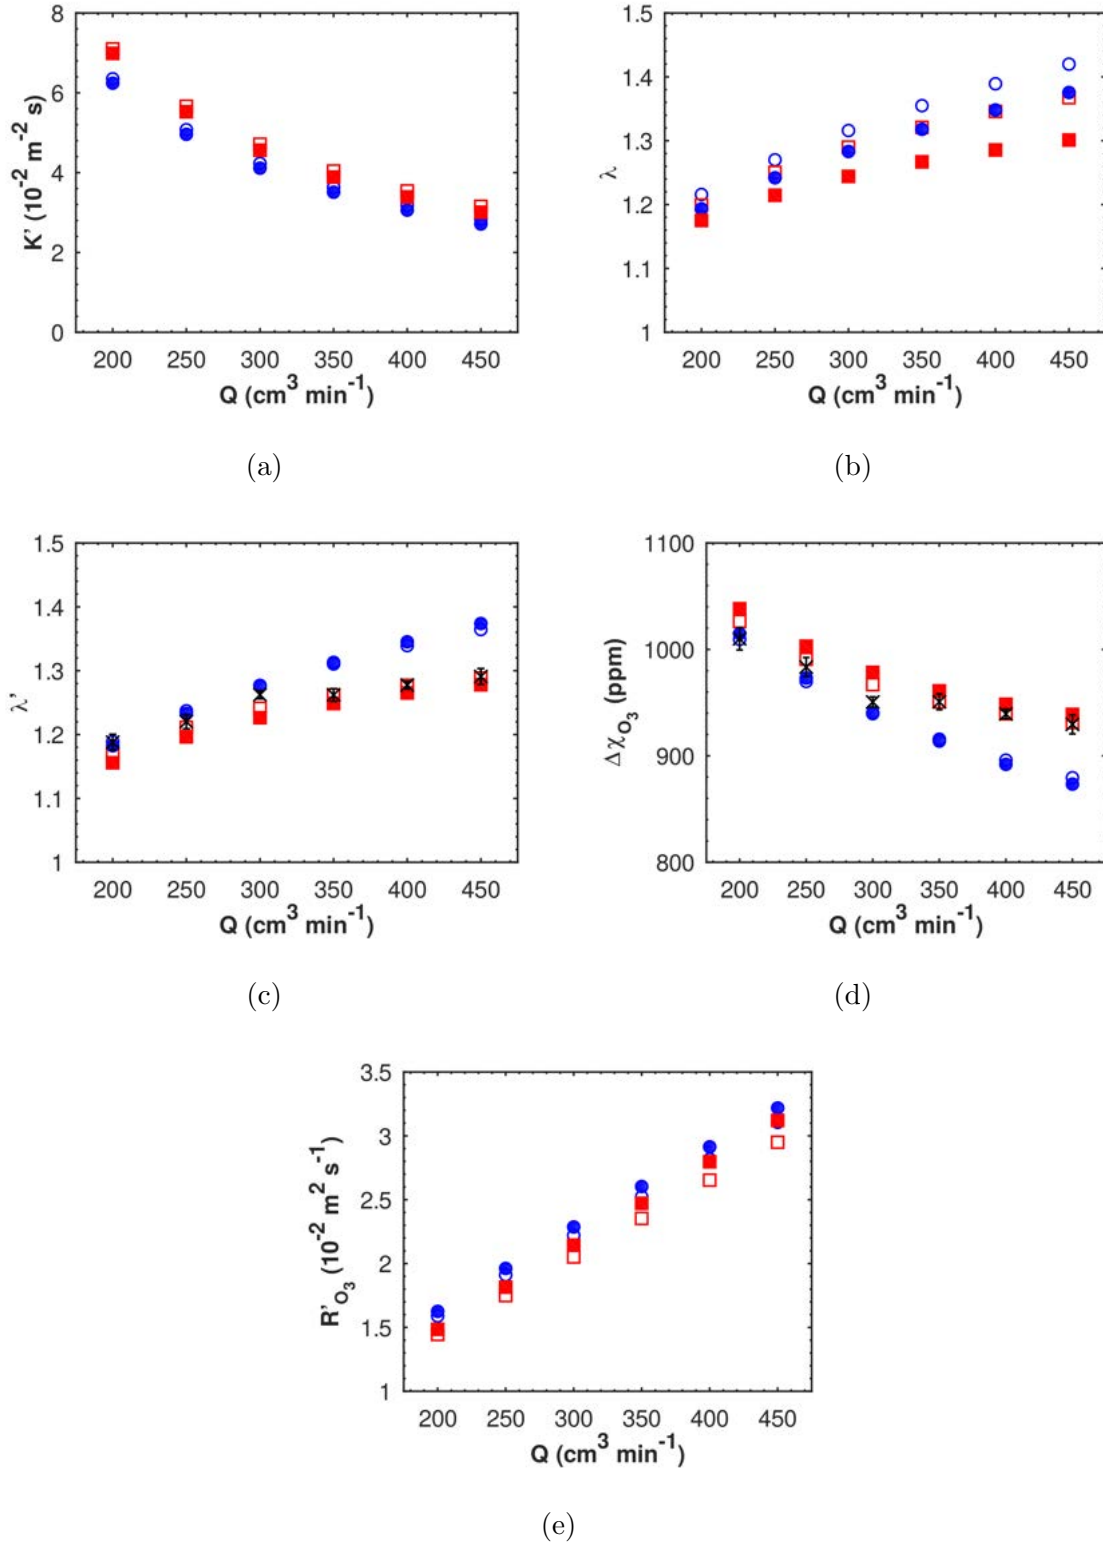

FIG. S15: Scalar variables as function of inlet flow rate  $Q$  for both Alpha ( $\circ$ ) and Beta ( $\square$ ) models: (a)  $K' = \Delta\chi_{O_3}/R'_{O_3}$ , (b)  $\lambda$ , (c)  $\lambda'$ , (d)  $\Delta\chi_{O_3}$ , and (e)  $R'_{O_3}$ . Shown are the DB (empty marker) and SD (full marker) formulations for each model.

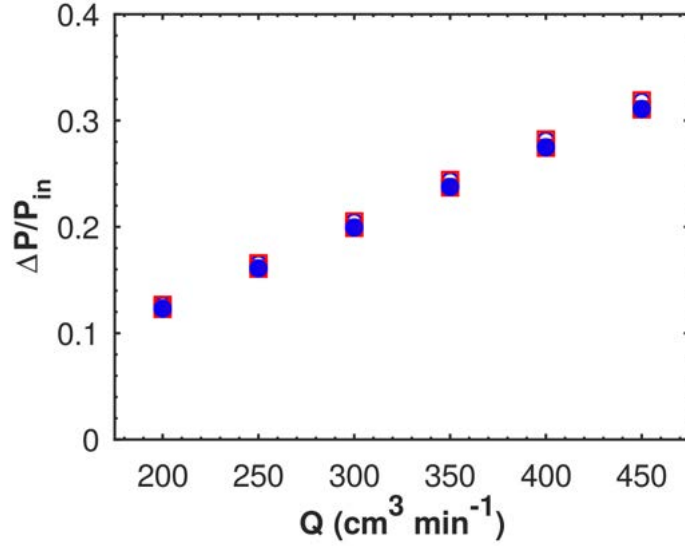

(a)

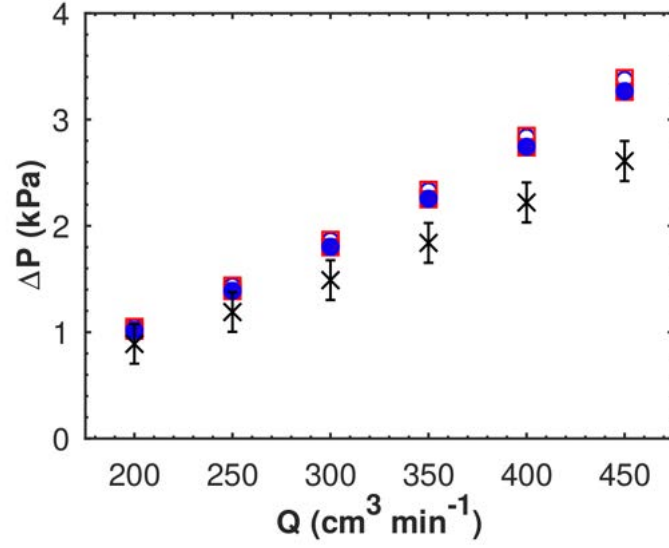

(b)

FIG. S16: Scalar variables as function of inlet flow rate  $Q$  for both Alpha (○) and Beta (□) models: (a)  $\Delta\chi_{O_3}/R'_{O_3}$ , (b)  $\Delta P/P_{in}$ , (c)  $\Delta\chi_{O_3}$ , (d)  $R'_{O_3}$ , and (e)  $\Delta P$ . Shown are the DB (empty marker) and SD (full marker) formulations for each model.

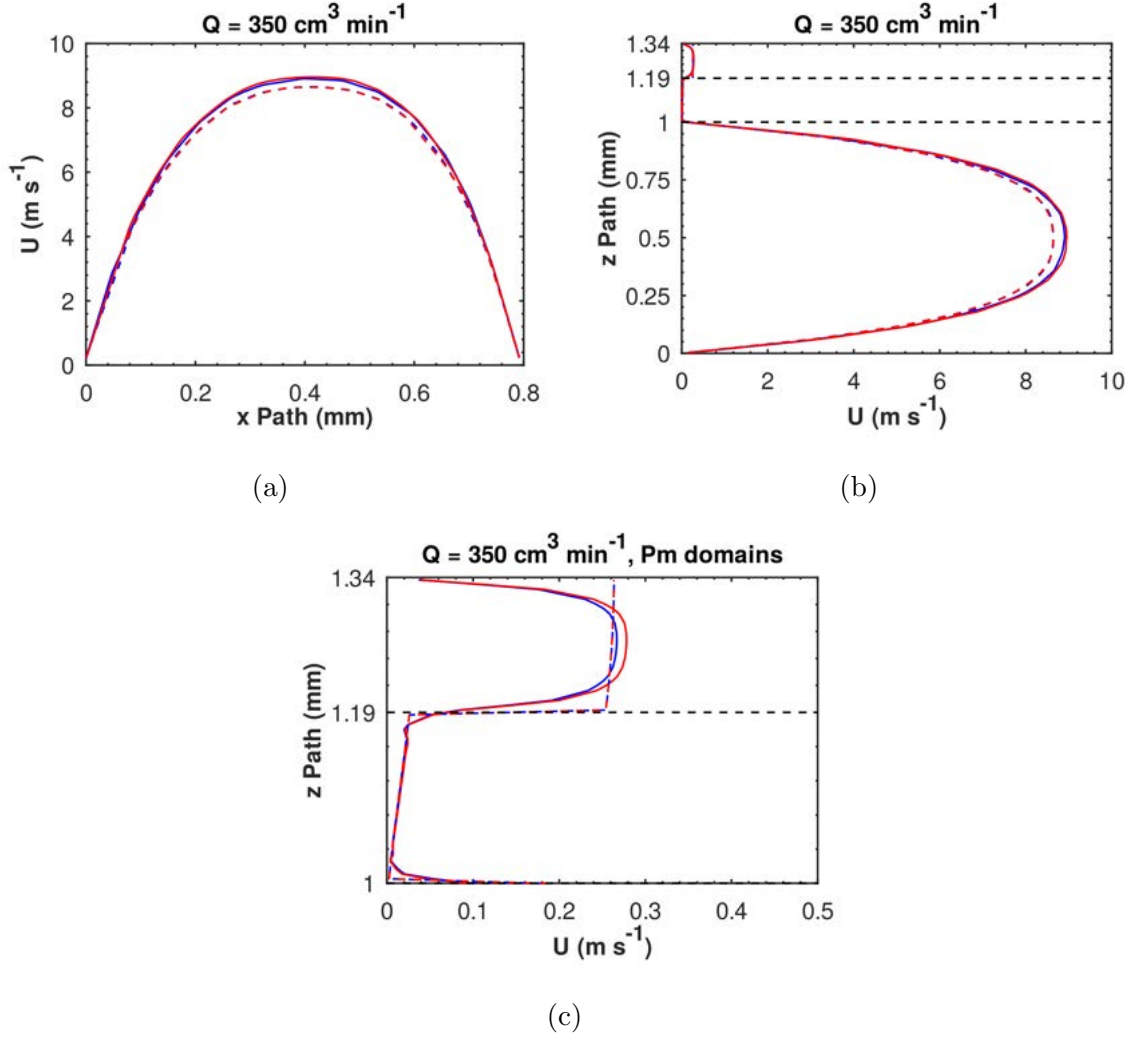

FIG. S17: Flow speed profiles for the Alpha) and Beta) models, with  $Q = 350 \text{ cm}^3 \text{ min}^{-1}$ ), using either the DB (full lines) or SD (dashed lines) formulations: **(a)** profile along the  $x$  axis, **(b)** along the  $z$  axis, with **(c)** zoom in on the Pm domains. The dashed horizontal lines indicate the boundaries between domains.

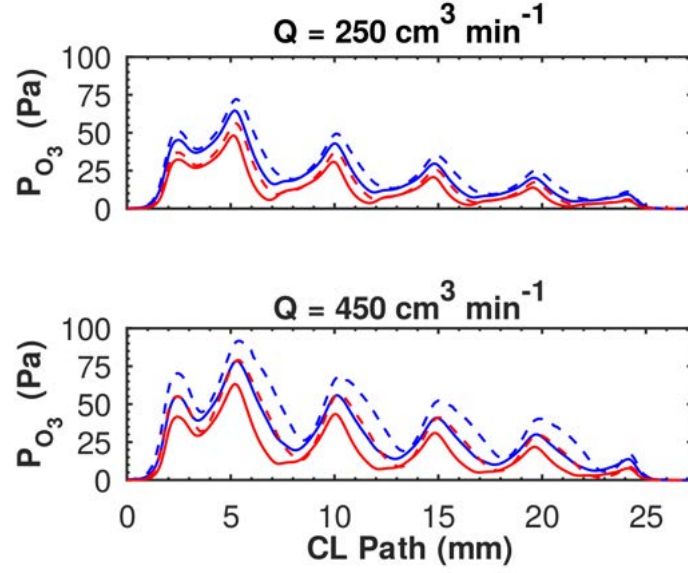

(a)

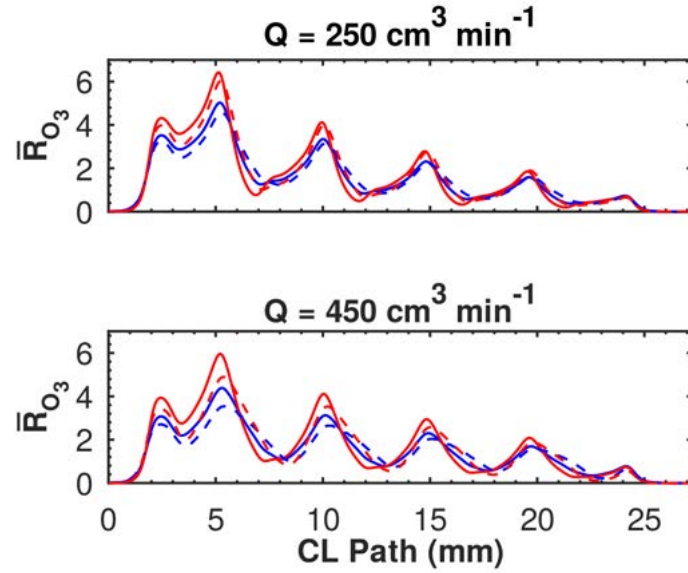

(b)

FIG. S18: (a) Partial pressure and (b) normalized reaction rate profiles as function of the path along the CL upper boundary, for inlet flow rates  $Q = 250$  (top) and  $450 \text{ cm}^3 \text{ min}^{-1}$  (bottom). Both models are shown, **Alpha** and **Beta**, using the DB (full lines) and SD (dashed lines) formulations for each model.

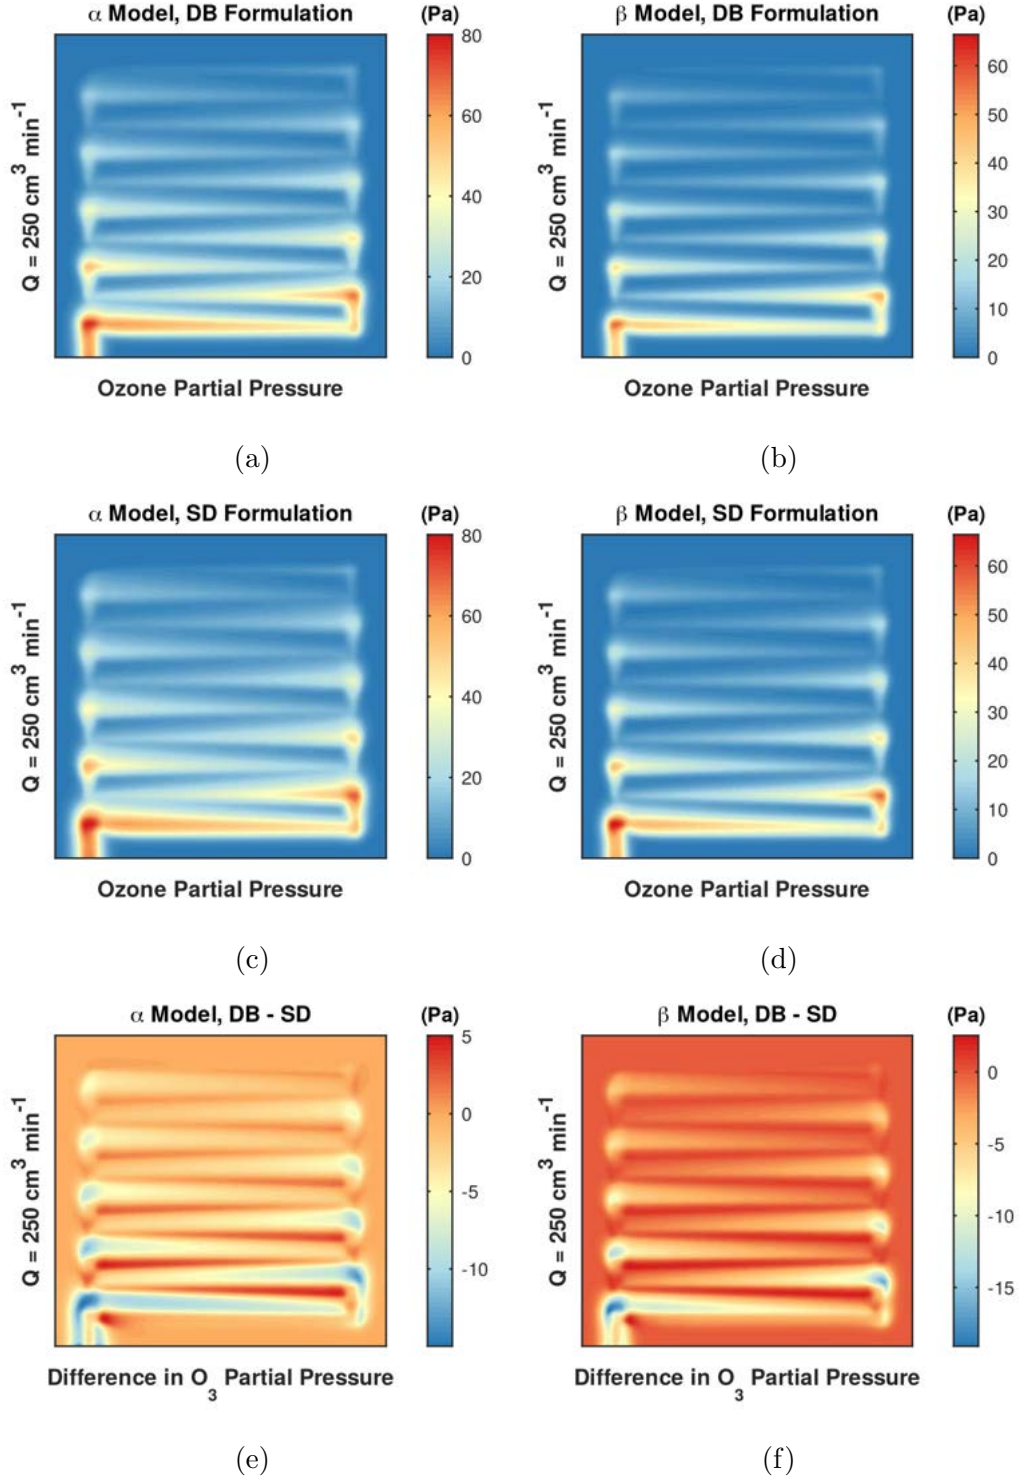

FIG. S19: Ozone partial pressure surfaces obtained at the upper boundary of the CL domain, for inlet flow rate  $Q = 250 \text{ cm}^3 \text{ min}^{-1}$ : (a) Alpha and (b) Beta models with DB formulation, (c) Alpha and (d) Beta models with SD formulation, (e) difference between (a) and (c), and (f) difference between (b) and (d).

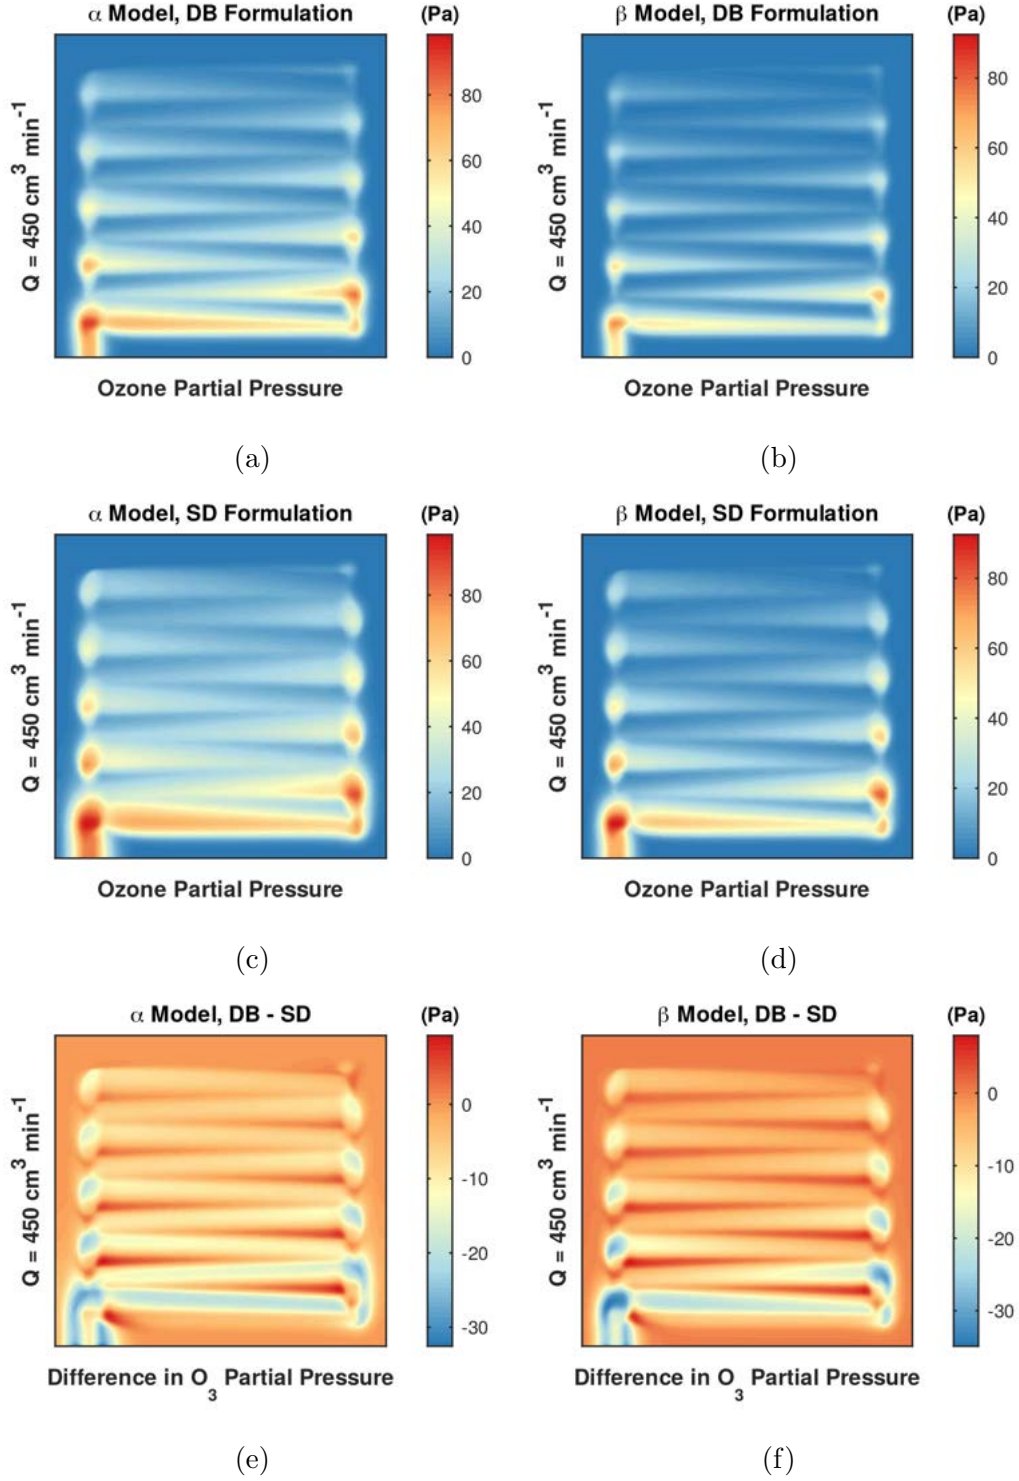

FIG. S20: Ozone partial pressure surfaces obtained at the upper boundary of the CL domain, for inlet flow rate  $Q = 450 \text{ cm}^3 \text{ min}^{-1}$ : (a) Alpha and (b) Beta models with DB formulation, (c) Alpha and (d) Beta models with SD formulation, (e) difference between (a) and (c), and (f) difference between (b) and (d).

## SV. PARAMETRIC STUDY OF REACTION RATE CONSTANTS

This section provides additional information on response variables used in Section III.B of the paper, concerning the parametric study on the reaction rate constants  $k_1$  and  $k_2$ . Figure S21 provide the relative difference in  $\Delta\chi_{\text{O}_3}$  and  $R'_{\text{O}_3}$  as  $k_2$  increases for a fixed  $k_1$ . Figure S22 presents the scalar response variables  $K = \Delta\chi_{\text{O}_3}/R_{\text{O}_3}$  and  $R_{\text{O}_3}$ , which analogous to the ones used in the paper,  $K'$  and  $R'_{\text{O}_3}$ , however using the total reaction rate  $R_{\text{O}_3}$ . Figure S23 provides the  $K'$  ration and stoichiometries  $\lambda$  and  $\lambda'$  in full range, complementing Fig. 7d of the paper. Figure S24 shows the effect of  $k_1$  and  $k_2$  on the  $P_{\text{O}_3}$  profile at the CL, for  $Q = 250$  and  $450 \text{ cm}^3 \text{ min}^{-1}$ , as well as the relative difference between increasing values of  $k_2$  for fixed  $k_1 = 10^2 \text{ s}^{-1}$ . Figures S25 through S28 shows the  $\bar{\mathbf{R}}_{\text{O}_3}$  surfaces for selected values of  $k_2$  and fixed  $k_1$ , for  $Q = 250, 350$ , and  $450 \text{ cm}^3 \text{ min}^{-1}$ . Figure S29 provides the  $\bar{\mathbf{R}}_{\text{O}_3}$  further normalized by the surface's maximum value for  $k_1 = 10^2 \text{ s}^{-1}$ ,  $k_2 = 10^{-1}$  and  $10 \text{ s}^{-1}$ , and  $Q = 250$  and  $450 \text{ cm}^3 \text{ min}^{-1}$ . Finally, Figures S30 through S33 shows the  $\mathbf{P}_{\text{O}_3}$  surfaces for selected values of  $k_2$  and fixed  $k_1$ , for  $Q = 250, 350$ , and  $450 \text{ cm}^3 \text{ min}^{-1}$ .

- 
- [1] T. Lopes, M. Ho, B. K. Kakati, and A. R. J. Kucernak. Assessing the performance of reactant transport layers and flow fields towards oxygen transport: A new imaging method based on chemiluminescence. *J. Power Sources*, 274:382–392, 2015.
  - [2] O. Beruski, T. Lopes, A. R. Kucernak, and J. Perez. Investigation of convective transport in the so-called “gas diffusion layer” used in polymer electrolyte fuel cell. *Phys. Rev. Fluids*, 2:103501, 2017.
  - [3] M. L. Huber and A. H. Harvey. Diffusion in gases. In W. M. Haynes, editor, *CRC handbook of chemistry and physics*, chapter 6, pages 259–260. CRC, Boca Raton, 95<sup>a</sup> edition, 2015.
  - [4] T. R. Marrero and E. A. Mason. Gaseous diffusion coefficients. *Journal of Physical and Chemical Reference Data*, 1:3–118, 1972.
  - [5] M. Le Bars and M. G. Worster. Interfacial conditions between pure fluid and a porous medium: implications for binary alloy solidification. *Journal of Fluid Mechanics*, 550:149–173, 2006.
  - [6] G. S. Beavers and D. D. Joseph. Boundary conditions at a naturally permeable wall. *Journal of Fluid Mechanics*, 30:197–207, 1967.

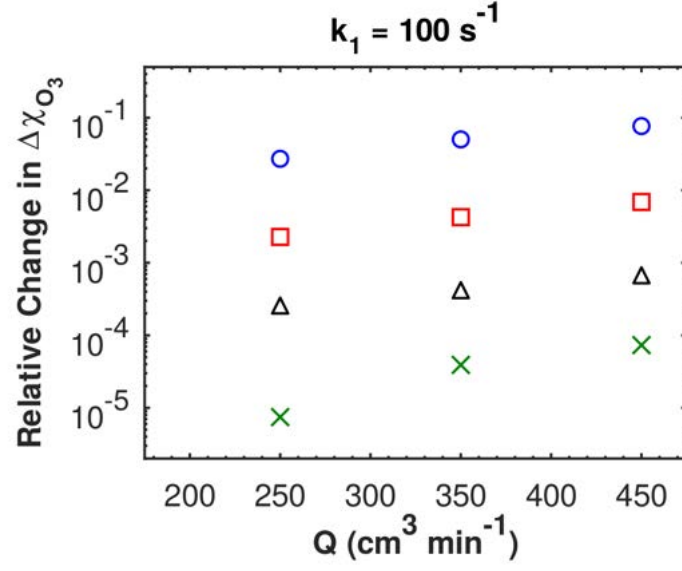

(a)

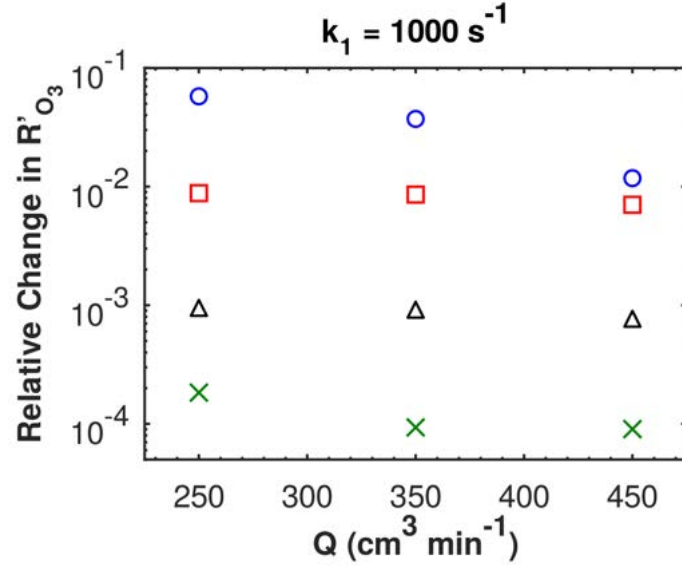

(b)

FIG. S21: Relative change in scalar response variables, as function of inlet flow rate, as  $k_2$  increases for fixed  $k_1$ : **(a)**  $\Delta\chi_{\text{O}_3}$  for  $k_1 = 10^2 \text{ s}^{-1}$  and **(b)**  $R'_{\text{O}_3}$  for  $k_1 = 10^3 \text{ s}^{-1}$ . Color code:

$k_2 = 1 - k'_2 = 10^{-1}$  ( $\circ$ ),  $k_2 = 10 - k'_2 = 1$  ( $\square$ ),  $k_2 = 10^2 - k'_2 = 10$  ( $\triangle$ ), and  $k_2 = 10^3 - k'_2 = 10^2$  ( $\times$ ).

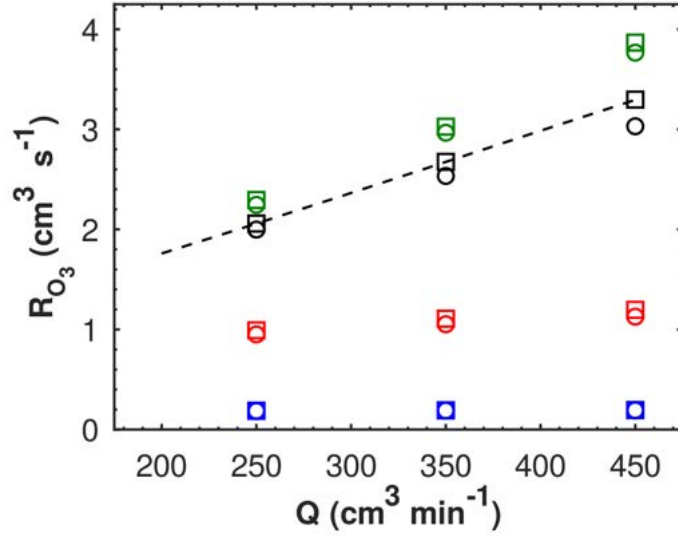

(a)

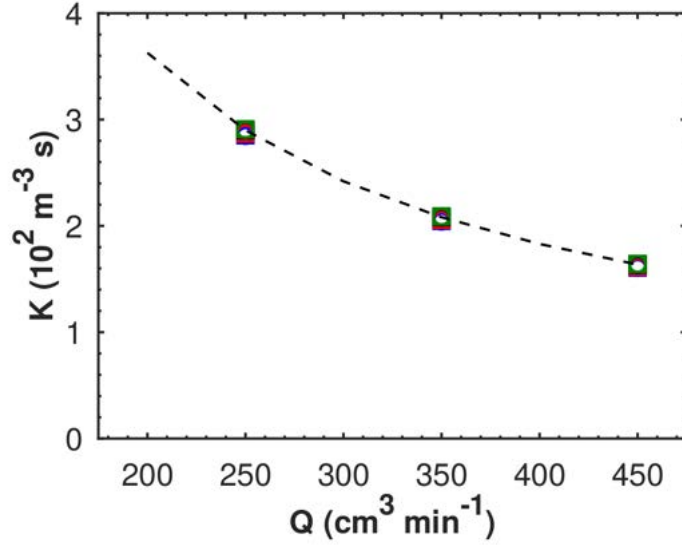

(b)

FIG. S22: Scalar response variables as function of the inlet flow rate for the Beta model, using different combinations of  $k_1$  and  $k_2$ : **(a)**  $R_{O_3}$  and **(b)**  $K = \Delta\chi_{O_3}/R_{O_3}$ . Different colors map the values of  $k_1$ : 1, 10,  $10^2$ , and  $10^3$  s<sup>-1</sup>; while the values of  $k_2$  are mapped by different symbols:  $10^{-1}$  (○) and  $10^3$  s<sup>-1</sup> (□).

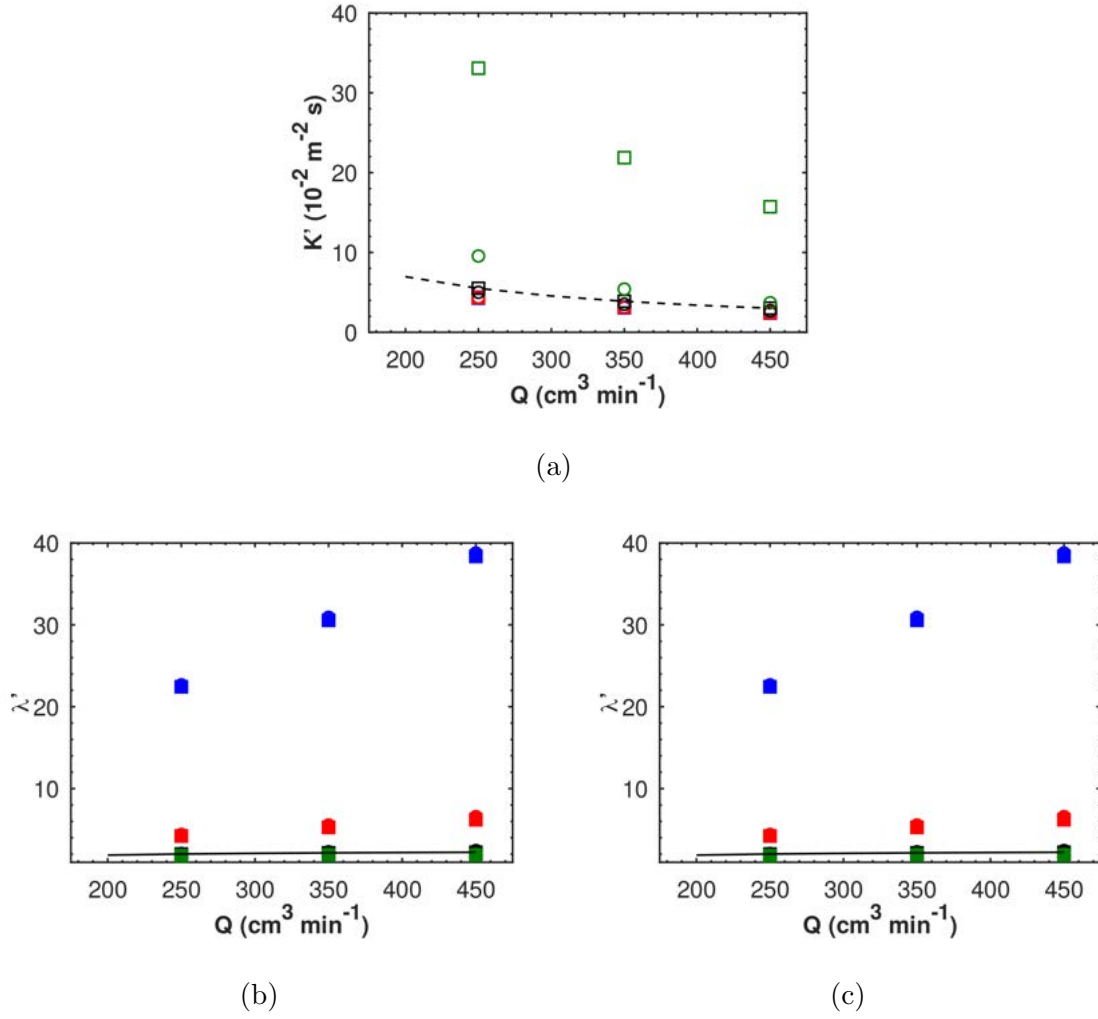

FIG. S23: Full range for the scalar response variables as function of the inlet flow rate for the Beta model, using different combinations of  $k_1$  and  $k_2$ : **(a)**  $\lambda$  and **(b)**  $\lambda'$ . Different colors map the values of  $k_1$ : 1, 10,  $10^2$ , and  $10^3$   $\text{s}^{-1}$ ; while the values of  $k_2$  are mapped by different symbols:  $10^{-1}$  (o) and  $10^3$   $\text{s}^{-1}$  ( $\square$ ).

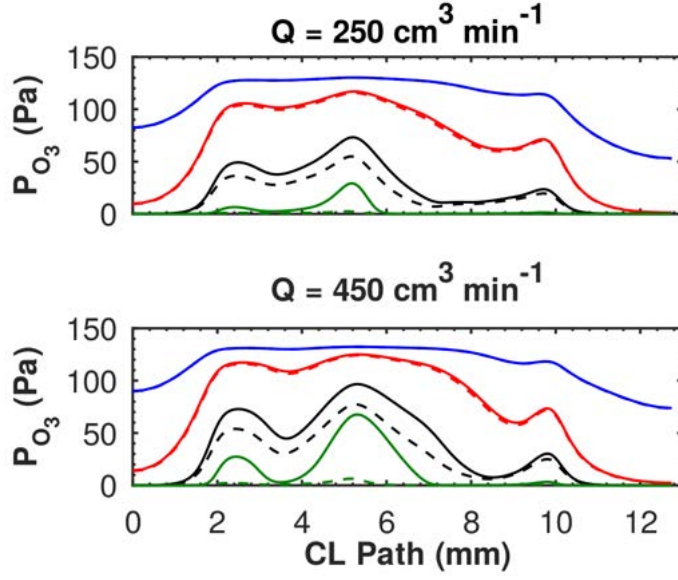

(a)

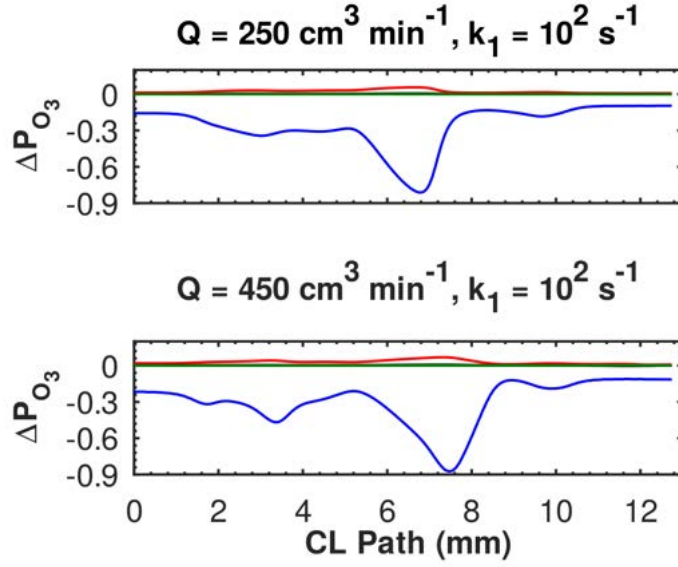

(b)

FIG. S24: Profiles associated with the ozone partial pressure, at  $Q = 250$  (top) and  $450 \text{ cm}^3 \text{ min}^{-1}$  (bottom), for selected values of  $k_1$  and  $k_2$ . **(a)** Normalized reaction rate profiles, with  $k_1 = 1, 10, 10^2$ , and  $10^3 \text{ s}^{-1}$ ; and  $k_2$ :  $10^{-1}$  (full lines) and  $10^3 \text{ s}^{-1}$  (dashed lines).

**(b)** Relative difference between profiles for increasing values of  $k_2$ , using

$$k_1 = 10^2 \text{ s}^{-1}: k_2 = 1 - k'_2 = 10^{-1}, k_2 = 10 - k'_2 = 1, k_2 = 10^2 - k'_2 = 10, \text{ and}$$

$$k_2 = 10^3 - k'_2 = 10^2.$$

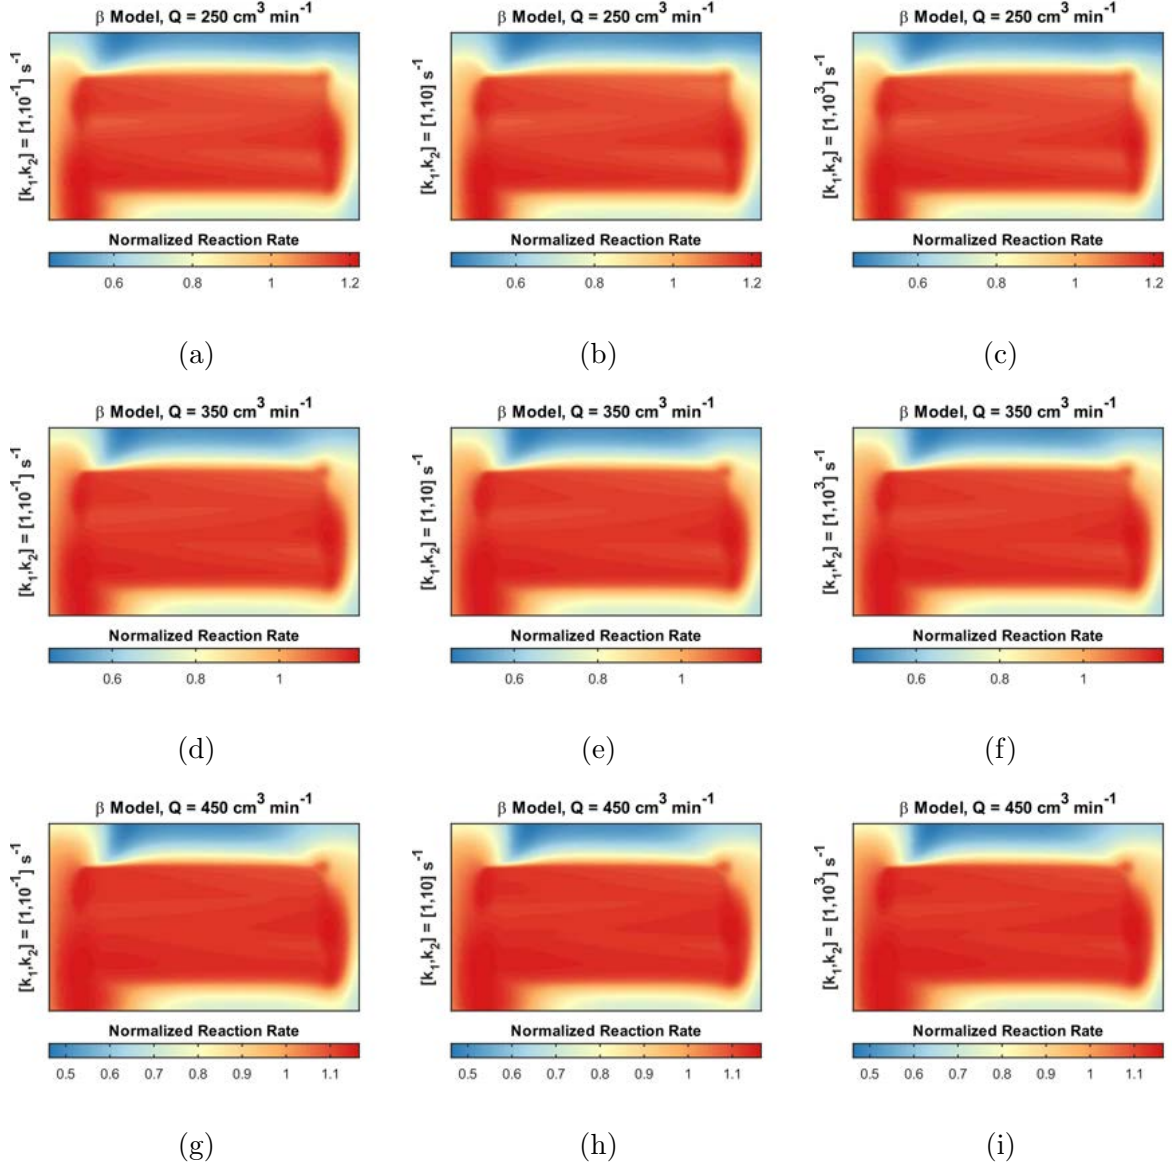

FIG. S25: Normalized reaction rate surfaces for  $k_1 = 1 \text{ s}^{-1}$ , with  $Q = 250$  (top row), 350 (middle row), and  $Q = 450 \text{ cm}^3 \text{ min}^{-1}$  (bottom row); and  $k_2 = 10^{-1}$  (left column), 10 (central column), and  $10^3 \text{ s}^{-1}$  (right column).

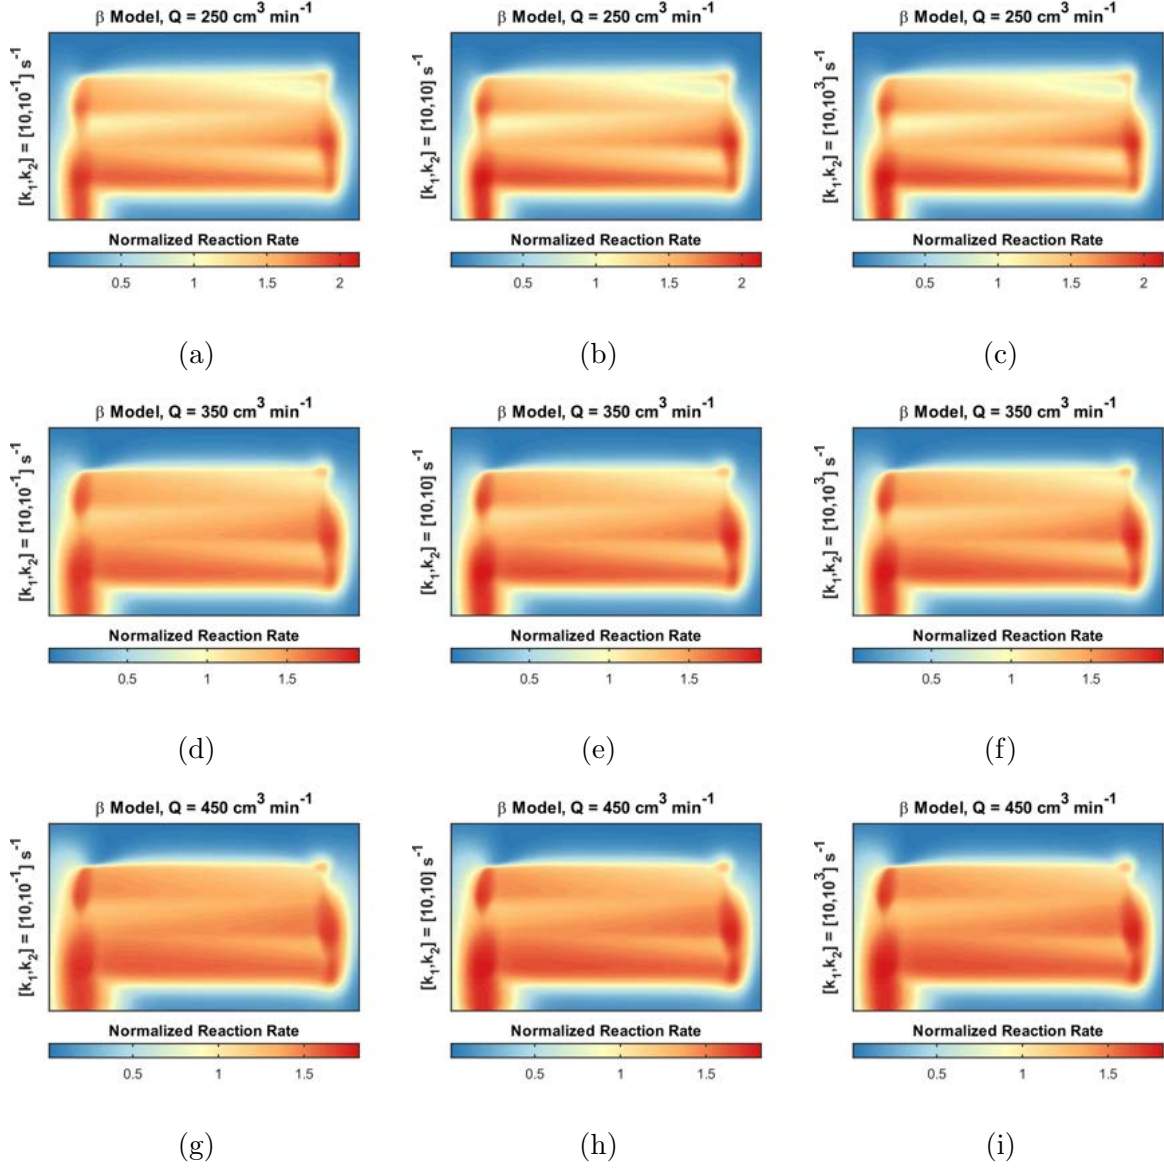

FIG. S26: Normalized reaction rate surfaces for  $k_1 = 10 \text{ s}^{-1}$ , with  $Q = 250$  (top row), 350 (middle row), and  $Q = 450 \text{ cm}^3 \text{ min}^{-1}$  (bottom row); and  $k_2 = 10^{-1}$  (left column), 10 (central column), and  $10^3 \text{ s}^{-1}$  (right column).

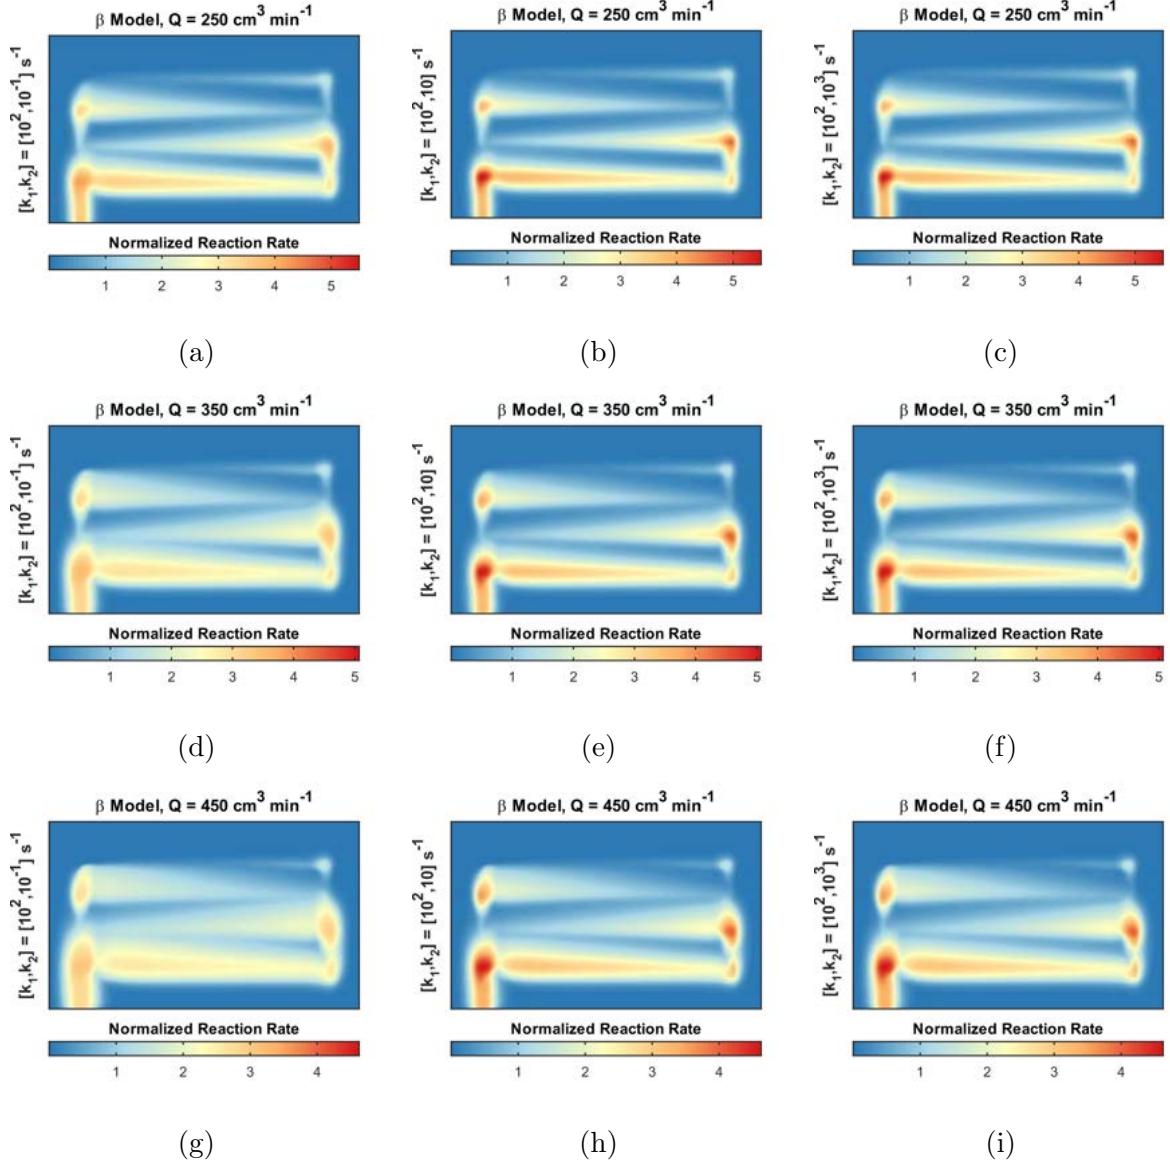

FIG. S27: Normalized reaction rate surfaces for  $k_1 = 10^2 \text{ s}^{-1}$ , with  $Q = 250$  (top row), 350 (middle row), and  $Q = 450 \text{ cm}^3 \text{min}^{-1}$  (bottom row); and  $k_2 = 10^{-1}$  (left column), 10 (central column), and  $10^3 \text{ s}^{-1}$  (right column).

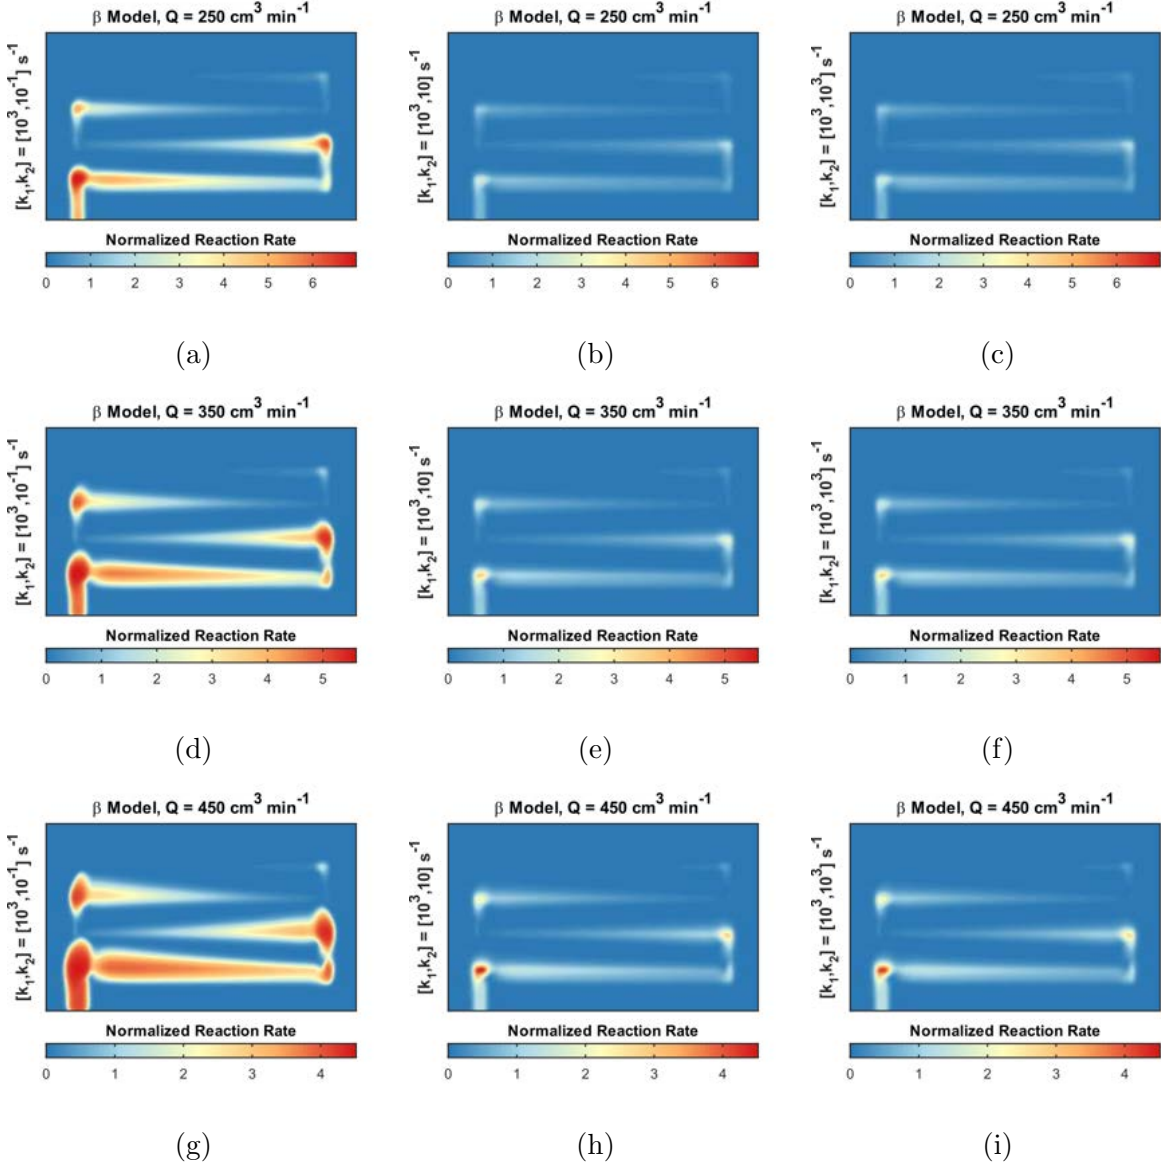

FIG. S28: Normalized reaction rate surfaces for  $k_1 = 10^3 \text{ s}^{-1}$ , with  $Q = 250$  (top row), 350 (middle row), and  $Q = 450 \text{ cm}^3 \text{ min}^{-1}$  (bottom row); and  $k_2 = 10^{-1}$  (left column), 10 (central column), and  $10^3 \text{ s}^{-1}$  (right column).

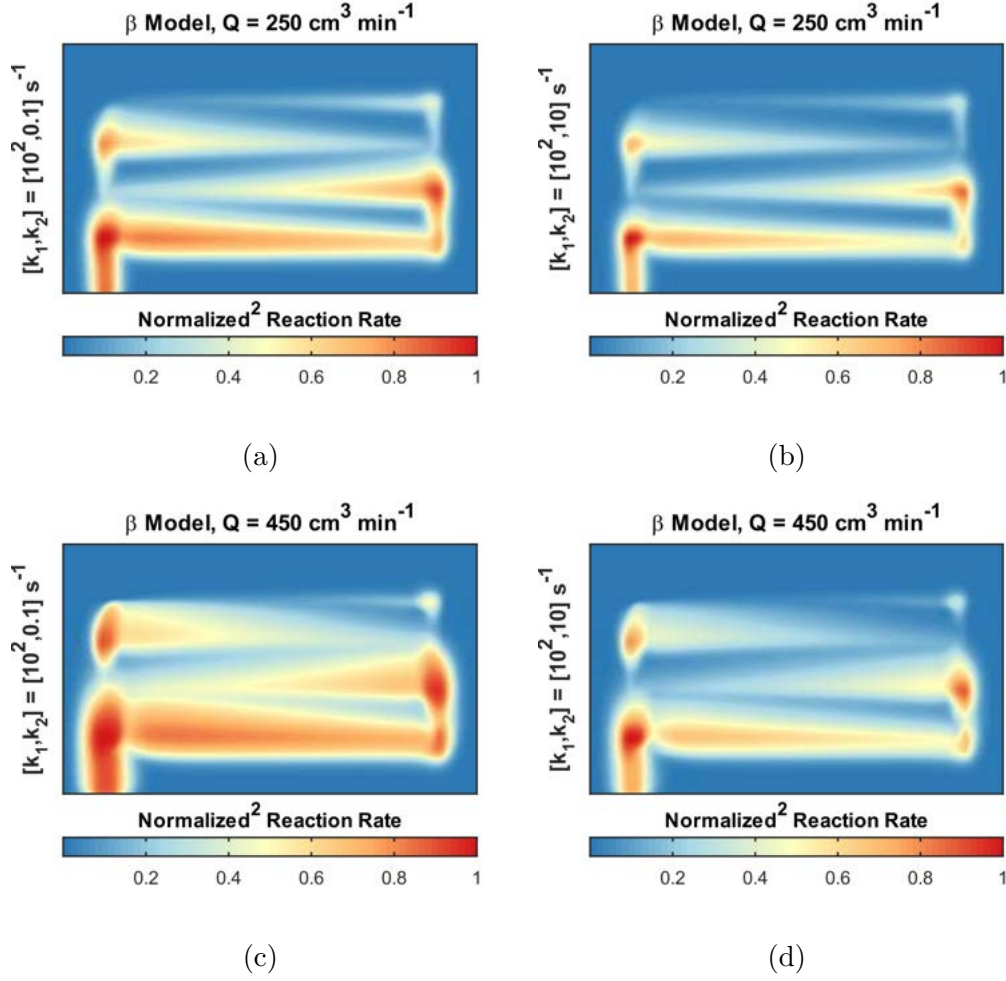

FIG. S29: Doubly normalized reaction rate surfaces for  $k_1 = 10^2 \text{ s}^{-1}$ , with  $Q = 250$  (top row) and  $Q = 450 \text{ cm}^3 \text{ min}^{-1}$  (bottom row), and  $k_2 = 10^{-1}$  (left column) and  $10 \text{ s}^{-1}$  (right column). The surfaces are normalized by their respective maximum values.

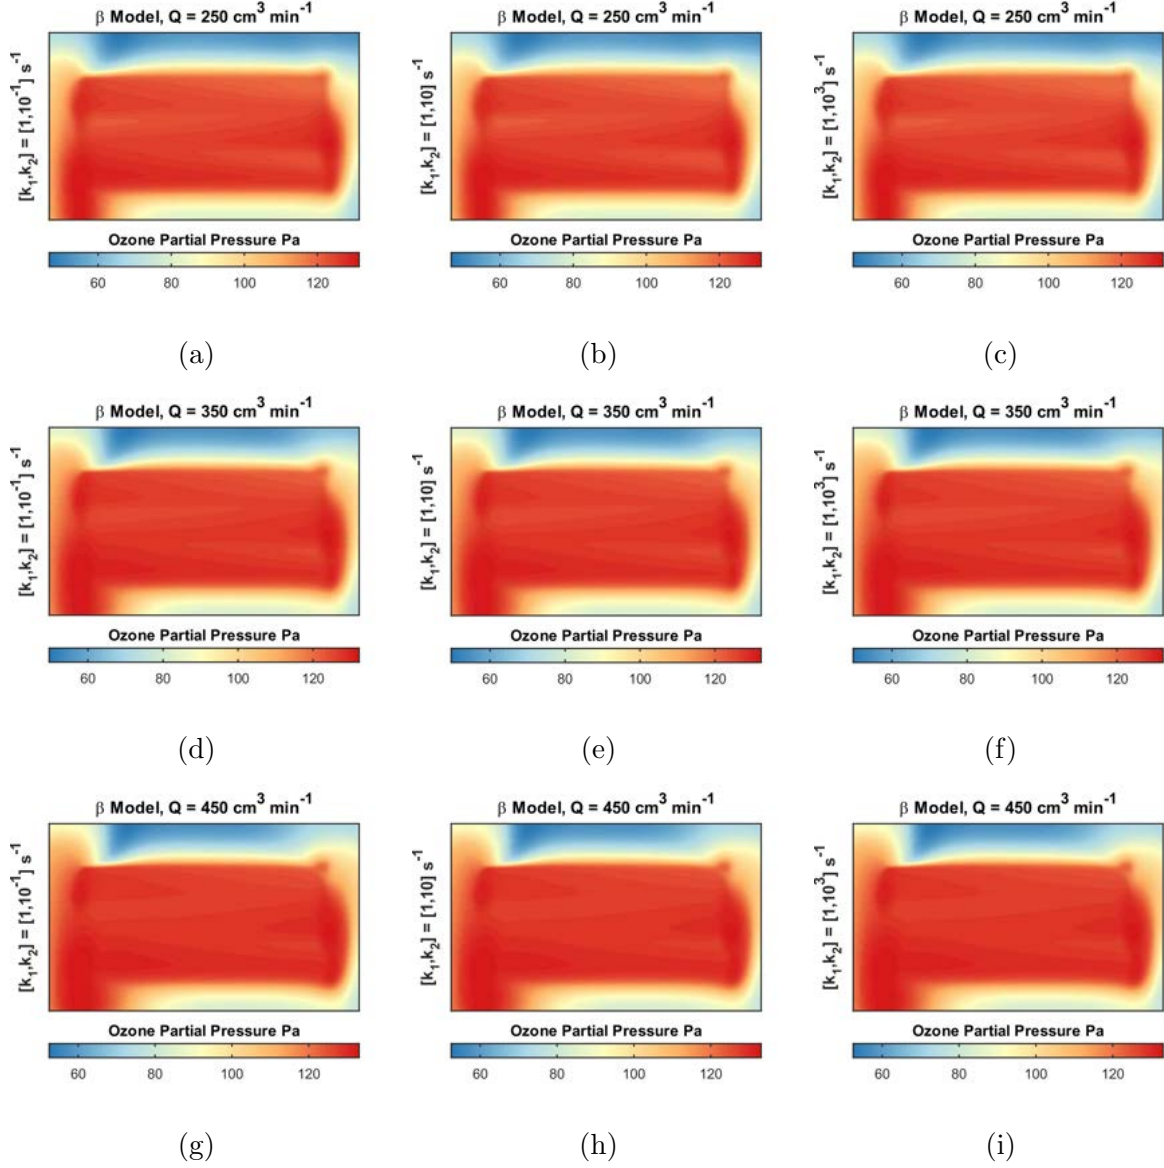

FIG. S30: Normalized ozone partial pressure surfaces for  $k_1 = 1 \text{ s}^{-1}$ , with  $Q = 250$  (top row), 350 (middle row), and  $Q = 450 \text{ cm}^3 \text{min}^{-1}$  (bottom row); and  $k_2 = 10^{-1}$  (left column), 10 (central column), and  $10^3 \text{ s}^{-1}$  (right column).

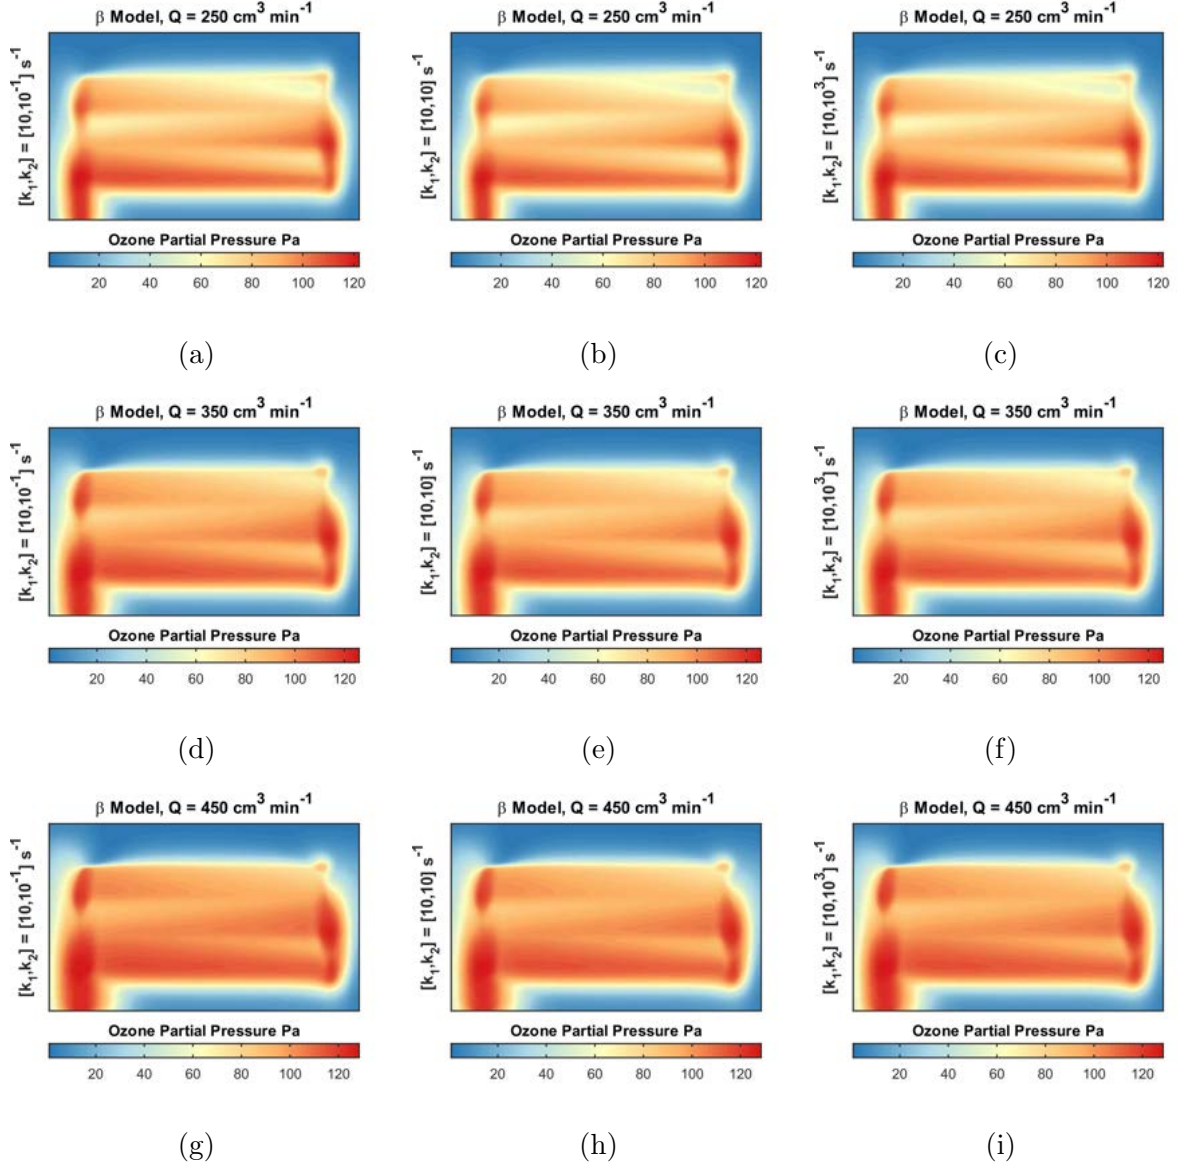

FIG. S31: Normalized ozone partial pressure surfaces for  $k_1 = 10 \text{ s}^{-1}$ , with  $Q = 250$  (top row),  $350$  (middle row), and  $Q = 450 \text{ cm}^3 \text{ min}^{-1}$  (bottom row); and  $k_2 = 10^{-1}$  (left column),  $10$  (central column), and  $10^3 \text{ s}^{-1}$  (right column).

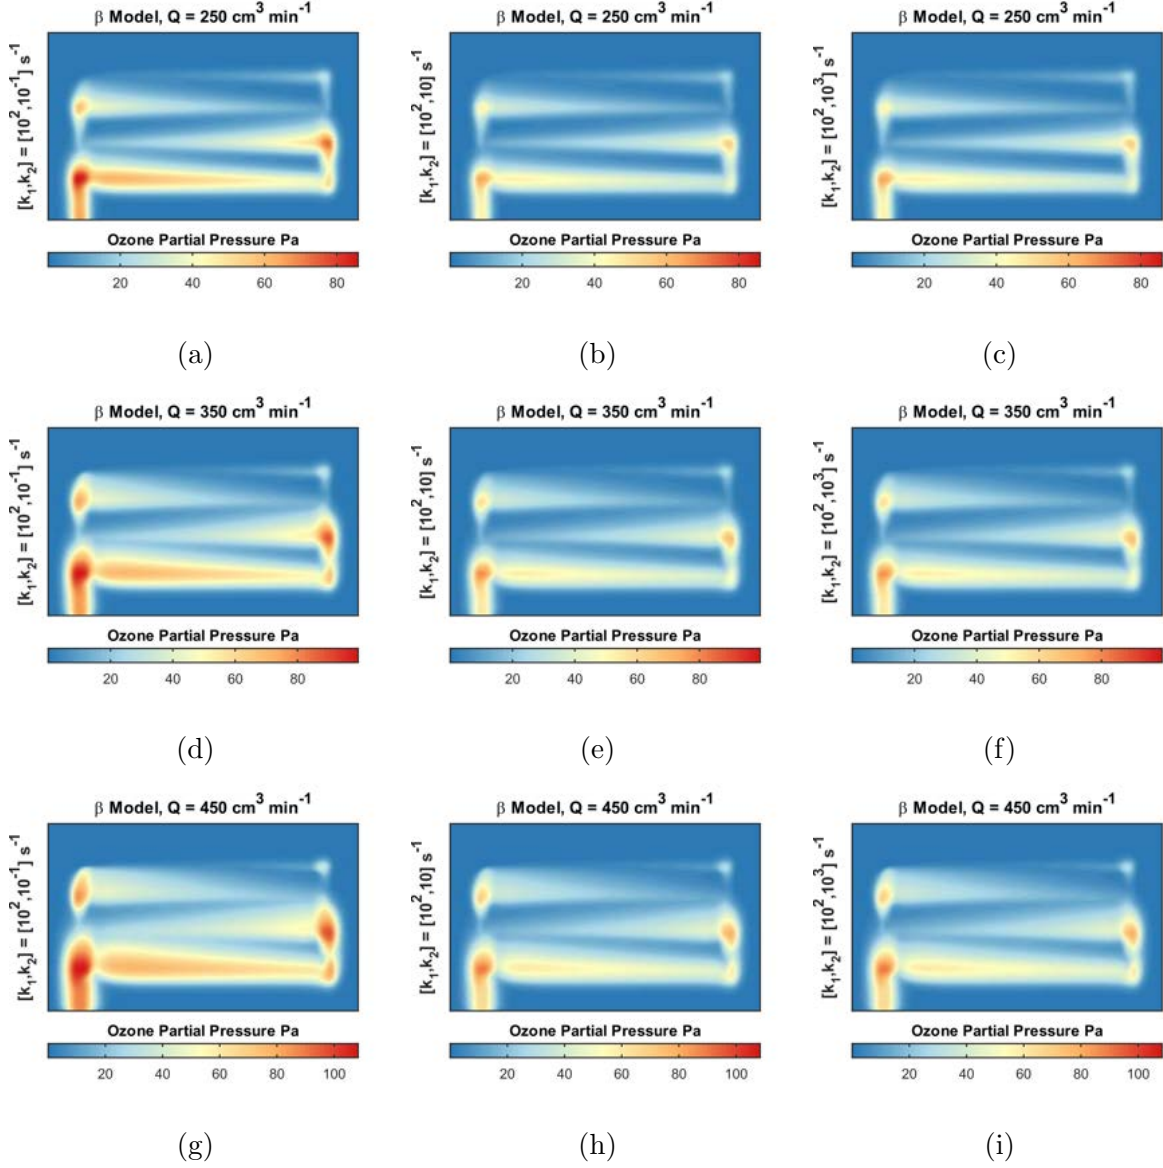

FIG. S32: Normalized ozone partial pressure surfaces for  $k_1 = 10^2 \text{ s}^{-1}$ , with  $Q = 250$  (top row), 350 (middle row), and  $Q = 450 \text{ cm}^3 \text{ min}^{-1}$  (bottom row); and  $k_2 = 10^{-1}$  (left column), 10 (central column), and  $10^3 \text{ s}^{-1}$  (right column).

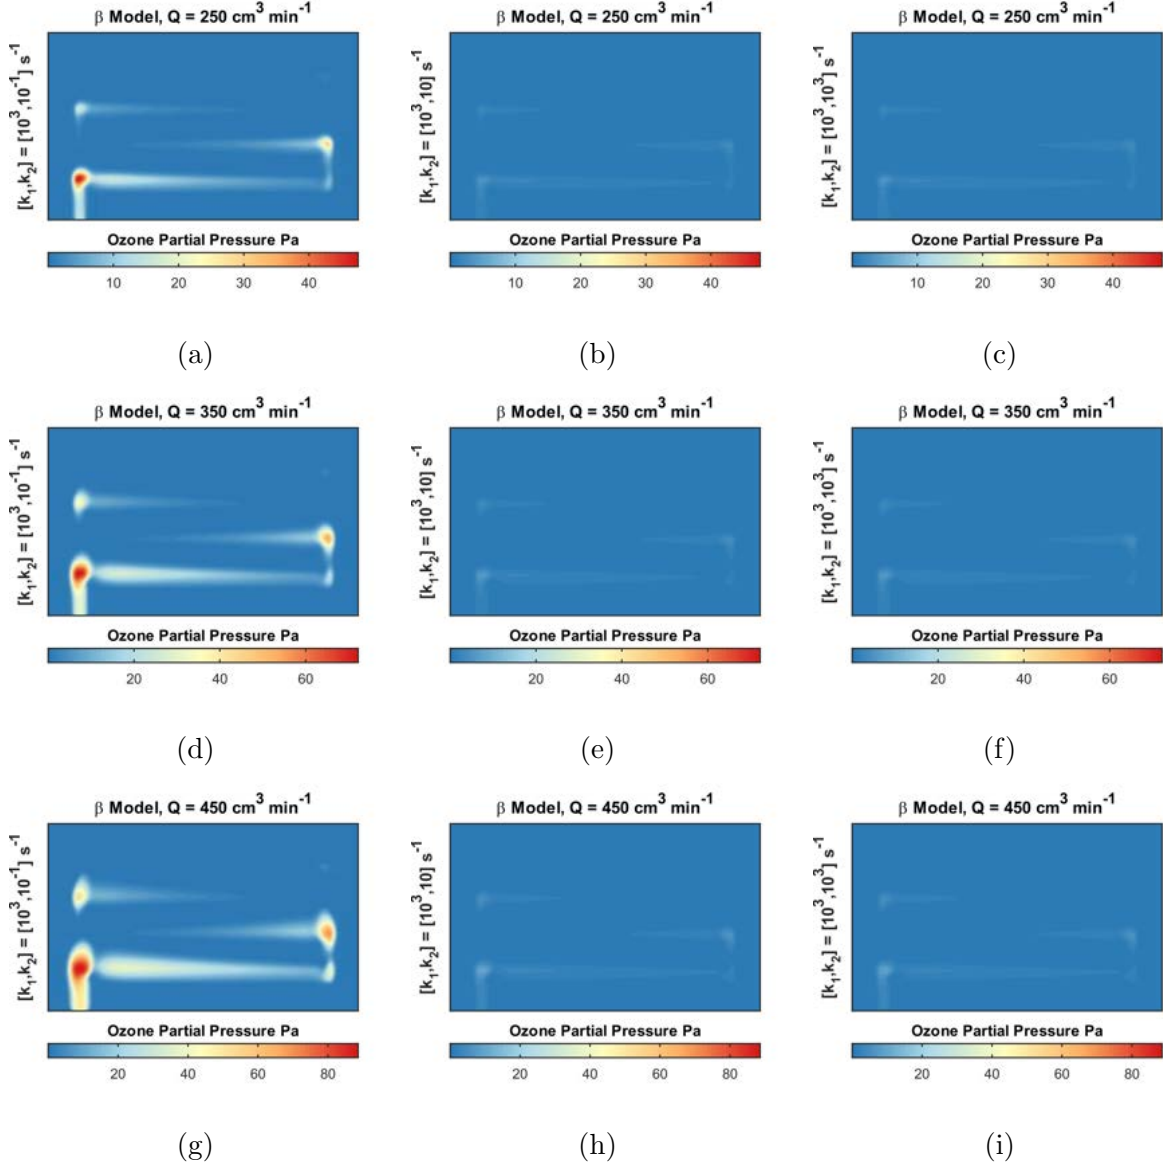

FIG. S33: Normalized ozone partial pressure surfaces for  $k_1 = 10^3 \text{ s}^{-1}$ , with  $Q = 250$  (top row),  $350$  (middle row), and  $Q = 450 \text{ cm}^3 \text{ min}^{-1}$  (bottom row); and  $k_2 = 10^{-1}$  (left column),  $10$  (central column), and  $10^3 \text{ s}^{-1}$  (right column).
