# Supplementary material for: Progress Report on Numerical Modeling of a Prototype Fuel Cell
Source: arXiv:2002.04519 ancillary file (2020-11-13)
Supplement: Supplementary file 2 [file sm_pt2.pdf]

# Progress Report on Numerical Modeling of a Prototype Fuel Cell:

## 2. Grid Convergence Study

### Supplemental Material

Otávio Beruski,<sup>1,\*</sup> Ivan Korkischko,<sup>1,†</sup> Thiago Lopes,<sup>1,‡</sup> and Fabio Coral Fonseca<sup>1,§</sup>

<sup>1</sup>*Instituto de Pesquisas Energéticas e Nucleares,  
IPEN/CNEN-SP, 05508-000, São Paulo, São Paulo, Brazil*

#### SI. INTRODUCTION

This document provides the supplementary information for some decisions, results and discussions made that were deemed secondary to the article. For proper context and discussions, we refer the reader to the paper. The following is presented here. Section SII presents additional information regarding the solvers and meshing procedures used in the models. Section SIII provides additional figures relevant to the grid convergence study, for both the reduced and full geometries used. Section SIV provides additional information on the extrapolation schemes carried for the error estimates, as well as errors estimates for the mesh variant containing so-called “boundary layer” elements (BLEs). Section SV provides figures to support the use of error estimates from the reduced geometry when analyzing the full geometry. Finally, Section SVI provides a brief discretization error assessment for response variables used in the context of Part 1, viz. the  $O_3$  inlet concentration, the normalized apparent reaction rate and  $K'$  ratio, and the real and apparent stoichiometries.

---

\* oberuski@alumni.usp.br

† ivan.korkischko@gmail.com

‡ tlopeschem@gmail.com

§ fabiocf@usp.br

## SII. SOLVERS AND MESHES

### A. Solvers

As mentioned in Section II.A.2 of the paper, the solver configuration used depends on the actual mesh, following a general configuration described in the paper. Here a more complete description is offered, as much as possible, following the hierarchy presented in the software.

The first point concerns the initial values and scaling of the variables to be solved. The initial values were usually the ones described in the paper, sometimes using other solutions as starting point. While some experimentation was done for each mesh case and mesh variant, it was seen that using the initial values always results in numerical convergence. Later on the research it was seen that using coarser meshes as starting point for finer ones reduced computational time and allowed smoother convergence. Independent of the choice, in all cases the scaling was based on the initial values, which generally means using the order of magnitude of each variable's initial value as the scale.

The solver configuration was based on a general configuration, as mentioned, and experimented on as the finer meshes were tested in order to allow reasonable computational resources and convergence smoothness. A parametric solver was always employed for the inlet flow rate, with  $200 \leq Q \leq 450 \text{ cm}^3 \text{ min}^{-1}$ , with a step of  $\delta Q = 50 \text{ cm}^3 \text{ min}^{-1}$ . For the variables, a segregated solver was always used, for the following variables and configurations:

1.  $\theta_{\text{O}_3}$ , using a direct solver with constant damping factor of 1 and update of the Jacobian matrix at every iteration. The termination technique was the number of iterations, being 1.
2.  $P$ ,  $\mathbf{u}$ , and an auxiliary variable for the mass flow inlet boundary condition, using an iterative solver with constant damping factor of 1 and Jacobian update every iteration. Termination technique was the number of iterations, being 1.
3.  $\omega_{\text{O}_3}$ , using either a direct ( $\lambda \leq 4$ ) or an iterative solver ( $\lambda > 4$ ) with constant damping factor 0.7 and Jacobian update every iteration. Termination technique was the number of iterations, being 1.

Step #2 sometimes employed variable damping factor ( $\lambda \geq 12$ ), however a suitable choice for the iterative solver allowed constant damping factor for all  $\lambda$ .

The direct solver used in step #1 was based on the Multifrontal Massively Parallel sparse direct Solver (MUMPS)[1, 2], memory allocation factor 1.2, and automatic pre-ordering algorithm and row pre-ordering turned on. Pivoting was turned on, with a threshold of 0.1. Error estimates were validated automatically, with a factor of 400 in error estimate.

The iterative solver used in step #2 was based on the Generalized Minimal Residual Method (GMRES)[3], with left preconditioning and 50 iterations before restart. A nonlinear-based error norm was used below an error level of 0.1. Error estimates were validated, with a factor of 100 in error estimate and a maximum number of 200 iterations. A geometric multigrid scheme was used as a single pre-conditioner, using a V-cycle and 2 iterations. The hierarchy generation method and number of levels depended on  $\lambda$  and, sometimes, on the mesh variant (BLEs or no-BLEs), and is given in Table S1. The pre- and post-smoother were based on the Symmetrical Coupled Gauss-Siedel (SCGS) scheme, closely resembling Vanka’s Block-Implicit Method [4], with 1 (pre-) or 2 (post-) iterations, relaxation factor of 0.7, and a direct block solver with stored factorization. The scheme is a blocked version, using mesh element lines and vertices, with a vertex relaxation factor of 0.5, and a Vanka-style hybrid subroutine for the auxiliary inlet mass flow variable. Finally, 1 secondary iteration was performed with relaxation factor 0.5. The coarse solver of the multigrid scheme was based on the Parallel sparse Direct Solver (PARDISO)[5], with an automatic scheduling method and a nested dissection multithreaded pre-ordering algorithm. Row pre-ordering and multithreaded forward and backward solve were turned on, and a pivoting perturbation of  $10^{-8}$  was used.

For the last step, #3, the direct solver used for  $\lambda \leq 4$  was the same as step #1, described above, however with a factor of 40 in error estimates. The iterative solver, used for  $\lambda > 4$ , was similar to the one described for step #2, based on GMRES, however with a factor of 40 in error estimate. The single pre-conditioner used, however, was based on the domain decomposition method[6], using a multiplicative Schwarz solver with 1 iteration, maximum of  $2.5 \times 10^5$  degrees of freedom per sub-domain, maximum of 1 node per sub-domain, and additional overlap of 1. Sub-domain coloring was turned on and a coarse level was used, generated by coarsening the mesh and reducing element order by a factor of 2, for  $\lambda \leq 12$  or 3 for  $\lambda = 16$ . The number of sub-domains varied between 4 and 16, however the software increased the number if necessary. Both the coarse and domain solver coupled to this scheme were the same as the solver described in step #1.

TABLE S1: Multigrid details for each mesh

| $\lambda$ | Mesh<br>Variant | Hierarchy<br>Generation Method  | Number of<br>Levels | Mesh<br>Coarsening Factor |
|-----------|-----------------|---------------------------------|---------------------|---------------------------|
| 2         | Both            | Lower element order first (any) | 1                   | 2                         |
| 4         | Both            | Lower element order first (any) | 1                   | 2                         |
| 8         | BLEs            | Coarsen mesh and lower order    | 2                   | 2                         |
|           | No-BLEs         | Lower element order first (any) | 2                   | 3                         |
| 10        | Both            | Manual                          | 2                   | $\lambda = 2, 4$          |
| 12        | Both            | Coarsen mesh and lower order    | 2                   | 2                         |
| 16        | BLEs            | Coarsen mesh and lower order    | 2                   | 4                         |
|           | No-BLEs         |                                 |                     | 2                         |

It should finally be pointed out that, as result of experimentation along the research, optimized solvers were established. One such example is given in Table S1 for  $\lambda = 10$ , where a manual hierarchy for the multigrid was used. In the end of the research, it was noticed that the series of meshes used in the convergence study were perfect for multigrid, and allowed for slightly cheaper and faster convergence. Thus, it was ultimately established for the chosen mesh,  $\lambda = 16$  or  $12$  without BLEs, a two-step solution: firstly by solving a mesh with  $\lambda = 6$  at  $Q = 200 \text{ cm}^3 \text{ min}^{-1}$ , using a multigrid level with  $\lambda = 4$ ; secondly by solving the finer mesh with  $\lambda = 16$  or  $12$ , with the previous step as starting point, using two multigrid levels,  $\lambda = 6, 4$ . Steps #1 to #3 follow the description above.

## B. Meshes

In the paper a brief description of the meshing procedure is given, with the outline of the hierarchy used to generate each mesh as function of  $\lambda$ . Here a more detailed description is given, again as much as possible, in order to minimize dependence on the software. Given the software's terminology, the meshing algorithm was the following:

1. Free tetrahedral node on Ch domain, with isotropic scaling factor of  $\lambda$  and a smoothing subroutine across removed control entities turned on, with number of iterations and maximum element depth of 4. This node has the following sub-nodes:

- (a) Boundary size sub-node, covering all boundaries of the Ch domain with the exception of the inlet and outlet boundaries. Element size parameters were customized: maximum element size  $1.06 \times 10^{-3}$  m, minimum element size  $3.16 \times 10^{-4}$  m, maximum element growth rate 1.15, curvature factor 0.6, and resolution of narrow regions 0.85.
  - (b) Domain size sub-node, covering the Ch domain. Element size parameters were the same as item #1.1.
  - (c) Corner refinement sub-node, covering the Ch domain and all boundaries except the inlet and outlet boundaries. Minimum angle between boundaries 240 deg and element size scaling factor 0.1.
2. Boundary layers node on Ch domain (optional), with corner setting set to *trimming*, minimum angle for trimming 240 deg, maximum angle for trimming 50 deg, and maximum layer decrement 2. The smoothing subroutine was turned on, with maximum number of iterations 4 and maximum element depth 6. This node had the following sub-node:
- (a) Boundary layer properties sub-node, covering all boundaries of the Ch domain except the inlet and outlet boundaries. Number of boundary layers 3, stretching factor 1.2, thickness of the first layer set to automatic, and thickness adjustment factor 1.
3. Copy face node, copying the upper boundary of the Ch domain onto the lower boundary of the MPS domain, specifically the projection of the Ch domain. Copy method was set to automatic, and a smooth subroutine was turned on, with number of iterations and maximum element depth of 4.
4. Free triangular node on the remaining lower MPS boundary, with isotropic scaling factor of 1. Tessellation was set to automatic, with resulting mesh indicating Delaunay tessellation. The smoothing subroutine was turned on, with number of iterations and maximum element depth of 4. This node had the following sub-node:
- (a) Size sub-node, covering the same boundary. Element size parameters were customized: max. element size  $5.85 \times 10^{-4}$  m, min. element size  $6.33 \times 10^{-5}$  m, max.

element growth rate 1.1, curvature factor 0.4, and resolution of narrow regions 0.9.

5. Swept node on the Pm domains (MPS and CL), with the lower MPS boundaries as source, and the upper CL boundary as destination. Face meshing method was quadrilateral; sweep path calculation was set to automatic, likely to be following straight lines; and destination mesh generation set to automatic as well, with no clear difference between methods. Interpolation method for linking faces was set to automatic, with no clear differences between transfinite in 2D or 3D. The smoothing subroutine was turned on, with number of iterations and maximum element depth of 4. This node had the following sub-node:

- (a) Distribution sub-node, covering both Pm domains, using a fixed number of elements of  $\lambda$ .

The same mesh algorithm was used for both reduced and full geometries, the only resulting difference being the number of elements. The total number of domain elements and the average element quality of the resulting meshes can be found in Table S2 and Figure S1 illustrate the resulting meshes in the reduced geometry.

TABLE S2: Properties for each mesh

| $\lambda$ | Mesh Variant | Geometry | Number of Domain Elements | Average Element Quality |
|-----------|--------------|----------|---------------------------|-------------------------|
| 2         | BLEs         | Reduced  | 78134                     | 0.4354                  |
|           |              | Full     | 167762                    | 0.4337                  |
|           | No-BLEs      | Reduced  | 53386                     | 0.6492                  |
|           |              | Full     | 114958                    | 0.6510                  |
| 4         | BLEs         | Reduced  | 279404                    | 0.4291                  |
|           |              | Full     | 646357                    | 0.4392                  |
|           | No-BLEs      | Reduced  | 219820                    | 0.5993                  |
|           |              | Full     | 510543                    | 0.6034                  |
| 8         | BLEs         | Reduced  | 1415349                   | 0.4728                  |
|           |              | Full     | 3296631                   | 0.4728                  |
|           | No-BLEs      | Reduced  | 1230431                   | 0.5834                  |
|           |              | Full     | 2874095                   | 0.5833                  |
| 10        | BLEs         | Reduced  | 2564273                   | 0.4886                  |
|           |              | Full     | —                         | —                       |
|           | No-BLEs      | Reduced  | 2284191                   | 0.5845                  |
|           |              | Full     | —                         | —                       |
| 12        | BLEs         | Reduced  | 4170282                   | 0.5014                  |
|           |              | Full     | 9772477                   | 0.5013                  |
|           | No-BLEs      | Reduced  | 3773525                   | 0.5887                  |
|           |              | Full     | 8864112                   | 0.5872                  |
| 16        | BLEs         | Reduced  | 9138557                   | 0.5100                  |
|           |              | Full     | —                         | —                       |
|           | No-BLEs      | Full     | 8448731                   | 0.5964                  |
|           |              | Full     | —                         | —                       |

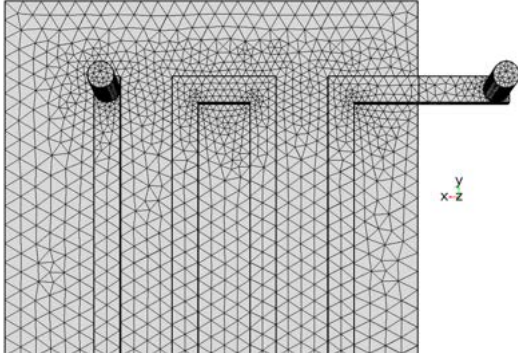

(a)

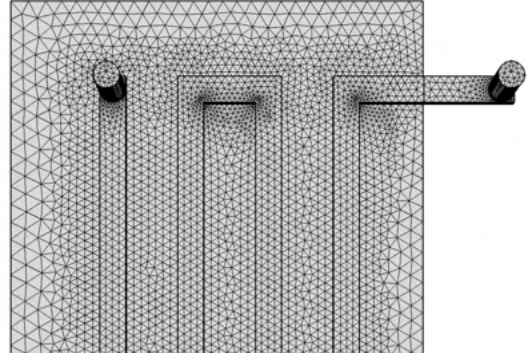

(b)

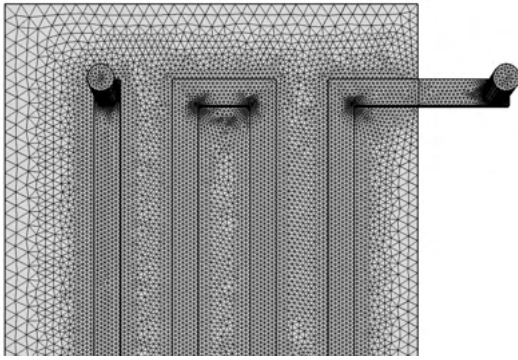

(c)

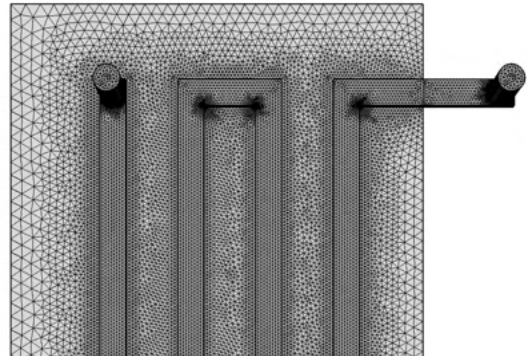

(d)

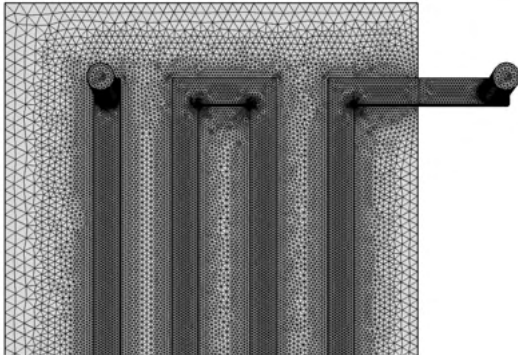

(e)

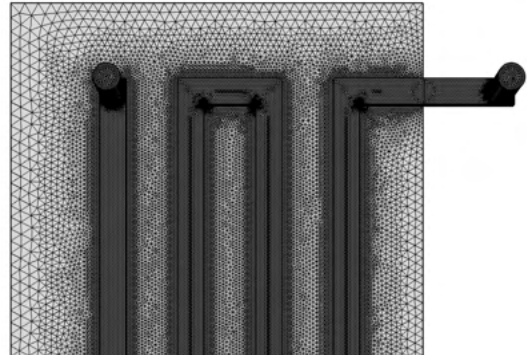

(f)

FIG. S1: Snapshots of the meshes resulting from the meshing procedures outlined in the text for the reduced geometry: (a)  $\lambda = 2$ , (b) 4, (c) 8, (d) 10, (e) 12, and (f) 16.

### SIII. MESH CONVERGENCE STUDY

This section provides additional plots on the qualitative analysis of the mesh convergence study carried in Section III.A, as well as for brief digressions to investigate relevant phenomena.

#### A. Reduced Geometry

Here are provided the additional information for the reduced geometry. Figure S2 shows the individual scalar variables, namely  $\Delta\chi_{\text{O}_3}$ ,  $R'_{\text{O}_3}$ , and  $\Delta P$ . Figure S3 shows selected values of  $\lambda$  for better comparison between mesh variants. And Figure S4 shows the dependence of different functionals of ozone molar flux on the effective normalized element spacing.

#### B. Full Geometry

Here are provided the additional information for the full geometry, including the results for the BLEs mesh variant, not shown in the paper. Figure S5 shows the individual scalar variables, namely  $\Delta\chi_{\text{O}_3}$ ,  $R'_{\text{O}_3}$ , and  $\Delta P$  for the no-BLEs mesh variant, while Figure S6 shows the  $\Delta\chi_{\text{O}_3}/R'_{\text{O}_3}$  and  $\Delta P/P_{\text{in}}$  ratios in addition to the individual variables for the BLEs mesh variant. Figures S7 and S8 show the  $U$   $x$  and  $z$  profiles for the no-BLEs and BLEs mesh variants, respectively. Figures S9 and S10 show the  $P_{\text{O}_3}$  profiles along the CL upper boundary for the no-BLEs and BLEs mesh variants, respectively, and compares with the respective reduced geometry case. Finally, Figures S11 and S12 present the  $\mathbf{P}_{\text{O}_3}$  surfaces for the no-BLEs and BLEs mesh variant, respectively.

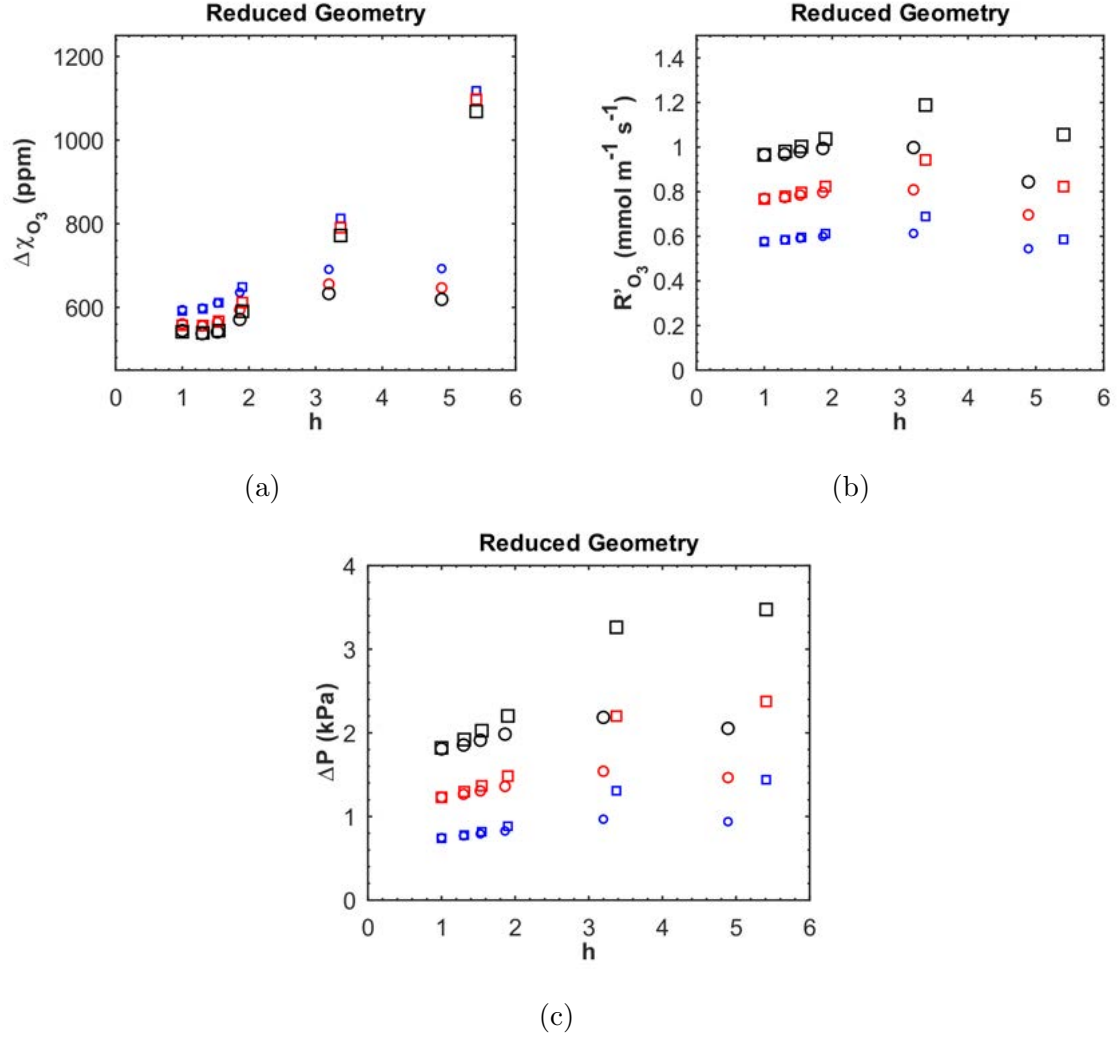

FIG. S2: Scalar response variables as a function of the normalized effective element spacing, obtained at the reduced geometry: **(a)**  $\Delta\chi_{O_3}$ , **(b)**  $R'_{O_3}$ , and **(c)**  $\Delta P$ . The following values of inlet flow rate  $Q$  are shown, with markers increasing in size with  $Q$ : 250, 350 and 450  $\text{cm}^3 \text{min}^{-1}$ . Both mesh variants are shown: with BLEs ( $\circ$ ) and without ( $\square$ ).

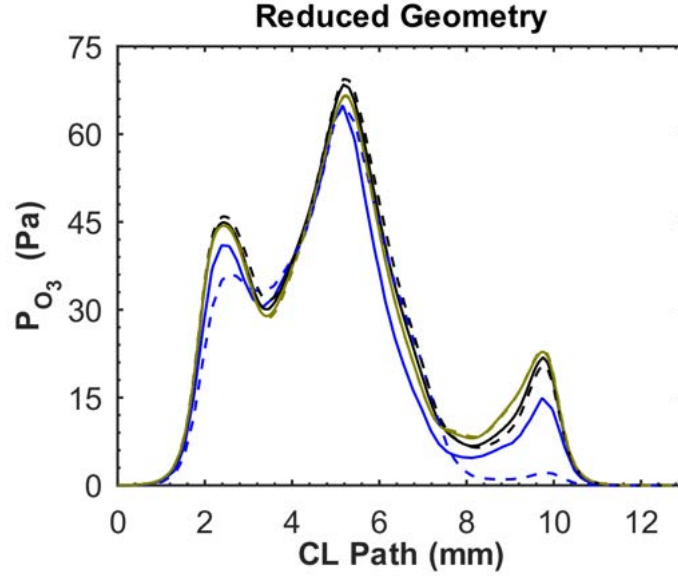

FIG. S3: Ozone partial pressure profiles as function of the path along the CL upper boundary, for inlet flow rate  $Q = 350 \text{ cm}^3 \text{ min}^{-1}$ . Both mesh variants are shown, BLEs (full line) and no-BLEs (dashed line), with the following values of  $\lambda = 2, 8$ , and  $16$ .

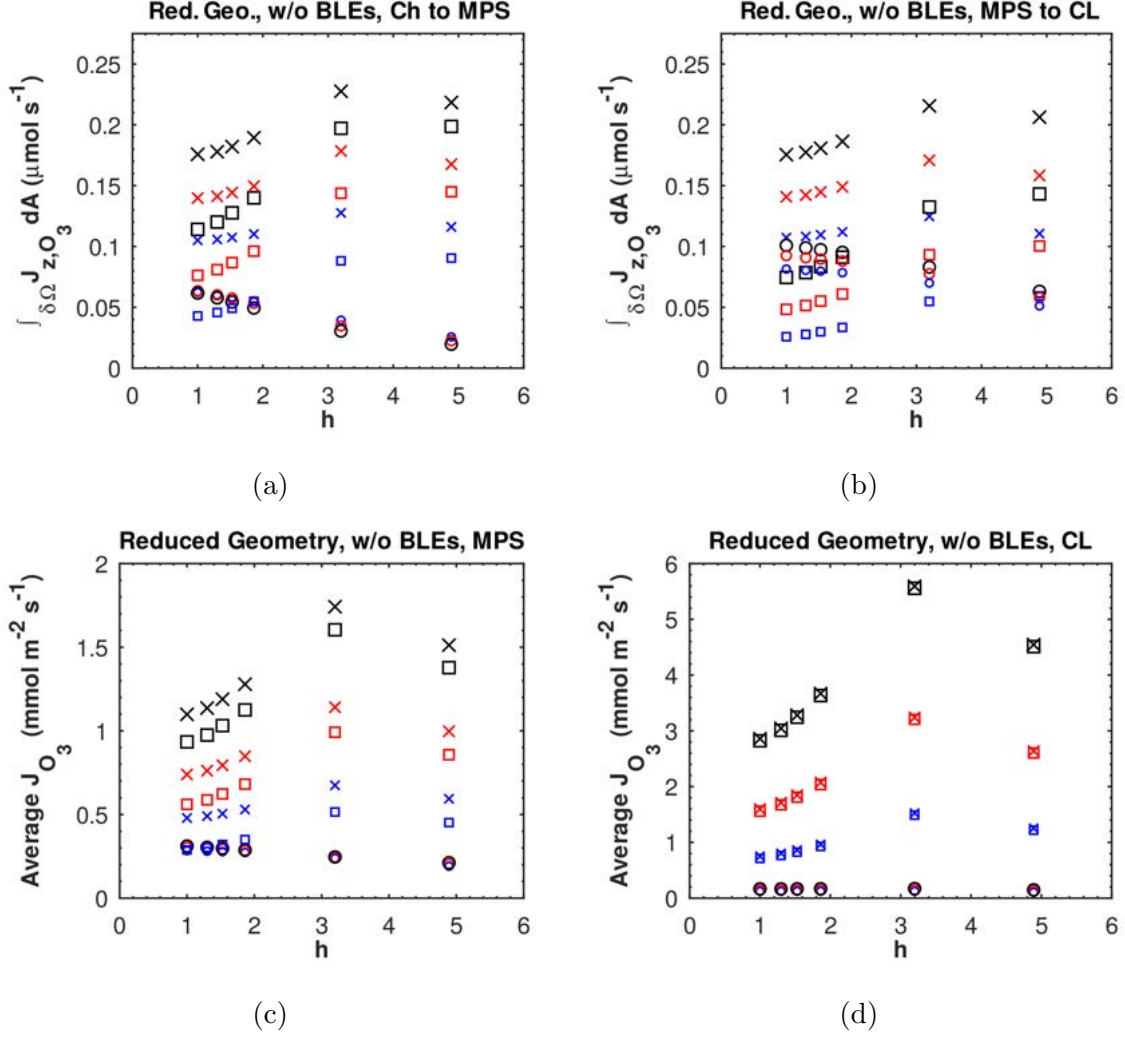

FIG. S4: Contributions to ozone molar flux as function of the normalized effective element spacing for the no-BLEs mesh variant. The following values of inlet flow rate  $Q$  are shown, with marker size increasing with  $Q$ : 250, 350, and 450  $\text{cm}^3 \text{min}^{-1}$ . (a) integrated  $z$  component of the molar flux over the boundary between Ch and MPS domains, and (b) between MPS and CL domains; (c) average magnitude of the molar flux over the MPS and (d) domains. Both diffusive ( $\circ$ ) and convective ( $\square$ ) contributions to the total molar flux are shown.

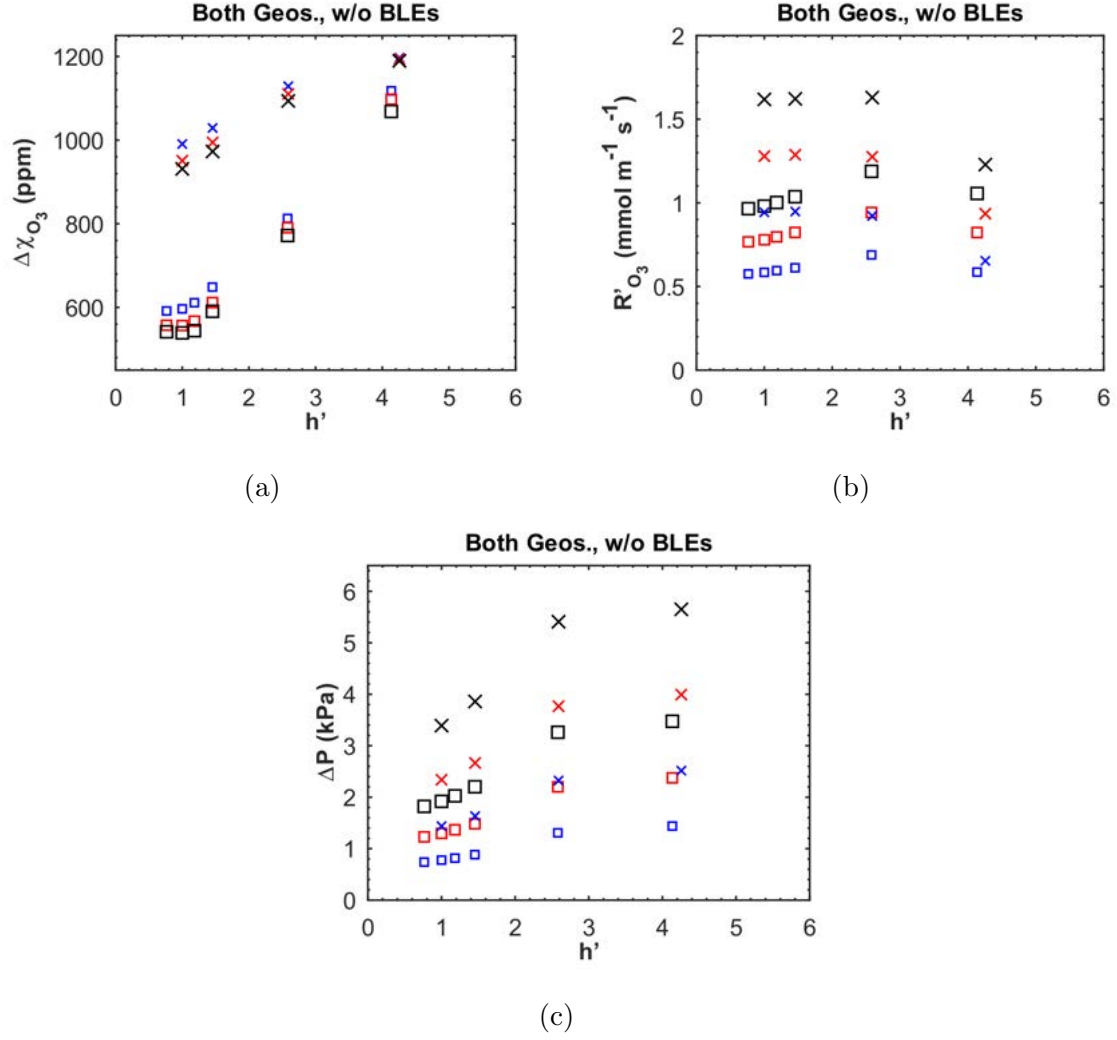

FIG. S5: Scalar response variables as a function of the normalized effective element spacing, obtained for both reduced ( $\square$ ) and full ( $\times$ ) geometries, using the no-BLEs mesh variant. : **(a)**  $\Delta\chi_{O_3}$ , **(b)**  $R'_{O_3}$ , and **(c)**  $\Delta P$ . The following values of inlet flow rate  $Q$  are shown, with markers increasing in size with  $Q$ : 250, 350 and 450  $\text{cm}^3 \text{min}^{-1}$ .

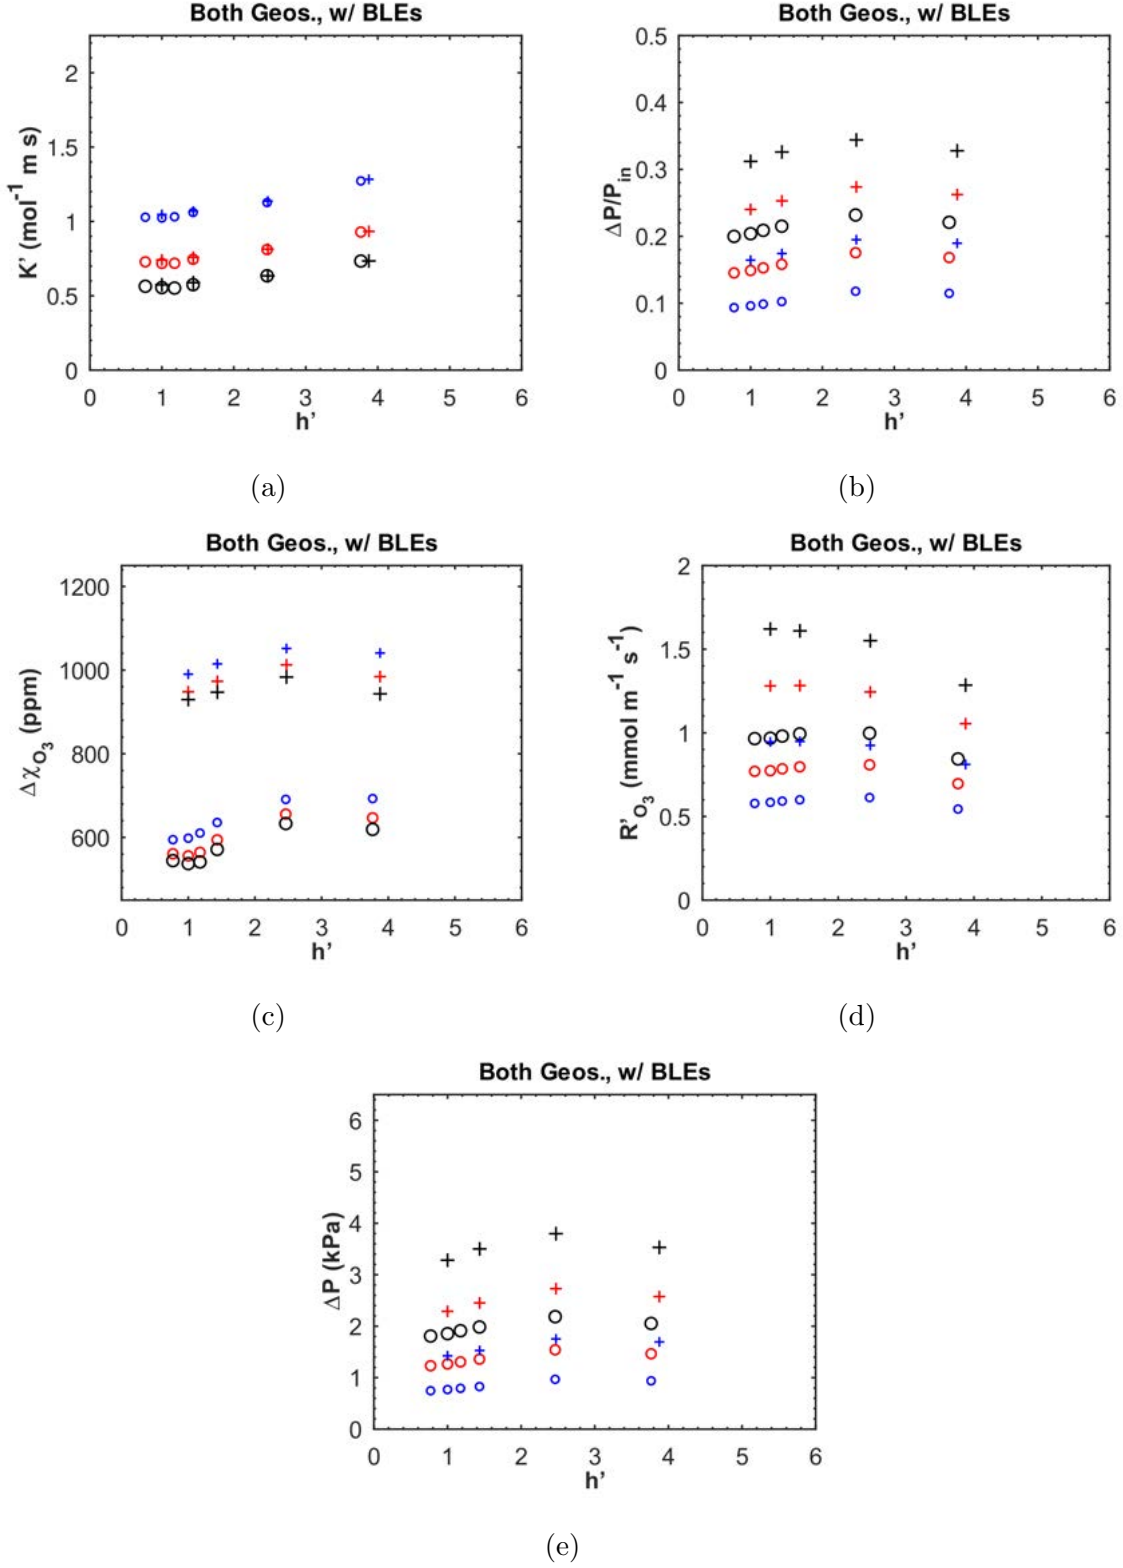

FIG. S6: Scalar response variables as function of the normalized effective element spacing, obtained for both reduced ( $\circ$ ) and full ( $+$ ) geometries, using the BLEs mesh variant: (a)  $K'$ , (b)  $\Delta P/P_{\text{in}}$ , (c)  $\Delta \chi_{\text{O}_3}$ , (d)  $R'_{\text{O}_3}$ , and (e)  $\Delta P$ . The following values  $Q$  are shown, with markers increasing in size with  $Q$ : 250, 350

and 450  $\text{cm}^3 \text{min}^{-1}$ .

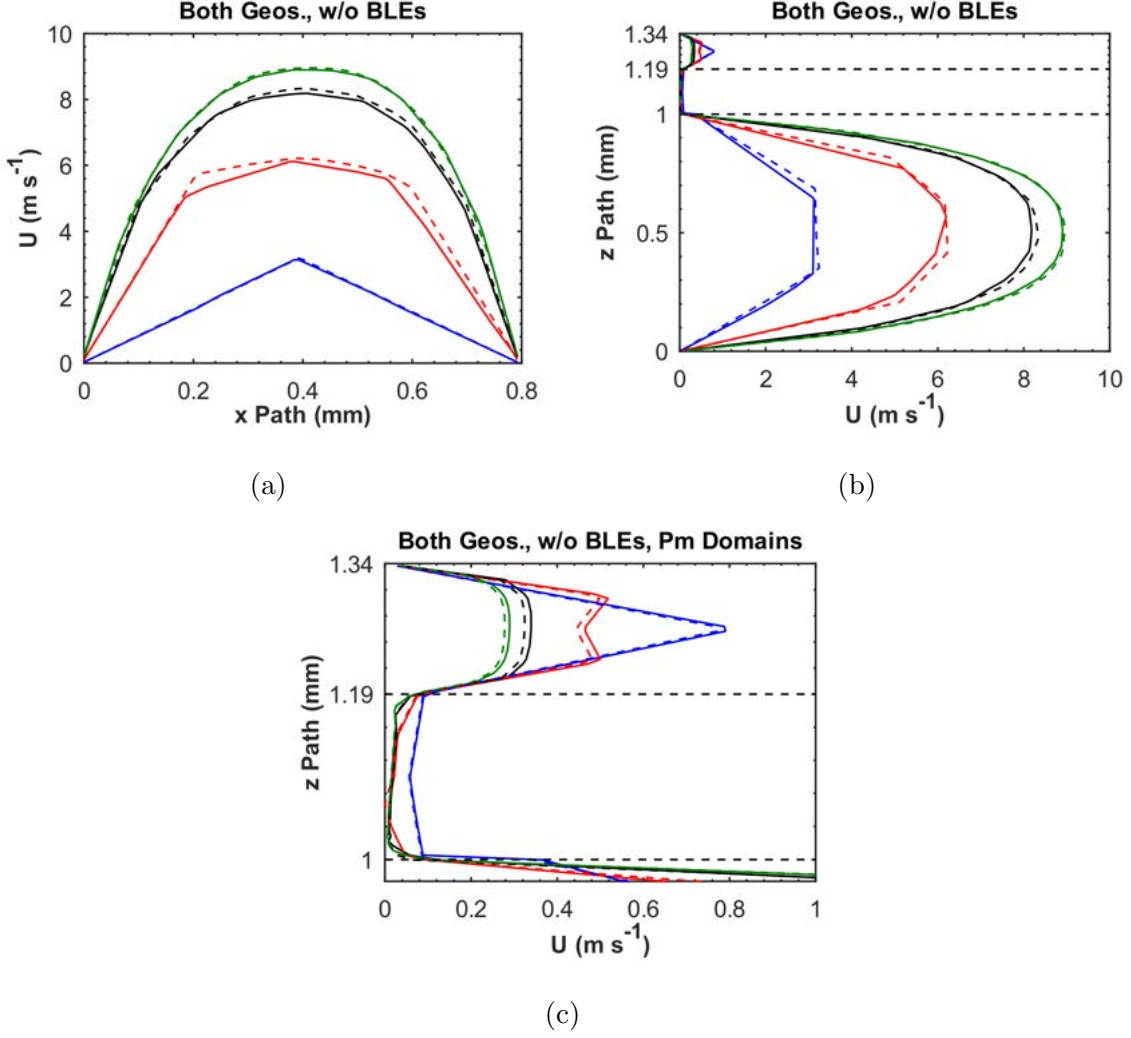

FIG. S7: Flow speed profiles for the reduced (full lines) and full (dashed lines) geometries, using the no-BLEs mesh variant, for  $Q = 350 \text{ cm}^3 \text{ min}^{-1}$ : **(a)** profile along the  $x$  axis, **(b)** along the  $z$  axis, with **(c)** zoom in on the Pm domains. The following values of  $\lambda$  are shown: 2, 4, 8, 12. The dashed horizontal lines indicate the boundaries between domains.

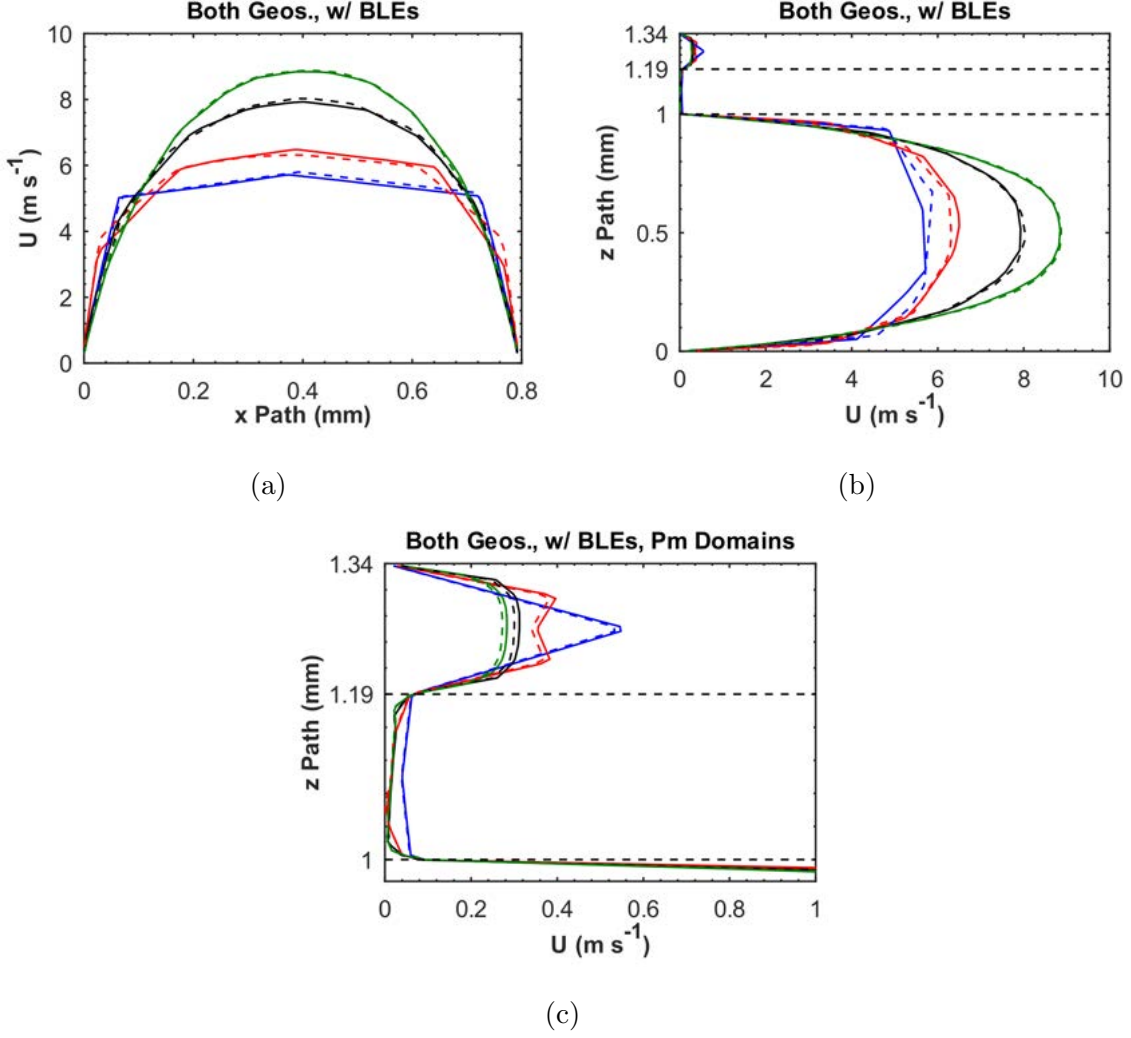

FIG. S8: Flow speed profiles for the reduced (full lines) and full (dashed lines) geometries, using the BLEs mesh variant, for  $Q = 350 \text{ cm}^3 \text{ min}^{-1}$ : **(a)** profile along the  $x$  axis, **(b)** along the  $z$  axis, with **(c)** zoom in on the Pm domains. The following values of  $\lambda$  are shown: 2, 4, 8, 12. The dashed horizontal lines indicate the boundaries between domains.

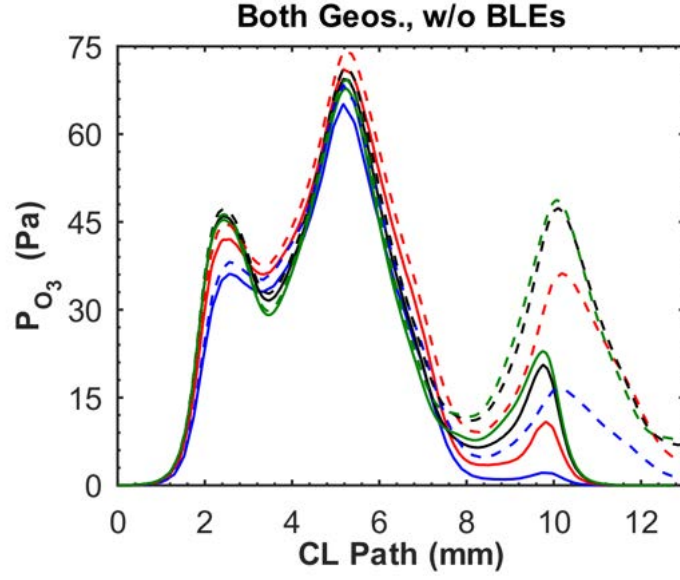

(a)

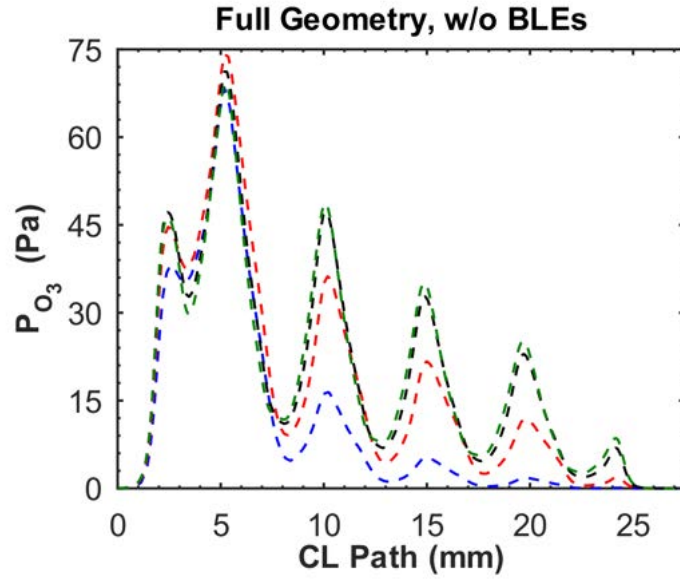

(b)

FIG. S9: Ozone partial pressure profiles for the reduced (full lines) and full (dashed lines) geometries, using the no-BLEs mesh variant, for  $Q = 350 \text{ cm}^3 \text{ min}^{-1}$ : The following values of  $\lambda$  are shown: 2, 4, 8, 12.

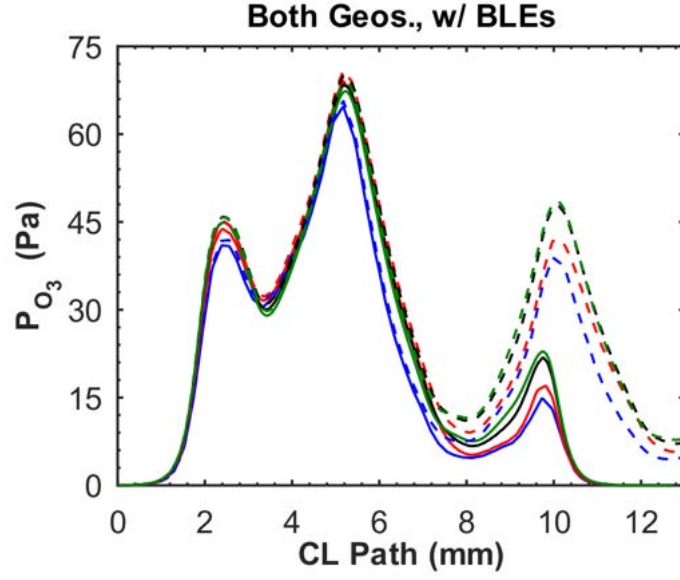

(a)

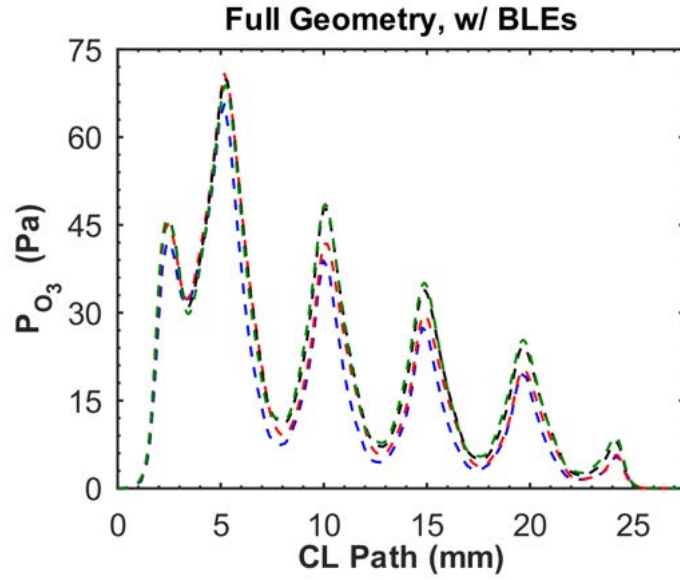

(b)

FIG. S10: Ozone partial pressure profiles for the reduced (full lines) and full (dashed lines) geometries, using the BLEs mesh variant, for  $Q = 350 \text{ cm}^3 \text{ min}^{-1}$ : The following values of  $\lambda$  are shown: 2, 4, 8, 12.

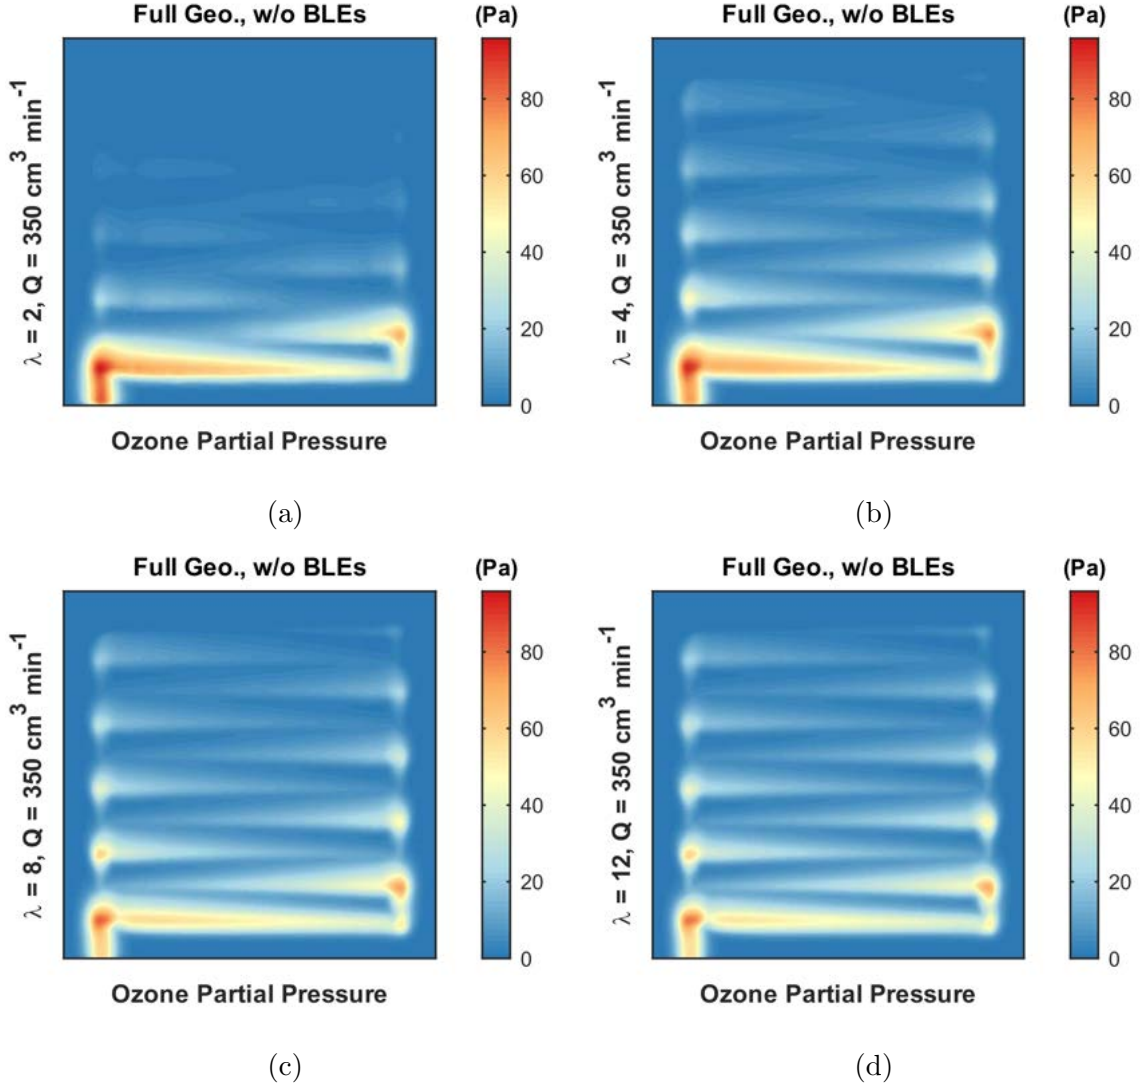

FIG. S11: Ozone partial pressure surfaces obtained at the upper boundary of the CL domain, for inlet flow rate  $Q = 350 \text{ cm}^3 \text{ min}^{-1}$ , using the no-BLEs mesh variant. The following values of  $\lambda$  are shown: (a) 2, (b) 4, (c) 8, and (d) 12.

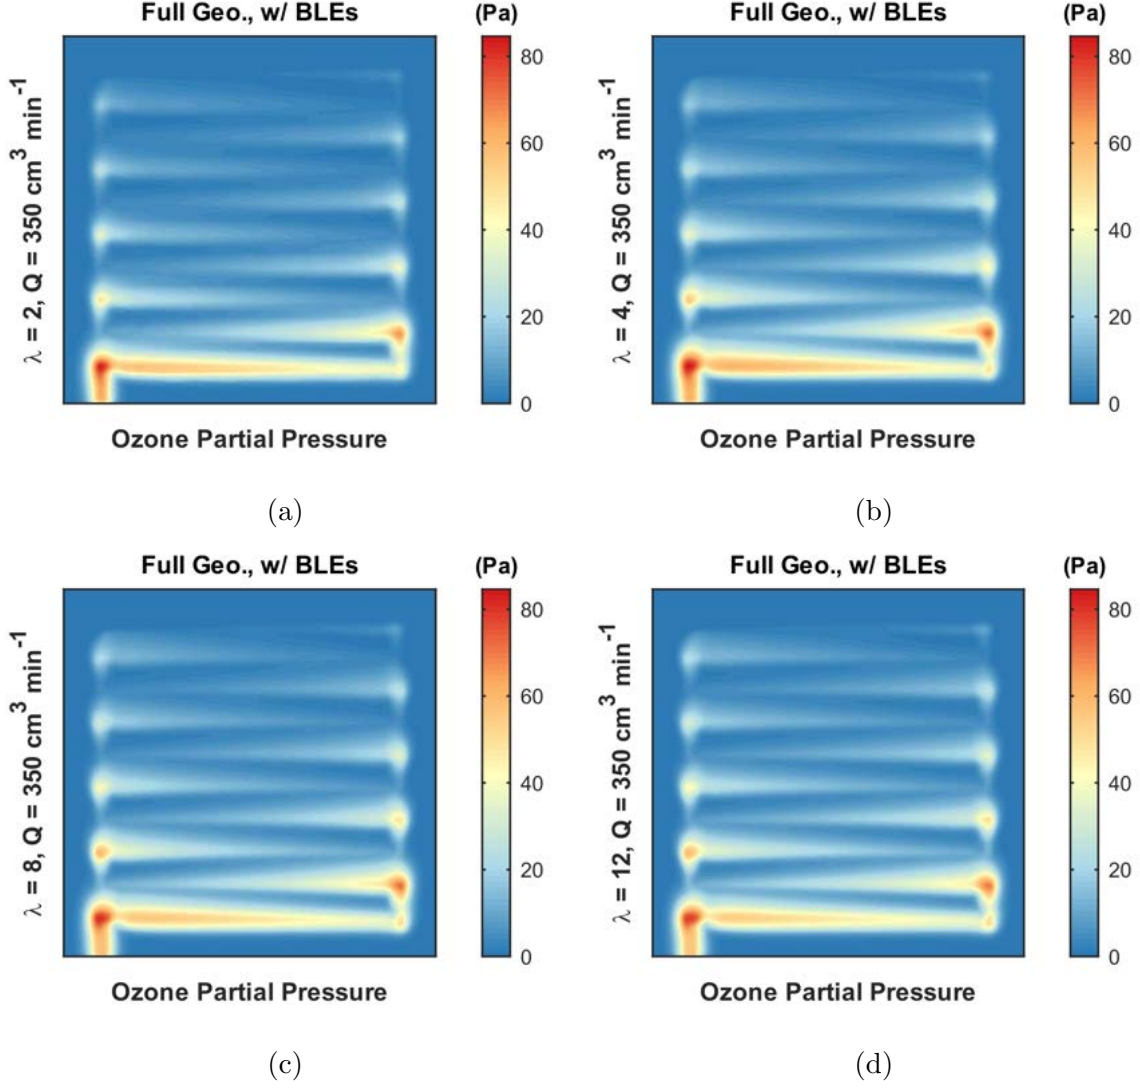

FIG. S12: Ozone partial pressure surfaces obtained at the upper boundary of the CL domain, for inlet flow rate  $Q = 350 \text{ cm}^3 \text{ min}^{-1}$ , using the BLEs mesh variant. The following values of  $\lambda$  are shown: (a) 2, (b) 4, (c) 8, and (d) 12.

## SIV. EXTRAPOLATION SCHEMES AND ERROR ESTIMATES

This section provides additional information on the extrapolation schemes used for the quantitative convergence analysis of Section III.A.3, such as trial mesh sets used and parameters estimated for each extrapolation scheme using both mesh variants. It is also provided the error estimates for the reduced geometry using the BLEs mesh variant.

### A. Tests with Extrapolation Schemes

As mentioned in Section III.A.3 of the paper, tests were carried in order to determine the suitability of each extrapolation scheme and mesh data sets to estimate discretization error. The extrapolation schemes have the following forms:

- Generalized Richardson extrapolation (GRE)[7]:

$$f_k = f_{\text{exact}} + g_p h_k^p + \mathcal{O}(h_k^{p+1}) \quad (1)$$

$$f_{\text{exact}} \approx \bar{f}_R = f_k - g_p h_k^p \quad (2)$$

- Mixed 1st- and 2nd-order extrapolation (MOE-12)[8]:

$$f_k = f_{\text{exact}} + g_1 h_k + g_2 h_k^2 + \mathcal{O}(h_k^3) \quad (3)$$

$$f_{\text{exact}} \approx \bar{f}_M^{(12)} = f_k - g_1 h_k - g_2 h_k^2 \quad (4)$$

- Mixed 1st-, 2nd-, and 3rd- order extrapolation (MOE-123):

$$f_{\text{exact}} \approx \bar{f}_M^{(123)} = f_k - g_1 h_k - g_2 h_k^2 - g_3 h_k^3 \quad (5)$$

With appropriate normalization of  $h$ , the equations can be rewritten in terms of the refinement ratio relative to the finer mesh ( $h_1 = 1$ ). Given the number of parameters, GRE and MOE-12 demand three meshes for estimation of each parameter, while MOE-123 demands four meshes. The GRE and MOE-12 were tested using the following data sets of  $\lambda$ : [8, 12, 16], [4, 10, 16], and [4, 8, 16]. The MOE-123 was tested with the following data sets of  $\lambda$ : [4, 8, 12, 16] and [2, 4, 10, 16]. The sets were chosen in order to abide by the criteria that the refinement ratio  $r_{\text{eff}} > 1.3$  as much as possible. Tables S3 to S5 collect this information

as well as the extrapolation parameters estimated for each variable of interest, i.e. the scalar ratios, for selected values of inlet flow rate and using the no-BLEs mesh variant. Figure S13 compares the extrapolation schemes with the numerical data. Tables S6 to S8 collect the data for the BLEs mesh variant, while Figures S13 and S14 compares the schemes with the numerical data.

## B. Error Estimates

Given the results collected in Tables S3 to S8, and Figures S13 and S14, the mesh data sets considered appropriate were chosen for the use of each extrapolation scheme, as discussed in the paper. Such data sets are highlighted in each table. Afterwards it is discussed the behavior of each scheme with  $h$ , leading to the choice of MOE-12 to estimate the discretization error on the reduced geometry. In addition to the estimates for the no-BLEs mesh variant, already shown in the paper and reproduced here for convenience, it is also given in Table S9 the estimates for the BLEs variant. Figure S15 shows the plots of each scalar variable, as function of  $Q$ , with the error estimates as error bars.

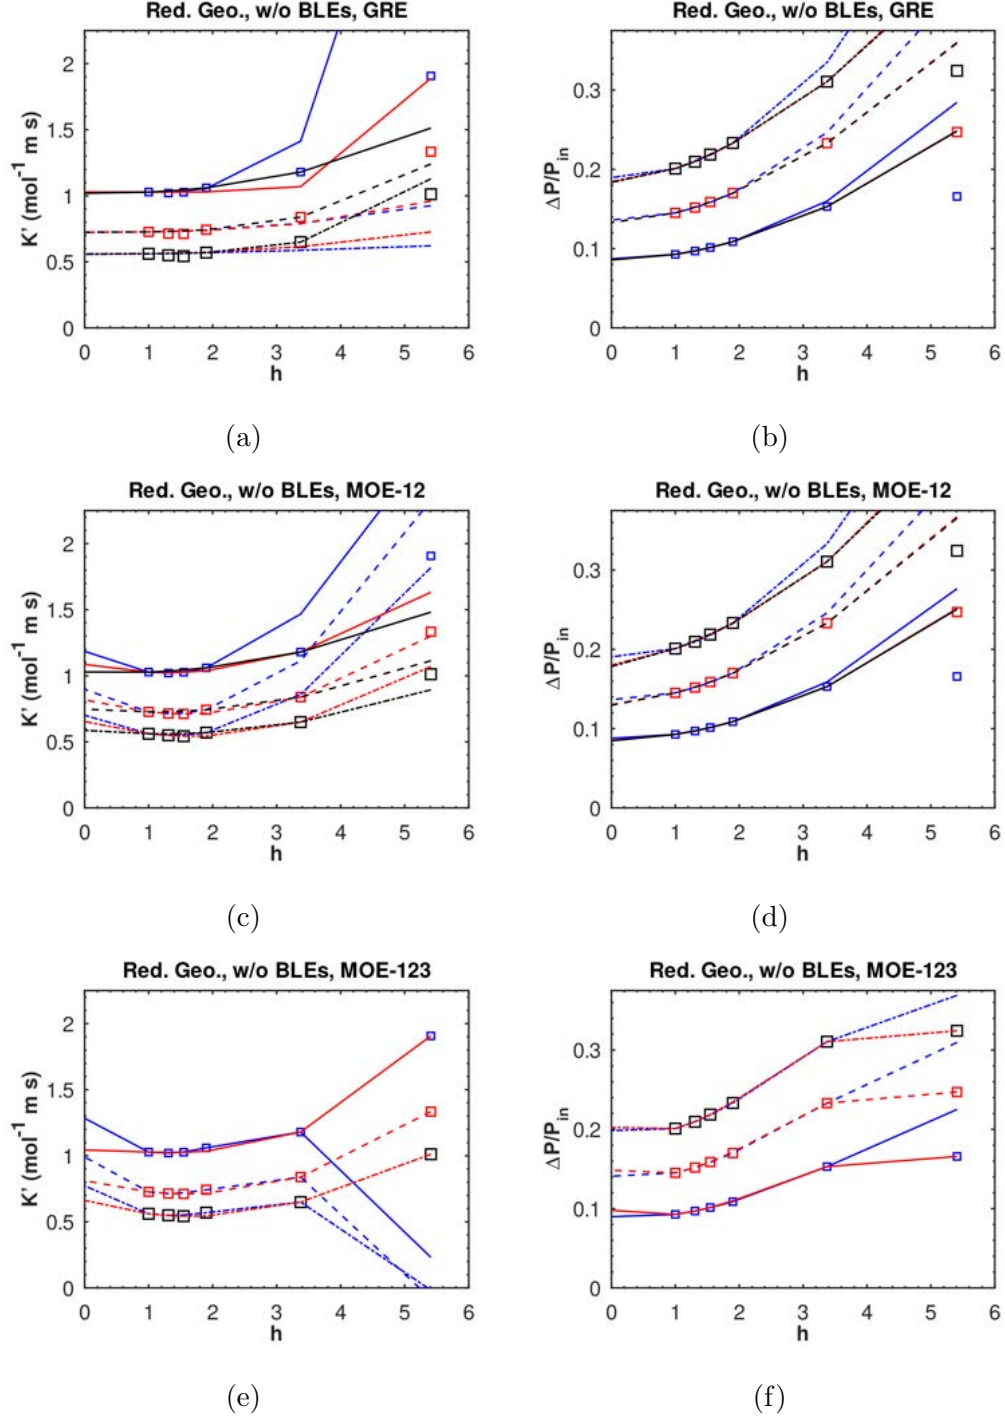

FIG. S13: Comparison between extrapolation schemes (lines) and numerical data ( $\square$ ) as a function of the normalized effective element spacing, obtained for the reduced geometry with the no-BLEs mesh variant: **(left column)**  $K' = \Delta\chi_{O_3}/R'_{O_3}$  and **(right column)**  $\Delta P/P_{in}$ . **(a-b)** GRE, **(c-d)** MOE-12, and **(e-f)** MOE-123. The following values of inlet flow rate  $Q$  are shown, with markers colored and increasing in size with  $Q$ : 250, 350 and 450  $\text{cm}^3 \text{min}^{-1}$ . The extrapolation schemes are coded according to the data sets from Tables S3 to S5 and  $Q$ : [8, 12, 16] (full line), [4, 10, 16] (dashed line), and [4, 8, 16] (dash-dot line).

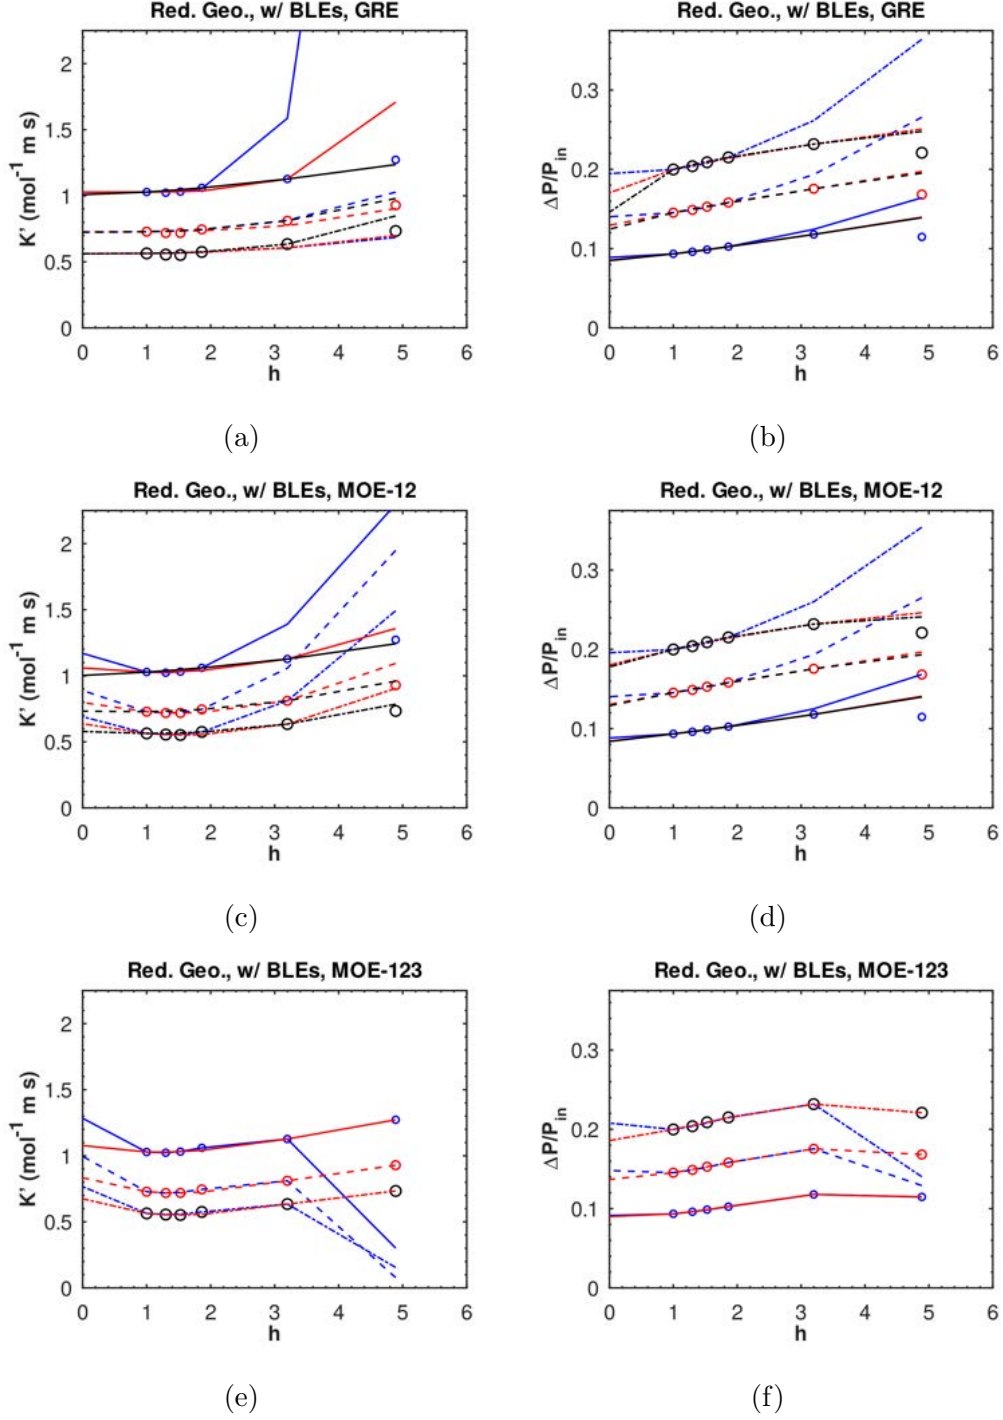

FIG. S14: Comparison between extrapolation schemes (lines) and numerical data (o) as a function of the normalized effective element spacing, obtained for the reduced geometry with the BLEs mesh variant: **(left column)**  $K' = \Delta\chi_{O_3}/R'_{O_3}$  and **(right column)**  $\Delta P/P_{in}$ . **(a-b)** GRE, **(c-d)** MOE-12, and **(e-f)** MOE-123. The following values of inlet flow rate  $Q$  are shown, with markers colored and increasing in size with  $Q$ : 250, 350 and 450  $\text{cm}^3 \text{min}^{-1}$ . The extrapolation schemes are coded according to the data sets from Tables S6 to S8 and  $Q$ : [8, 12, 16] (full line), [4, 10, 16] (dashed line), and [4, 8, 16] (dash-dot line).

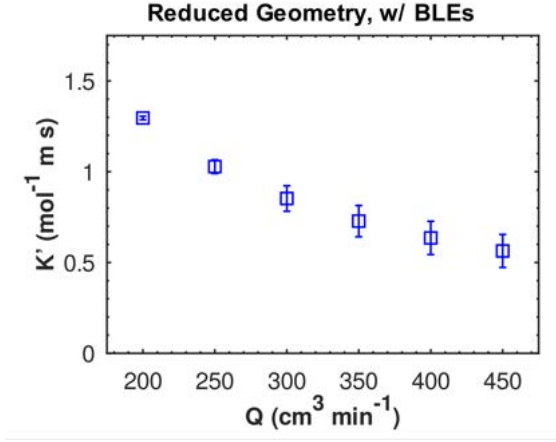

(a)

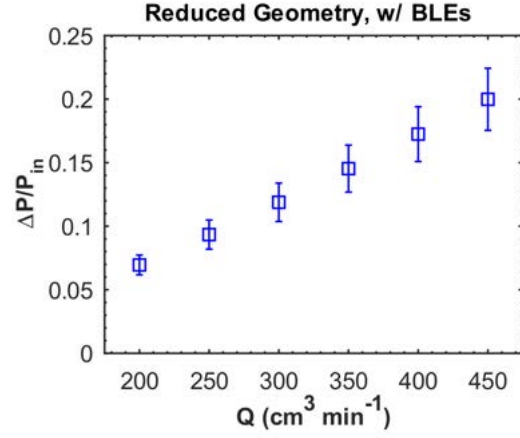

(b)

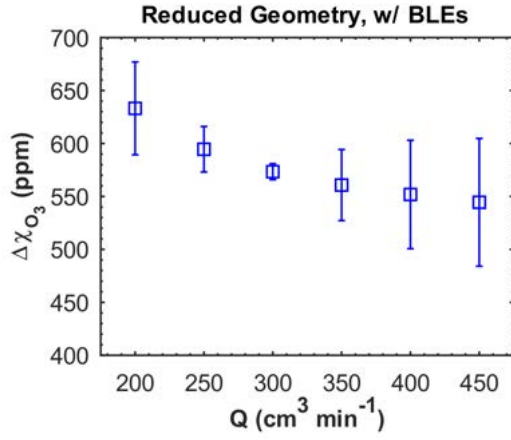

(c)

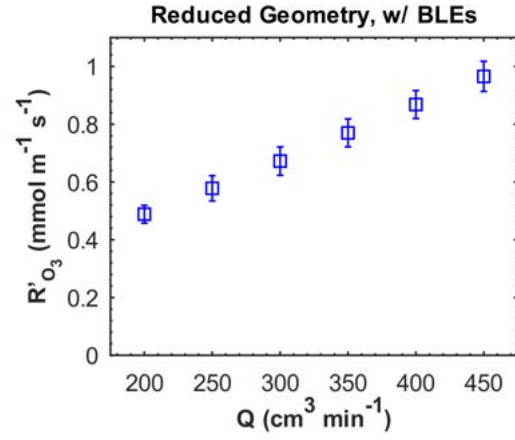

(d)

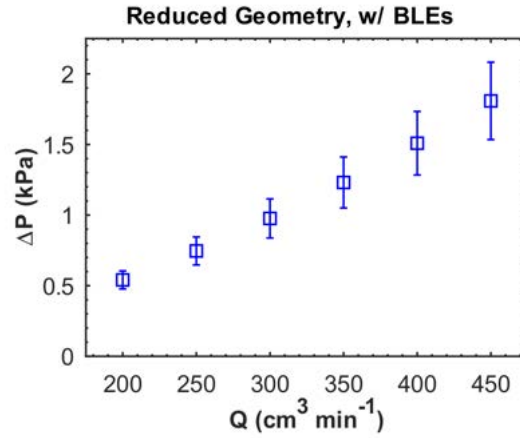

(e)

FIG. S15: Scalar response variables as function of the inlet flow rate using the BLEs mesh variant with the reduced geometry: (a)  $K' = \Delta\chi_{O_3}/R'_{O_3}$ , (b)  $\Delta P/P_{in}$ , (c)  $\Delta\chi_{O_3}$ , (d)  $R'_{O_3}$ , and (e)  $\Delta P$ . Error bars show the estimated discretization error.

TABLE S3: Data sets and parameters for the GRE using the no-BLEs mesh variant

| Data Set    | Variable <sup>a</sup>    | $Q$ (cm <sup>3</sup> min <sup>-1</sup> ) | $g_p$                            | $p$            | $\bar{f}_R^a$                  |
|-------------|--------------------------|------------------------------------------|----------------------------------|----------------|--------------------------------|
| [8, 12, 16] | $K'$                     | 250                                      | $(1.49 - 0.982i) \times 10^{-3}$ | $4.57 - 8.92i$ | $1.03 + 9.82 \times 10^{-4}i$  |
|             |                          | 350                                      | $(4.20 + 0.191i) \times 10^{-3}$ | $2.30 - 9.27i$ | $0.723 - 1.91 \times 10^{-3}i$ |
|             |                          | 450                                      | $(4.34 + 0.172i) \times 10^{-3}$ | $1.60 - 9.41i$ | $0.557 - 1.72 \times 10^{-3}i$ |
|             | $\Delta P/P_{\text{in}}$ | 250                                      | $5.56 \times 10^{-3}$            | 2.11           | $8.72 \times 10^{-2}$          |
|             |                          | 350                                      | $9.09 \times 10^{-3}$            | 2.05           | $13.6 \times 10^{-2}$          |
|             |                          | 450                                      | $11.4 \times 10^{-3}$            | 2.09           | $19.0 \times 10^{-2}$          |
| [4, 10, 16] | $K'$                     | 250                                      | $(1.63 - 5.77i) \times 10^{-5}$  | $6.44 - 4.10i$ | $1.03 + 5.77 \times 10^{-5}i$  |
|             |                          | 350                                      | $(2.21 - 3.28i) \times 10^{-3}$  | $2.76 - 4.38i$ | $0.725 + 3.28 \times 10^{-3}i$ |
|             |                          | 450                                      | $(3.45 - 4.38i) \times 10^{-3}$  | $2.30 - 4.46i$ | $0.558 - 4.38 \times 10^{-3}i$ |
|             | $\Delta P/P_{\text{in}}$ | 250                                      | $6.84 \times 10^{-3}$            | 1.88           | $8.59 \times 10^{-2}$          |
|             |                          | 350                                      | $12.1 \times 10^{-3}$            | 1.74           | $13.3 \times 10^{-2}$          |
|             |                          | 450                                      | $16.5 \times 10^{-3}$            | 1.67           | $18.4 \times 10^{-2}$          |
| [4, 8, 16]  | $K'$                     | 250                                      | $8.91 \times 10^{-3}$            | 2.38           | 1.02                           |
|             |                          | 350                                      | $2.34 \times 10^{-3}$            | 3.20           | 0.724                          |
|             |                          | 450                                      | $0.753 \times 10^{-3}$           | 3.92           | 0.560                          |
|             | $\Delta P/P_{\text{in}}$ | 250                                      | $6.91 \times 10^{-3}$            | 1.87           | $8.58 \times 10^{-2}$          |
|             |                          | 350                                      | $12.2 \times 10^{-3}$            | 1.73           | $13.3 \times 10^{-2}$          |
|             |                          | 450                                      | $17.4 \times 10^{-3}$            | 1.63           | $18.4 \times 10^{-2}$          |

<sup>a</sup> The  $K'$  ratio has units of mol<sup>-1</sup> m s while  $\Delta P/P_{\text{in}}$  is dimensionless.

TABLE S4: Data sets and parameters for the MOE-12 using the no-BLEs mesh variant

| <b>Data Set</b> | <b>Variable<sup>a</sup></b> | <b><math>Q</math> (cm<sup>3</sup> min<sup>-1</sup>)</b> | <b><math>g_1</math></b> | <b><math>g_2</math></b> | <b><math>\bar{f}_M^a</math></b> |
|-----------------|-----------------------------|---------------------------------------------------------|-------------------------|-------------------------|---------------------------------|
| [8, 12, 16]     | $K'$                        | 250                                                     | $-25.8 \times 10^{-2}$  | $10.1 \times 10^{-2}$   | 1.18                            |
|                 |                             | 350                                                     | $-26.8 \times 10^{-2}$  | $9.84 \times 10^{-2}$   | 0.896                           |
|                 |                             | 450                                                     | $-21.8 \times 10^{-2}$  | $7.85 \times 10^{-2}$   | 0.701                           |
|                 | $\Delta P/P_{\text{in}}$    | 250                                                     | $-1.90 \times 10^{-3}$  | $6.80 \times 10^3$      | $8.78 \times 10^{-2}$           |
|                 |                             | 350                                                     | $-1.42 \times 10^3$     | $10.0 \times 10^3$      | $13.7 \times 10^2$              |
|                 |                             | 450                                                     | $-3.12 \times 10^3$     | $13.4 \times 10^3$      | $19.1 \times 10^2$              |
| [4, 10, 16]     | $K'$                        | 250                                                     | $-9.43 \times 10^{-2}$  | $3.59 \times 10^{-2}$   | 1.09                            |
|                 |                             | 350                                                     | $-13.1 \times 10^{-2}$  | $4.08 \times 10^{-2}$   | 0.817                           |
|                 |                             | 450                                                     | $-13.1 \times 10^{-2}$  | $3.84 \times 10^{-2}$   | 0.654                           |
|                 | $\Delta P/P_{\text{in}}$    | 250                                                     | $2.59 \times 10^3$      | $5.21 \times 10^3$      | $8.59 \times 10^2$              |
|                 |                             | 350                                                     | $8.31 \times 10^3$      | $6.56 \times 10^3$      | $13.0 \times 10^2$              |
|                 |                             | 450                                                     | $13.3 \times 10^3$      | $7.52 \times 10^3$      | $18.0 \times 10^2$              |
| [4, 8, 16]      | $K'$                        | 250                                                     | $-1.99 \times 10^{-2}$  | $1.91 \times 10^{-2}$   | 1.03                            |
|                 |                             | 350                                                     | $-4.03 \times 10^{-2}$  | $2.00 \times 10^{-2}$   | 0.747                           |
|                 |                             | 450                                                     | $-4.49 \times 10^{-2}$  | $1.88 \times 10^{-2}$   | 0.587                           |
|                 | $\Delta P/P_{\text{in}}$    | 250                                                     | $2.95 \times 10^3$      | $5.13 \times 10^3$      | $8.46 \times 10^2$              |
|                 |                             | 350                                                     | $9.21 \times 10^3$      | $6.36 \times 10^3$      | $13.0 \times 10^2$              |
|                 |                             | 450                                                     | $15.6 \times 10^3$      | $6.99 \times 10^3$      | $17.8 \times 10^2$              |

<sup>a</sup> The  $K'$  ratio has units of mol<sup>-1</sup> m s while  $\Delta P/P_{\text{in}}$  is dimensionless.

TABLE S5: Data sets and parameters for the MOE-123 using the no-BLEs mesh variant

| Data Set       | Variable <sup>a</sup>    | $Q$ (cm <sup>3</sup> min <sup>-1</sup> ) | $g_1$                  | $g_2$                 | $g_3$                  | $\bar{f}_M^a$         |
|----------------|--------------------------|------------------------------------------|------------------------|-----------------------|------------------------|-----------------------|
| [4, 8, 12, 16] | $K'$                     | 250                                      | -14.4                  | 8.01                  | -1.18                  | 38.3                  |
|                |                          | 350                                      | -14.4                  | 7.70                  | -1.13                  | 29.6                  |
|                |                          | 450                                      | -11.4                  | 5.99                  | -0.865                 | 23.1                  |
|                | $\Delta P/P_{\text{in}}$ | 250                                      | $-6.52 \times 10^{-3}$ | $1.02 \times 10^{-2}$ | $-8.11 \times 10^{-4}$ | $8.99 \times 10^{-2}$ |
|                |                          | 350                                      | $-11.6 \times 10^{-3}$ | $1.75 \times 10^{-2}$ | $-17.8 \times 10^{-4}$ | $14.1 \times 10^{-2}$ |
|                |                          | 450                                      | $-20.9 \times 10^{-3}$ | $2.66 \times 10^{-2}$ | $-31.3 \times 10^{-4}$ | $19.9 \times 10^{-2}$ |
| [2, 4, 10, 16] | $K'$                     | 250                                      | -0.396                 | -0.322                | 0.236                  | 31.2                  |
|                |                          | 350                                      | -3.63                  | 1.05                  | $2.85 \times 10^{-2}$  | 24.3                  |
|                |                          | 450                                      | -4.42                  | 1.45                  | $-5.10 \times 10^{-2}$ | 19.8                  |
|                | $\Delta P/P_{\text{in}}$ | 250                                      | $-2.25 \times 10^{-2}$ | $1.98 \times 10^{-2}$ | $-2.47 \times 10^{-3}$ | $9.79 \times 10^{-2}$ |
|                |                          | 350                                      | $-2.69 \times 10^{-2}$ | $2.71 \times 10^{-2}$ | $-3.47 \times 10^{-3}$ | $14.8 \times 10^{-2}$ |
|                |                          | 450                                      | $-2.99 \times 10^{-2}$ | $3.28 \times 10^{-2}$ | $-4.26 \times 10^{-3}$ | $20.2 \times 10^{-2}$ |

<sup>a</sup> The  $K'$  ratio has units of mol<sup>-1</sup> m s while  $\Delta P/P_{\text{in}}$  is dimensionless.

TABLE S6: Data sets and parameters for the GRE using the BLEs mesh variant

| Data Set    | Variable <sup>a</sup>    | $Q$ (cm <sup>3</sup> min <sup>-1</sup> ) | $g_p$                           | $p$            | $\bar{f}_R^a$                 |
|-------------|--------------------------|------------------------------------------|---------------------------------|----------------|-------------------------------|
| [8, 12, 16] | $K'$                     | 250                                      | $(2.40 + 1.70i) \times 10^{-2}$ | $5.63 + 9.14i$ | $30.7 - 1.70 \times 10^{-2}i$ |
|             |                          | 350                                      | $(9.10 + 4.43i) \times 10^{-2}$ | $2.92 + 9.49i$ | $21.7 - 4.43 \times 10^{-2}i$ |
|             |                          | 450                                      | $(8.65 + 3.84i) \times 10^{-2}$ | $2.39 + 9.58i$ | $16.8 - 3.84 \times 10^{-2}i$ |
|             | $\Delta P/P_{\text{in}}$ | 250                                      | $4.49 \times 10^{-3}$           | 1.78           | $8.90 \times 10^{-2}$         |
|             |                          | 350                                      | $5.10 \times 10^{-3}$           | 2.02           | $14.0 \times 10^{-2}$         |
|             |                          | 450                                      | $5.26 \times 10^{-3}$           | 2.19           | $19.5 \times 10^{-2}$         |
| [4, 10, 16] | $K'$                     | 250                                      | $1.55 \times 10^{-2}$           | 4.52           | 30.7                          |
|             |                          | 350                                      | $(3.78 + 5.59i) \times 10^{-2}$ | $3.11 + 4.58i$ | $21.7 - 5.59 \times 10^{-2}i$ |
|             |                          | 450                                      | $(5.94 + 7.72i) \times 10^{-2}$ | $2.67 + 4.65i$ | $16.8 - 7.72 \times 10^{-2}i$ |
|             | $\Delta P/P_{\text{in}}$ | 250                                      | $8.01 \times 10^{-3}$           | 1.21           | $8.55 \times 10^{-2}$         |
|             |                          | 350                                      | $15.9 \times 10^{-3}$           | 0.913          | $12.9 \times 10^{-2}$         |
|             |                          | 450                                      | $29.6 \times 10^{-3}$           | 0.631          | $17.0 \times 10^{-2}$         |
| [4, 8, 16]  | $(K'$                    | 250                                      | $59.7 \times 10^{-2}$           | 1.53           | 30.1                          |
|             |                          | 350                                      | $13.8 \times 10^{-2}$           | 2.53           | 21.6                          |
|             |                          | 450                                      | $5.22 \times 10^{-2}$           | 3.21           | 16.8                          |
|             | $\Delta P/P_{\text{in}}$ | 250                                      | $8.53 \times 10^{-3}$           | 1.16           | $8.50 \times 10^{-2}$         |
|             |                          | 350                                      | $20.9 \times 10^{-3}$           | 0.769          | $12.5 \times 10^{-2}$         |
|             |                          | 450                                      | $54.1 \times 10^{-3}$           | 0.400          | $14.6 \times 10^{-2}$         |

<sup>a</sup> The  $K'$  ratio has units of mol<sup>-1</sup> m s while  $\Delta P/P_{\text{in}}$  is dimensionless.

TABLE S7: Data sets and parameters for the MOE-12 using the BLEs mesh variant

| <b>Data Set</b> | <b>Variable<sup>a</sup></b> | $Q$ (cm <sup>3</sup> min <sup>-1</sup> ) | $g_1$                  | $g_2$                  | $\bar{f}_M^a$         |
|-----------------|-----------------------------|------------------------------------------|------------------------|------------------------|-----------------------|
| [8, 12, 16]     | $K'$                        | 250                                      | -7.08                  | 2.86                   | 34.9                  |
|                 |                             | 350                                      | -7.65                  | 2.89                   | 26.5                  |
|                 |                             | 450                                      | -5.98                  | 2.22                   | 20.6                  |
|                 | $\Delta P/P_{\text{in}}$    | 250                                      | $2.26 \times 10^{-3}$  | $28.9 \times 10^{-4}$  | $8.84 \times 10^{-2}$ |
|                 |                             | 350                                      | $-2.63 \times 10^{-4}$ | $5.28 \times 10^{-3}$  | $14.0 \times 10^{-2}$ |
|                 |                             | 450                                      | $-31.1 \times 10^{-3}$ | $7.27 \times 10^{-3}$  | $19.6 \times 10^{-2}$ |
| [4, 10, 16]     | $K'$                        | 250                                      | -1.60                  | 0.702                  | 31.6                  |
|                 |                             | 350                                      | -3.06                  | 0.996                  | 23.8                  |
|                 |                             | 450                                      | -3.13                  | 0.976                  | 19.0                  |
|                 | $\Delta P/P_{\text{in}}$    | 250                                      | $8.55 \times 10^{-3}$  | $6.19 \times 10^{-4}$  | $8.43 \times 10^{-2}$ |
|                 |                             | 350                                      | $15.1 \times 10^{-2}$  | $-3.34 \times 10^{-4}$ | $13.1 \times 10^{-2}$ |
|                 |                             | 450                                      | $21.1 \times 10^{-2}$  | $-15.7 \times 10^{-4}$ | $18.0 \times 10^{-2}$ |
| [4, 8, 16]      | $K'$                        | 250                                      | 0.592                  | 0.179                  | 29.9                  |
|                 |                             | 350                                      | -0.489                 | 0.385                  | 21.9                  |
|                 |                             | 450                                      | -0.858                 | 0.434                  | 17.3                  |
|                 | $\Delta P/P_{\text{in}}$    | 250                                      | $9.16 \times 10^{-3}$  | $4.74 \times 10^{-4}$  | $8.39 \times 10^{-2}$ |
|                 |                             | 350                                      | $17.3 \times 10^{-3}$  | $-8.41 \times 10^{-4}$ | $12.9 \times 10^{-2}$ |
|                 |                             | 450                                      | $24.4 \times 10^{-3}$  | $-23.5 \times 10^{-4}$ | $17.8 \times 10^{-2}$ |

<sup>a</sup> The  $K'$  ratio has units of mol<sup>-1</sup> m s while  $\Delta P/P_{\text{in}}$  is dimensionless.

TABLE S8: Data sets and parameters for the MOE-123 using the BLEs mesh variant

| Data Set       | Variable <sup>a</sup>    | $Q$ (cm <sup>3</sup> min <sup>-1</sup> ) | $g_1$                  | $g_2$                 | $g_3$                  | $\bar{f}_M^a$         |
|----------------|--------------------------|------------------------------------------|------------------------|-----------------------|------------------------|-----------------------|
| [4, 8, 12, 16] | $K'$                     | 250                                      | -14.9                  | 8.73                  | 01.41                  | 38.3                  |
|                |                          | 350                                      | -15.0                  | 8.37                  | -1.32                  | 29.7                  |
|                |                          | 450                                      | -11.2                  | 6.14                  | -0.942                 | 22.9                  |
|                | $\Delta P/P_{\text{in}}$ | 250                                      | $-4.83 \times 10^{-3}$ | $8.17 \times 10^{-3}$ | $-1.27 \times 10^{-3}$ | $9.14 \times 10^{-2}$ |
|                |                          | 350                                      | $-18.2 \times 10^{-3}$ | $18.7 \times 10^{-3}$ | $-3.22 \times 10^{-3}$ | $14.8 \times 10^{-2}$ |
|                |                          | 450                                      | $-31.4 \times 10^{-3}$ | $28.3 \times 10^{-2}$ | $-5.06 \times 10^{-3}$ | $20.8 \times 10^{-2}$ |
| [2, 4, 10, 16] | $K'$                     | 250                                      | -2.72                  | 1.36                  | -0.116                 | 32.2                  |
|                |                          | 350                                      | -5.20                  | 2.27                  | -0.223                 | 24.9                  |
|                |                          | 450                                      | -5.35                  | 2.29                  | -0.230                 | 20.1                  |
|                | $\Delta P/P_{\text{in}}$ | 250                                      | $-2.78 \times 10^{-3}$ | $7.37 \times 10^{-3}$ | $-1.18 \times 10^{-3}$ | $9.01 \times 10^{-2}$ |
|                |                          | 350                                      | $2.86 \times 10^{-3}$  | $6.98 \times 10^{-3}$ | $-1.28 \times 10^{-3}$ | $13.7 \times 10^{-2}$ |
|                |                          | 450                                      | $10.2 \times 10^{-3}$  | $4.96 \times 10^{-3}$ | $-1.14 \times 10^{-3}$ | $18.6 \times 10^{-2}$ |

<sup>a</sup> The  $K'$  ratio has units of mol<sup>-1</sup> m s while  $\Delta P/P_{\text{in}}$  is dimensionless.

TABLE S9: Error estimates for the reduced geometry using the MOE-12 scheme.

| Variable                                                 | Mesh Variant | Relative Error Estimate (%) |         |      |
|----------------------------------------------------------|--------------|-----------------------------|---------|------|
|                                                          |              | Minimum                     | Maximum | Mean |
| $K'$ (mol <sup>-1</sup> m s)                             | no-BLEs      | 2.25                        | 17.7    | 11.2 |
|                                                          | BLEs         | 0.756                       | 14.3    | 8.35 |
| $\Delta P/P_{\text{in}}$                                 | no-BLEs      | 7.98                        | 14.5    | 12.7 |
|                                                          | BLEs         | 12.3                        | 14.2    | 13.6 |
| $\Delta\chi_{\text{O}_3}$ (ppm)                          | no-BLEs      | 1.02                        | 14.8    | 8.06 |
|                                                          | BLEs         | 1.30                        | 10.2    | 6.14 |
| $R'_{\text{O}_3}$ (mol m <sup>-1</sup> s <sup>-1</sup> ) | no-BLEs      | 4.33                        | 6.61    | 6.01 |
|                                                          | BLEs         | 5.63                        | 8.05    | 6.75 |
| $\Delta P$ (Pa)                                          | no-BLEs      | 7.11                        | 13.8    | 11.9 |
|                                                          | BLEs         | 13.0                        | 17.2    | 15.8 |

## SV. CORRELATION BETWEEN REDUCED AND FULL GEOMETRIES

This section provides additional information to back up the scaling used to (further) estimate the discretization error of the full geometry. Figure S16 shows plots of the scalar variables obtained for the full geometry against respective variables obtained at the reduced geometry. All data was obtained using the no-BLEs mesh variant. Table S10 summarizes the results shown in the paper for minimum, maximum, and mean error for each response variable.

In order to scale up the error, ordinary linear regressions were carried for each variable. The resulting equations are the following:

- $K'$ :  $\bar{f}_{\text{full}} = 2.8315 \times 10^{-2} + 0.99961 f_{\text{red}}$
- $\Delta P/P_{\text{in}}$ :  $\bar{f}_{\text{full}} = 2.9928 \times 10^{-2} + 1.3940 f_{\text{red}}$
- $\Delta\chi_{\text{O}_3}$ :  $\bar{f}_{\text{full}} = 416.37 + 0.95900 f_{\text{red}}$
- $R'_{\text{O}_3}$ :  $\bar{f}_{\text{full}} = -6.4656 \times 10^{-5} + 1.7203 f_{\text{red}}$
- $\Delta P$ :  $\bar{f}_{\text{full}} = 99.007 + 1.7207 f_{\text{red}}$

The linear regressions are shown for their respective variables in Fig. S16.

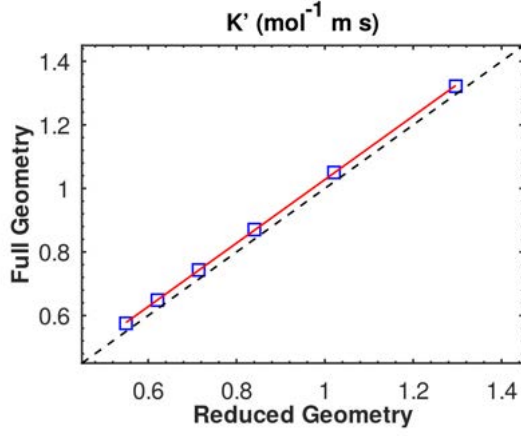

(a)

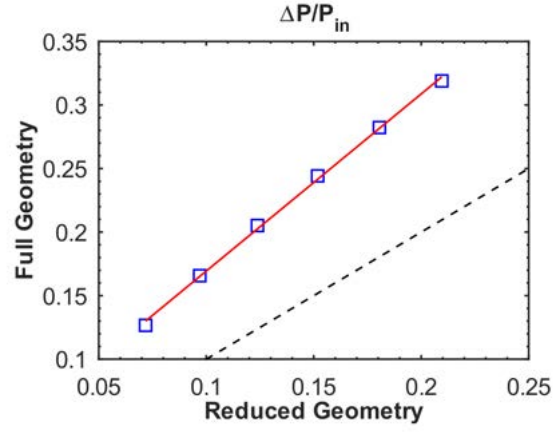

(b)

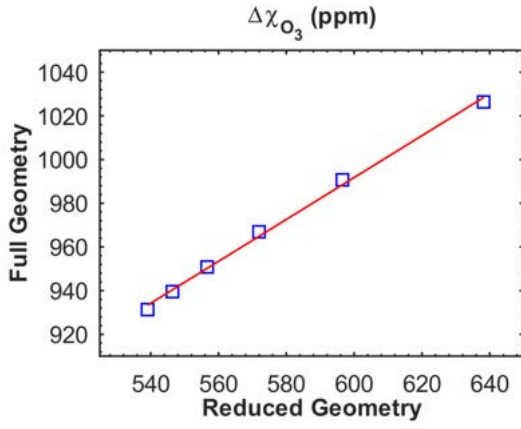

(c)

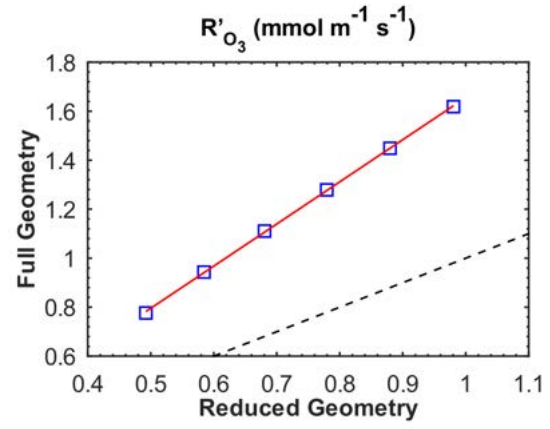

(d)

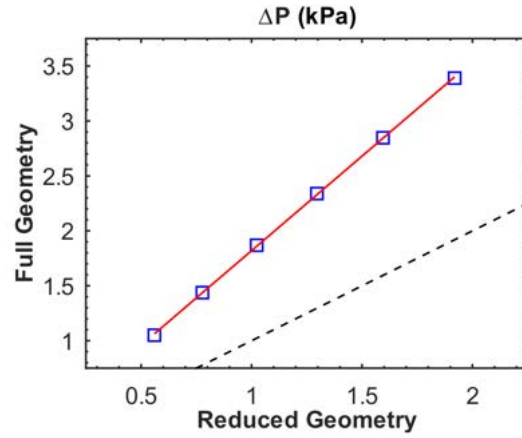

(e)

FIG. S16: Scalar response variables obtained from the full geometry plotted against their respective values obtained from the reduced geometry: (a)  $K' = \Delta\chi_{O_3}/R'_{O_3}$ , (b)  $\Delta P/P_{in}$ , (c)  $\Delta\chi_{O_3}$ , (d)  $R'_{O_3}$ , and (e)  $\Delta P$ . Also shown in each plot is a 1:1 correlation (dashed line) and the linear regression between

TABLE S10: Error estimates for the full geometry using the MOE-12 scheme and the no-BLEs mesh variant.

| Variable                                                 | Relative Error Estimate (%) |         |      |
|----------------------------------------------------------|-----------------------------|---------|------|
|                                                          | Minimum                     | Maximum | Mean |
| $K'$ (mol <sup>-1</sup> m s)                             | 2.14                        | 19.0    | 12.2 |
| $\Delta P/P_{\text{in}}$                                 | 10.2                        | 18.2    | 15.9 |
| $\Delta\chi_{\text{O}_3}$ (ppm)                          | 0.888                       | 9.01    | 4.85 |
| $R'_{\text{O}_3}$ (mol m <sup>-1</sup> s <sup>-1</sup> ) | 6.49                        | 9.37    | 8.54 |
| $\Delta P$ (Pa)                                          | 11.7                        | 20.6    | 17.9 |

## SVI. ERROR ESTIMATE FOR AUXILIARY RESPONSE VARIABLES

As mentioned in Sections II.B.2 and III.C, some additional response variables had their discretization error estimated due to their interest in Part 1 in the context of model comparison. These variables were the  $\text{O}_3$  inlet concentration,  $C_{\text{O}_3,\text{in}}$ ; the normalized apparent reaction rate,  $R'_{\text{O}_3}/C_{\text{O}_3,\text{in}}$  and the related  $K'$  ratio; and the real and apparent stoichiometries, here labeled  $\lambda$  and  $\lambda'$ , respectively, according to the terminology of Part 1.

The auxiliary variables were obtained in accordance with Section II.B of Part 1. Briefly,  $C_{\text{O}_3,\text{in}}$  is the inlet concentration of  $\text{O}_3$ , obtained directly from the model's results. The normalized  $R'_{\text{O}_3}$  is simply the ratio between the apparent reaction rate and the  $\text{O}_3$  inlet concentration,  $R'_{\text{O}_3}/C_{\text{O}_3,\text{in}}$ ; while the normalized  $K'$  follows from its definition, in this case using the normalized  $R'_{\text{O}_3}$ . The real stoichiometry is given by:

$$\lambda = \frac{\dot{n}_{\text{O}_3,\text{in}}}{R_{\text{O}_3}}, \quad (6)$$

where  $\dot{n}_{\text{O}_3,\text{in}} = QC_{\text{O}_3,\text{in}}$  is the inlet molar rate of  $\text{O}_3$  and  $R_{\text{O}_3}$  is the decomposition term integrated over the whole CL domain. Finally, the apparent stoichiometry is defined as:

$$\lambda' = \frac{\Delta\chi_{\text{O}_3}}{\chi_{\text{O}_3,\text{in}}} \quad (7)$$

where  $\chi_{\text{O}_3,\text{in}} = 1200$  ppm is the inlet molar fraction of  $\text{O}_3$ .

The process to estimate the discretization error follows the description of Section II.B.2, regarding the convergence analysis, the extrapolation scheme, and the estimation of the error for the reduced geometry. The further estimate of the discretization error for the full geometry follows the description of Section III.C, correlating the response variables for the reduced and full geometries, and then projecting the error estimated for the reduced geometry to the full one. The linear regressions estimating the scale up between reduced and full geometries are the following:

- $C_{\text{O}_3,\text{in}}$ :  $\bar{f}_{\text{full}} = -3.8350 \times 10^{-2} + 1.7215f_{\text{red}}$
- normalized  $R'_{\text{O}_3}$ :  $\bar{f}_{\text{full}} = -9.3809 \times 10^{-4} + 1.6858f_{\text{red}}$
- normalized  $K'$ :  $\bar{f}_{\text{full}} = 2.0143 \times 10^{-2} + 0.99679f_{\text{red}}$
- $\lambda$ :  $\bar{f}_{\text{full}} = 0.31496 + 0.46649f_{\text{red}}$

- $\lambda'$ :  $\bar{f}_{\text{full}} = 0.51785 + 0.34550f_{\text{red}}$

The results for this Section are shown below. Figure S17 shows the dependency of each auxiliary response variable on the normalized effective element spacing  $h'$ , for both geometries and using the no-BLEs mesh variant. Figure S18 plots the auxiliary response variables obtained for the full geometry against the reduced one. Finally, Figure S19 shows the auxiliary response variables as function of the inlet flow rate  $Q$ , with the estimated discretization errors as error bars for both geometries, using the no-BLEs mesh variant. Table S11 summarizes the relative errors using the MOE-12 scheme for both reduced and full geometries using the no-BLEs mesh variant.

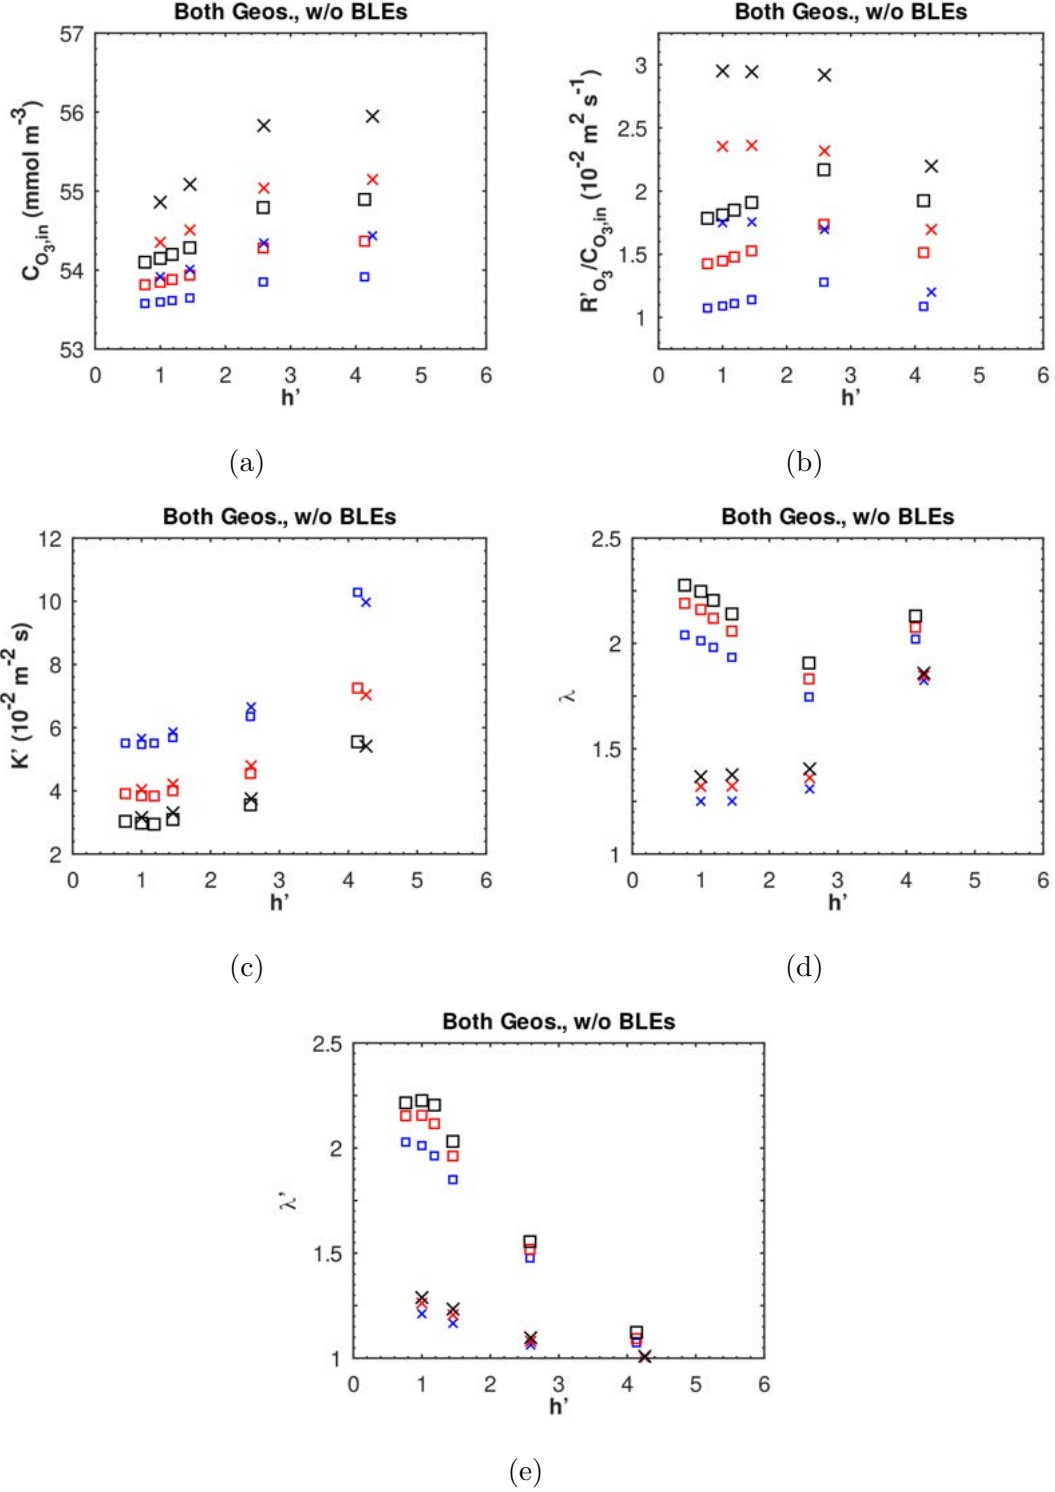

FIG. S17: Auxiliary response variables as a function of the normalized effective element spacing, obtained for both reduced ( $\square$ ) and full ( $\times$ ) geometries, using the no-BLEs mesh variant: (a)  $C_{O_3,in}$ , (b) normalized  $R'_{O_3}$ , (c) normalized  $K'$ , (d) real stoichiometry  $\lambda$ , and (e) apparent stoichiometry  $\lambda'$ . The following values of  $Q$  are shown, with markers increasing in size with  $Q$ : 250, 350 and 450 cm<sup>3</sup> min<sup>-1</sup>.

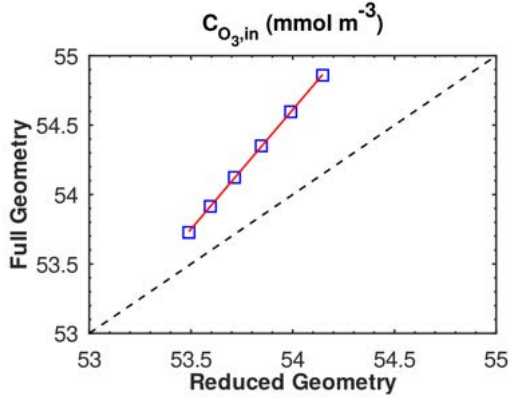

(a)

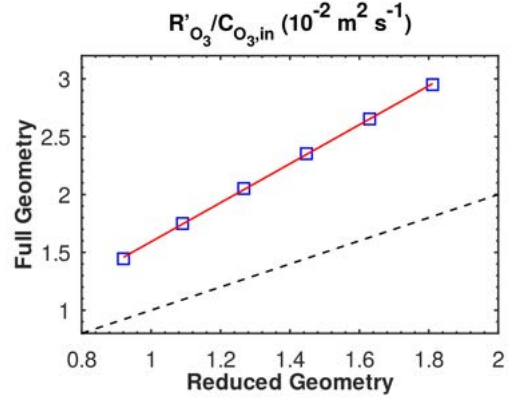

(b)

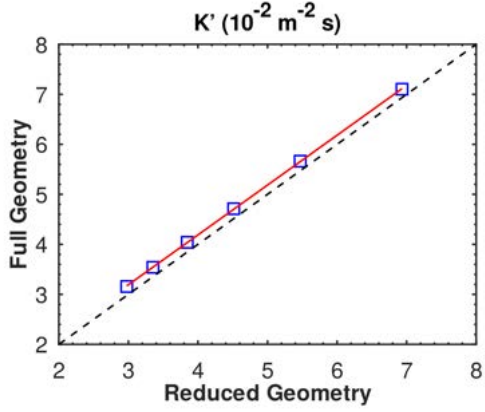

(c)

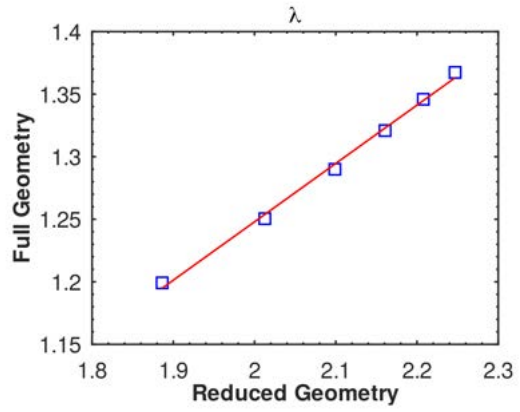

(d)

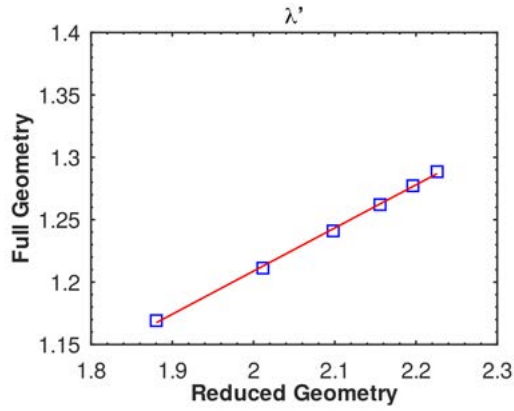

(e)

FIG. S18: Auxiliary response variables obtained from the full geometry plotted against their respective values obtained from the reduced geometry: (a)  $C_{O_3,in}$ , (b) normalized  $R'_{O_3}$ , (c) normalized  $K'$ , (d) real stoichiometry  $\lambda$ , and (e) apparent stoichiometry  $\lambda'$ . Also shown in each plot is a 1:1 correlation (dashed line) and the linear regression between variables (full line).

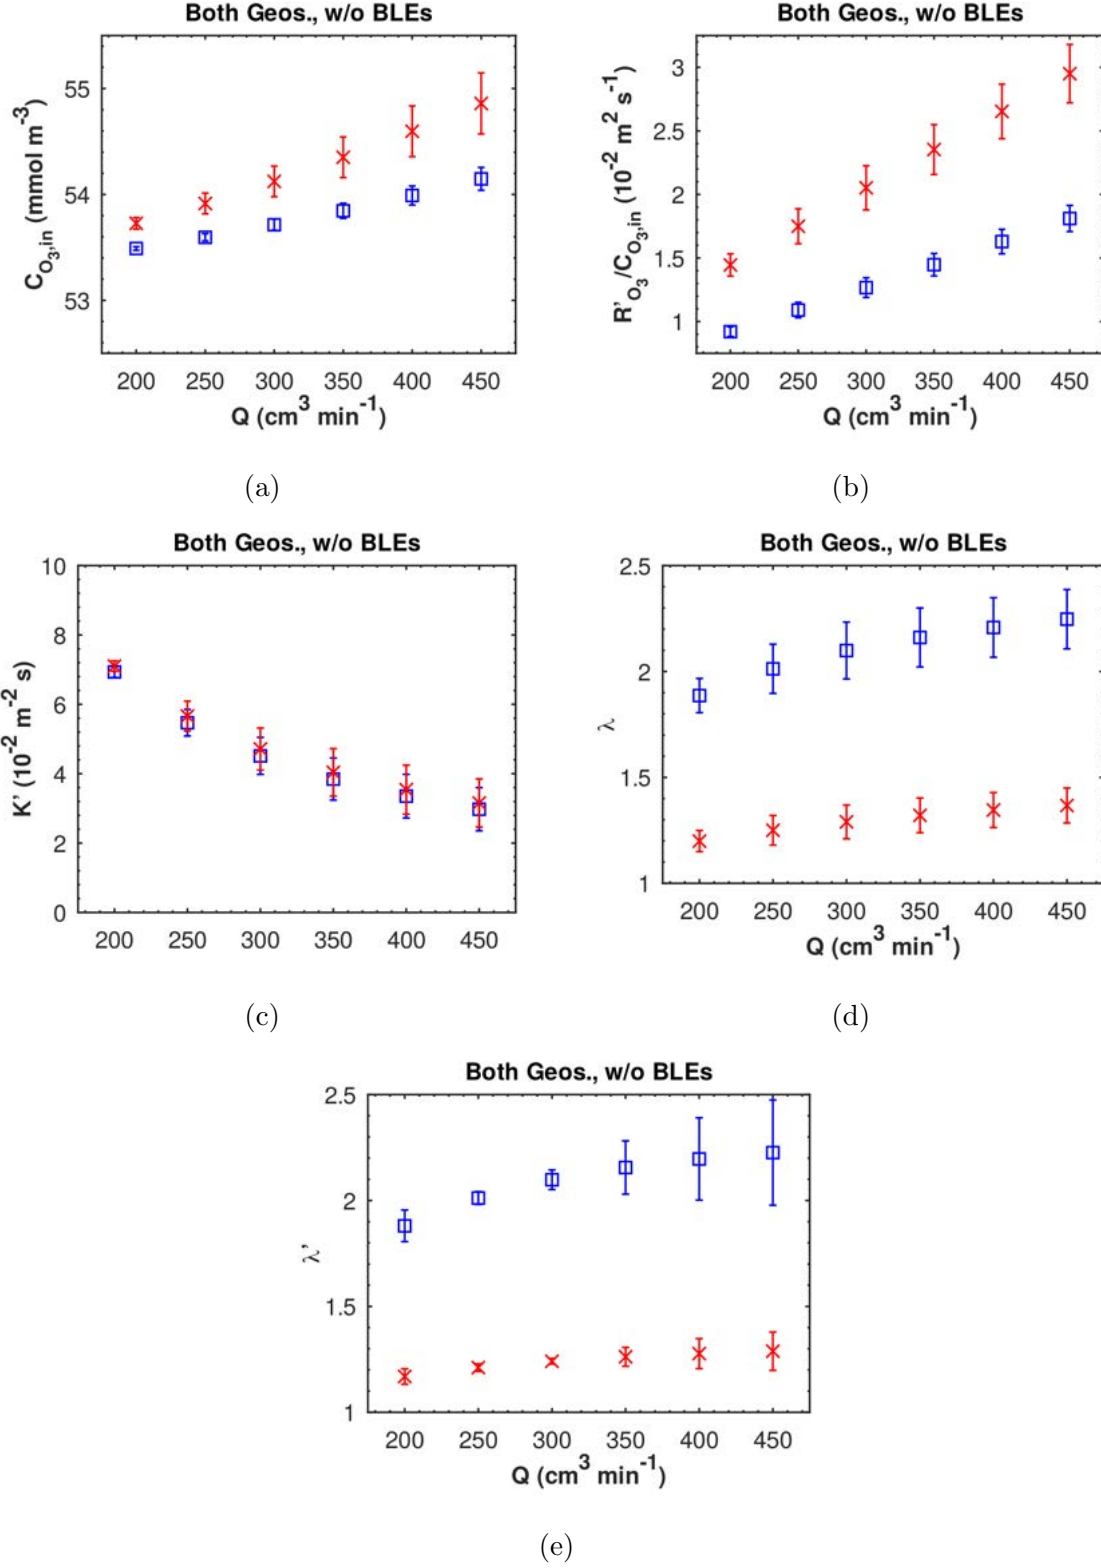

FIG. S19: Auxiliary response variables as function of the inlet flow rate, for both reduced ( $\circ$ ) and full ( $\square$ ) geometries using the no-BLEs mesh variant: (a)  $C_{O_3,in}$ , (b) normalized  $R'_{O_3}$ , (c) normalized  $K'$ , (d) real stoichiometry  $\lambda$ , and (e) apparent stoichiometry  $\lambda'$ .

TABLE S11: Error estimates for the auxiliary response variables for both geometries, using the MOE-12 scheme and no-BLEs mesh variant.

| Variable                                           | Geometry | Relative Error Estimate (%) |         |       |
|----------------------------------------------------|----------|-----------------------------|---------|-------|
|                                                    |          | Minimum                     | Maximum | Mean  |
| $C_{\text{O}_3,\text{in}}$ ( $\text{mol m}^{-3}$ ) | Reduced  | 0.0319                      | 0.200   | 0.116 |
|                                                    | Full     | 0.101                       | 0.527   | 0.312 |
| $R'_{\text{O}_3}$ ( $\text{m}^2 \text{s}^{-1}$ )   | Reduced  | 4.32                        | 6.55    | 5.95  |
|                                                    | Full     | 6.33                        | 9.13    | 8.29  |
| $K'$ ( $\text{m}^{-2} \text{s}$ )                  | Reduced  | 2.24                        | 17.6    | 11.2  |
|                                                    | Full     | 2.08                        | 18.63   | 12.0  |
| $\lambda$                                          | Reduced  | 4.10                        | 6.05    | 5.57  |
|                                                    | Full     | 4.04                        | 5.90    | 5.46  |
| $\lambda'$                                         | Reduced  | 1.47                        | 12.3    | 5.92  |
|                                                    | Full     | 1.07                        | 7.44    | 3.74  |

- 
- [1] P. R. Amestoy, I. S. Duff, J. Koster, and J.-Y. L'Excellent. A fully asynchronous multifrontal solver using distributed dynamic scheduling. *SIAM Journal on Matrix Analysis and Applications*, 23(1):15–41, 2001.
- [2] P. R. Amestoy, A. Guermouche, J.-Y. L'Excellent, and S. Pralet. Hybrid scheduling for the parallel solution of linear systems. *Parallel Computing*, 32(2):136–156, 2006.
- [3] Y. Saad and M. H. Schultz. GMRES: A generalized minimal residual algorithm for solving nonsymmetric linear systems. *SIAM Journal on Scientific and Statistical Computing*, 7:856–869, 1986.
- [4] S. P. Vanka. Block-implicit multigrid solution of Navier-Stokes equations in primitive variables. *J. Comput. Phys.*, 65:138–158, 1986.
- [5] O. Schenk and K. Gärtner. *Parallel Sparse Direct Solver PARDISO - User Guide*, versão 5.0.0 edition, 2014.
- [6] A. Toselli and O. B. Widlund. *Domain Decomposition Methods*. Springer, Berlin, Heidelberg, 1 edition, 2005.
- [7] P. J. Roache. Quantification of uncertainty in computational fluid dynamics. *Annu. Rev. Fluid. Mech.*, 29:123–160, 1997.
- [8] C. J Roy. Grid convergence error analysis for mixed-order numerical schemes. *AIAA J.*, 41:595–604, 2003.
